# Supplementary material for: Vertical Federated Learning without Revealing Intersection Membership
Source: arXiv:2106.05508 source file (2021-06-10)
Supplement: Supplementary file 1 [file additional_experiments.tex]

\section{Additional Experiments}
\subsection{Criteo}

\begin{figure*}[t]
  \begin{minipage}[b]{0.33\linewidth}
  \centering
    \includegraphics[width=\linewidth]{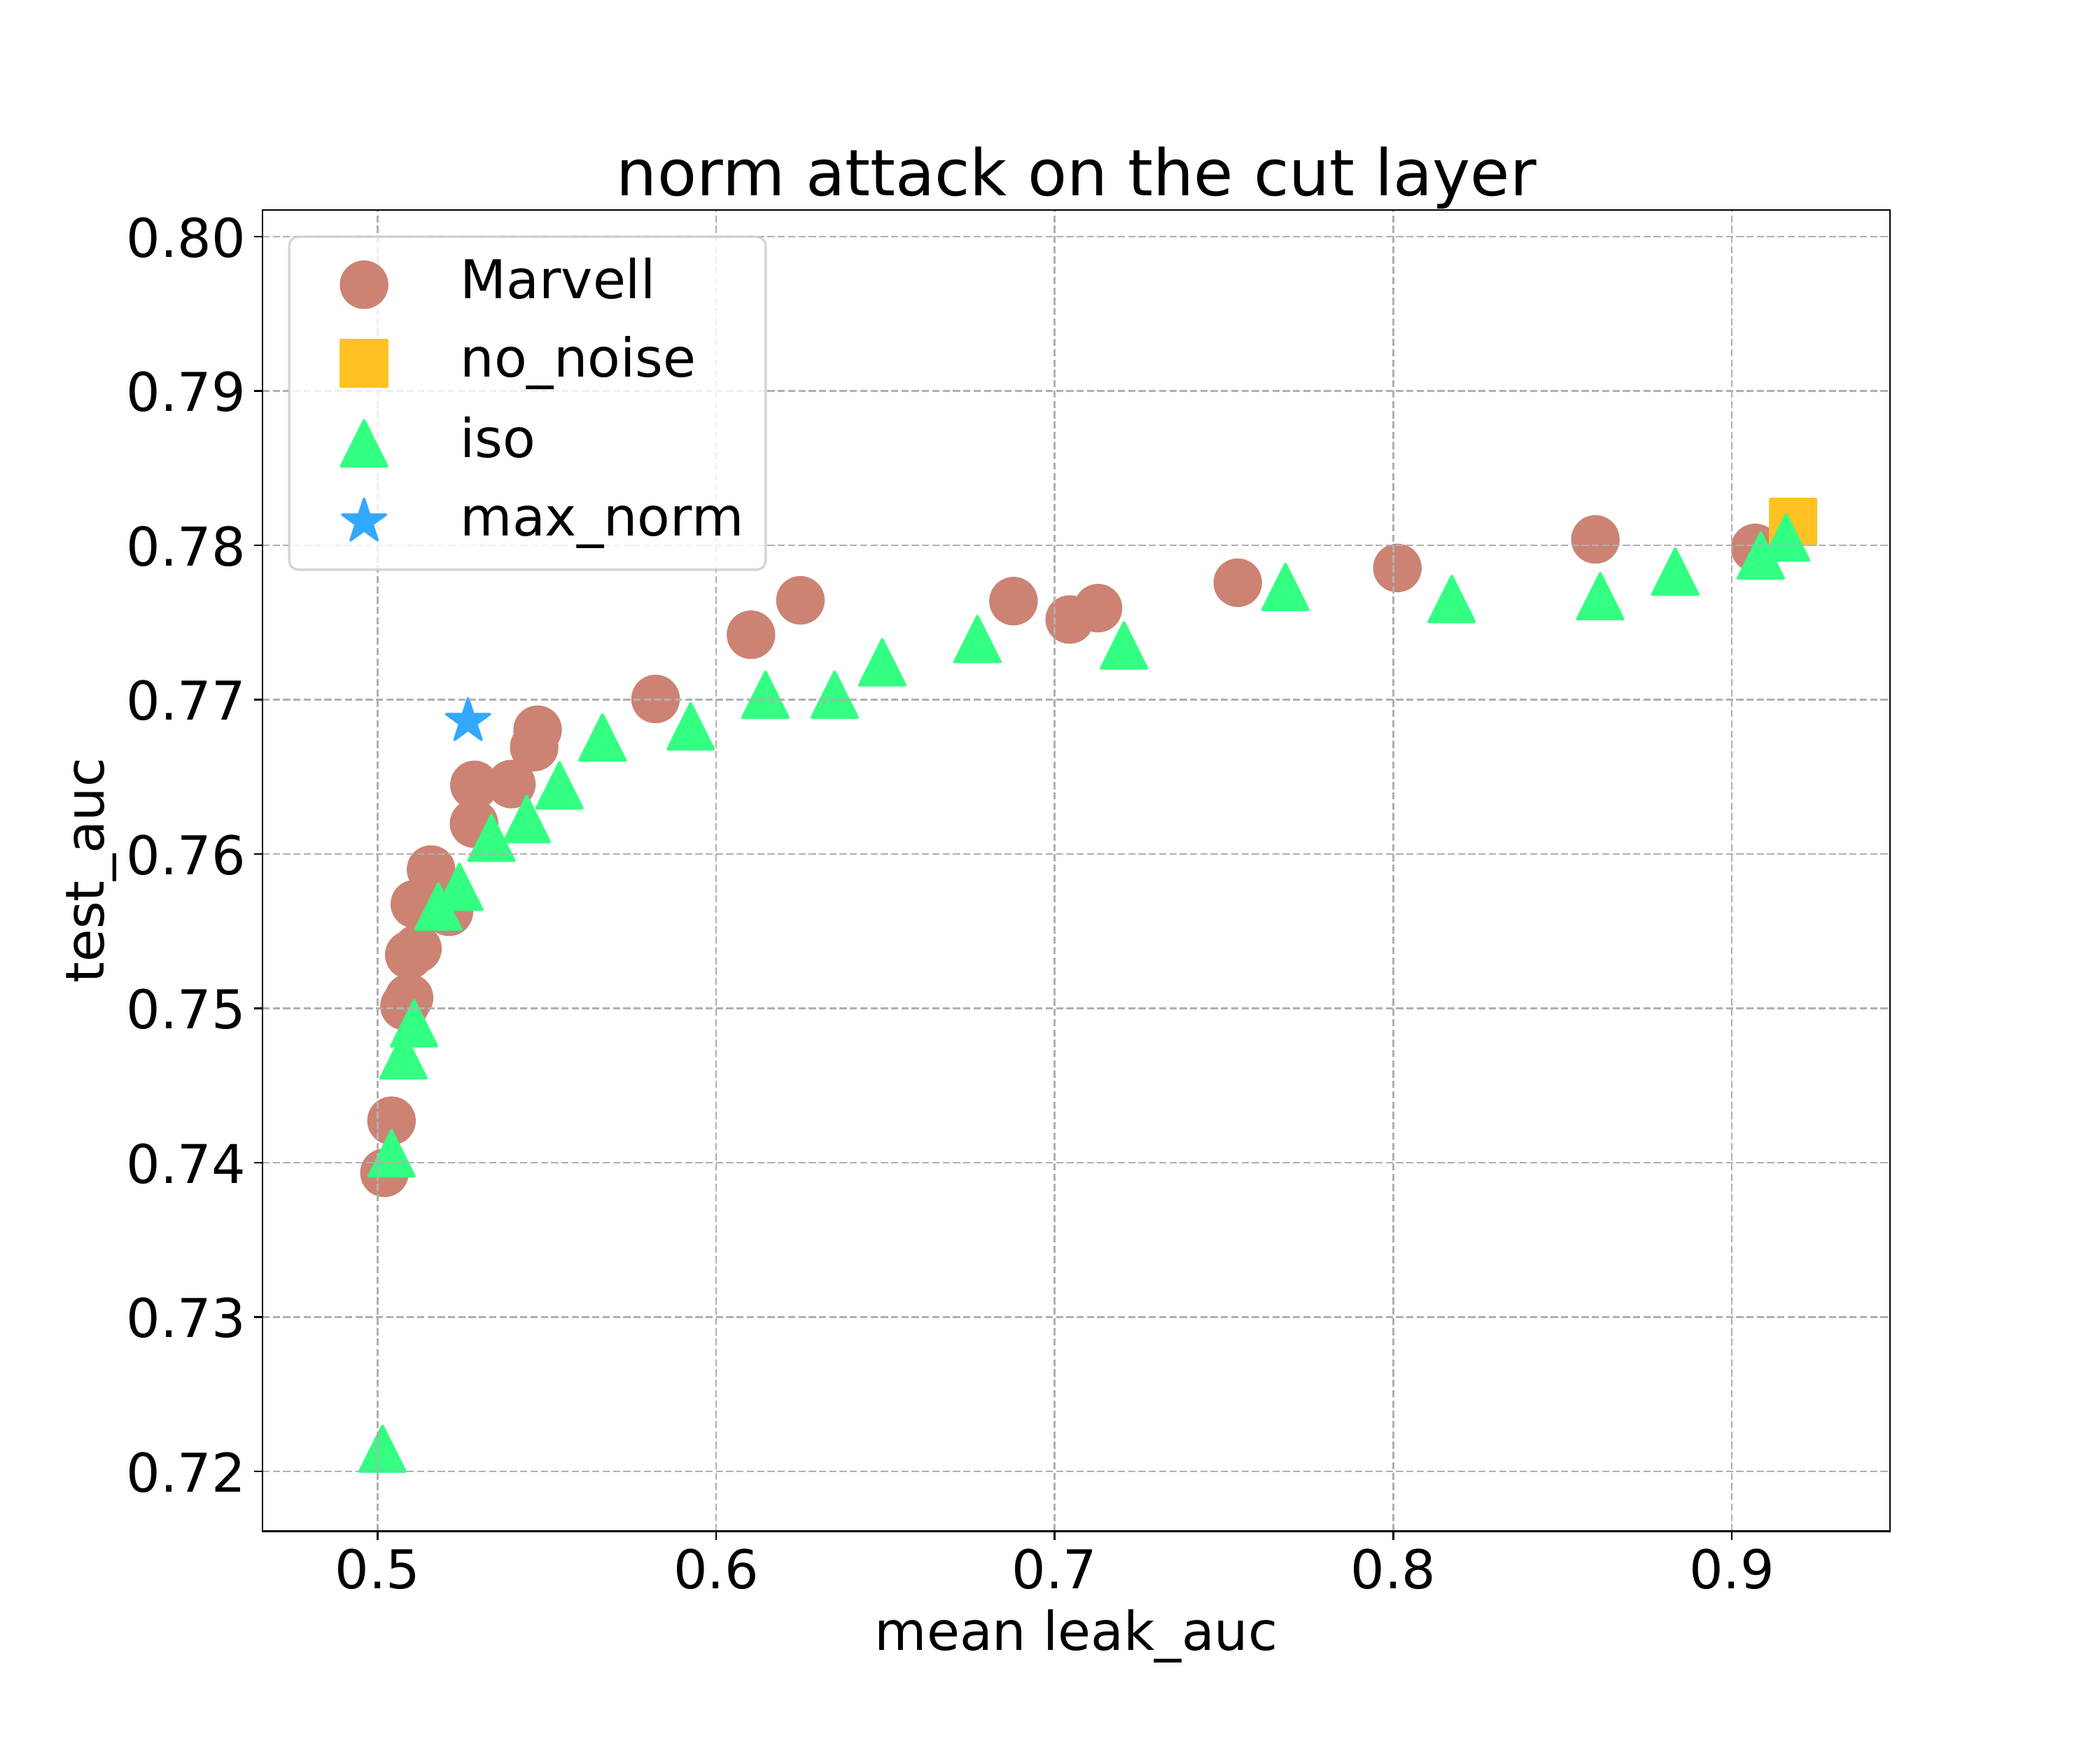}
      \caption*{ (a: )}
  \end{minipage}
  \begin{minipage}[b]{0.33\linewidth}
  \centering
    \includegraphics[width=\linewidth]{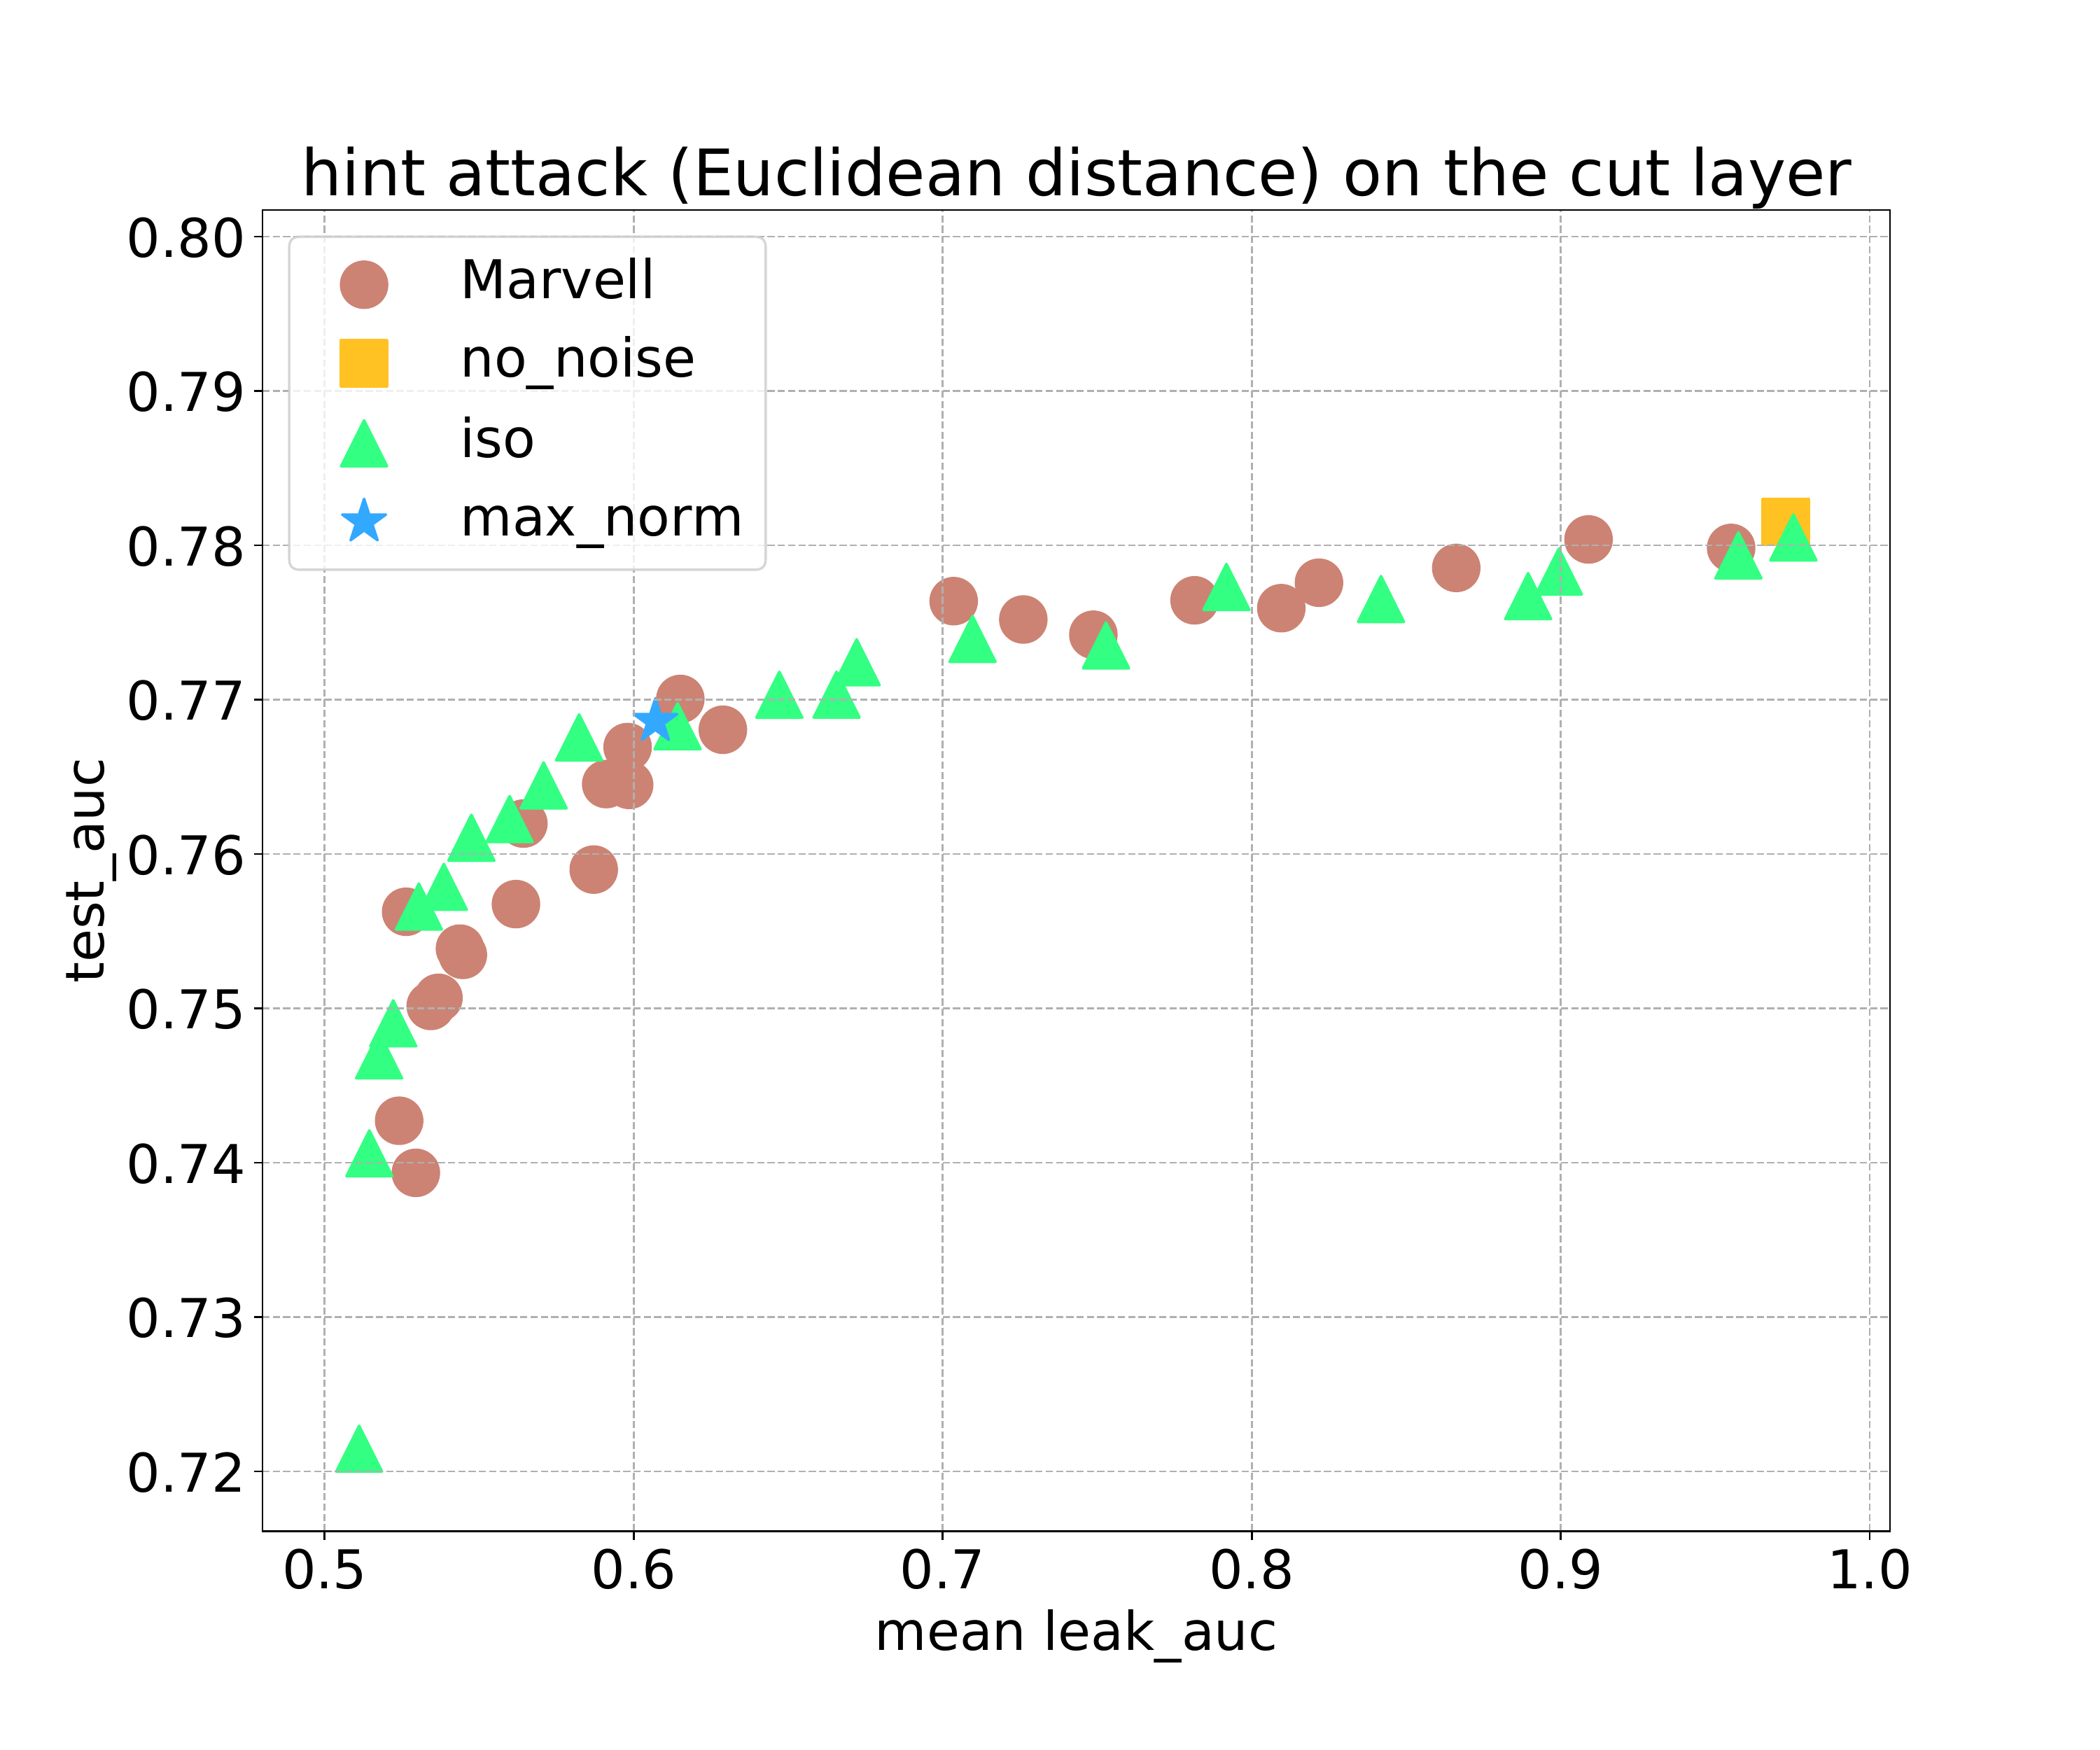}
    \caption*{(b: )}
  \end{minipage}
   \begin{minipage}[b]{0.33\linewidth}
  \centering
    \includegraphics[width=\linewidth]{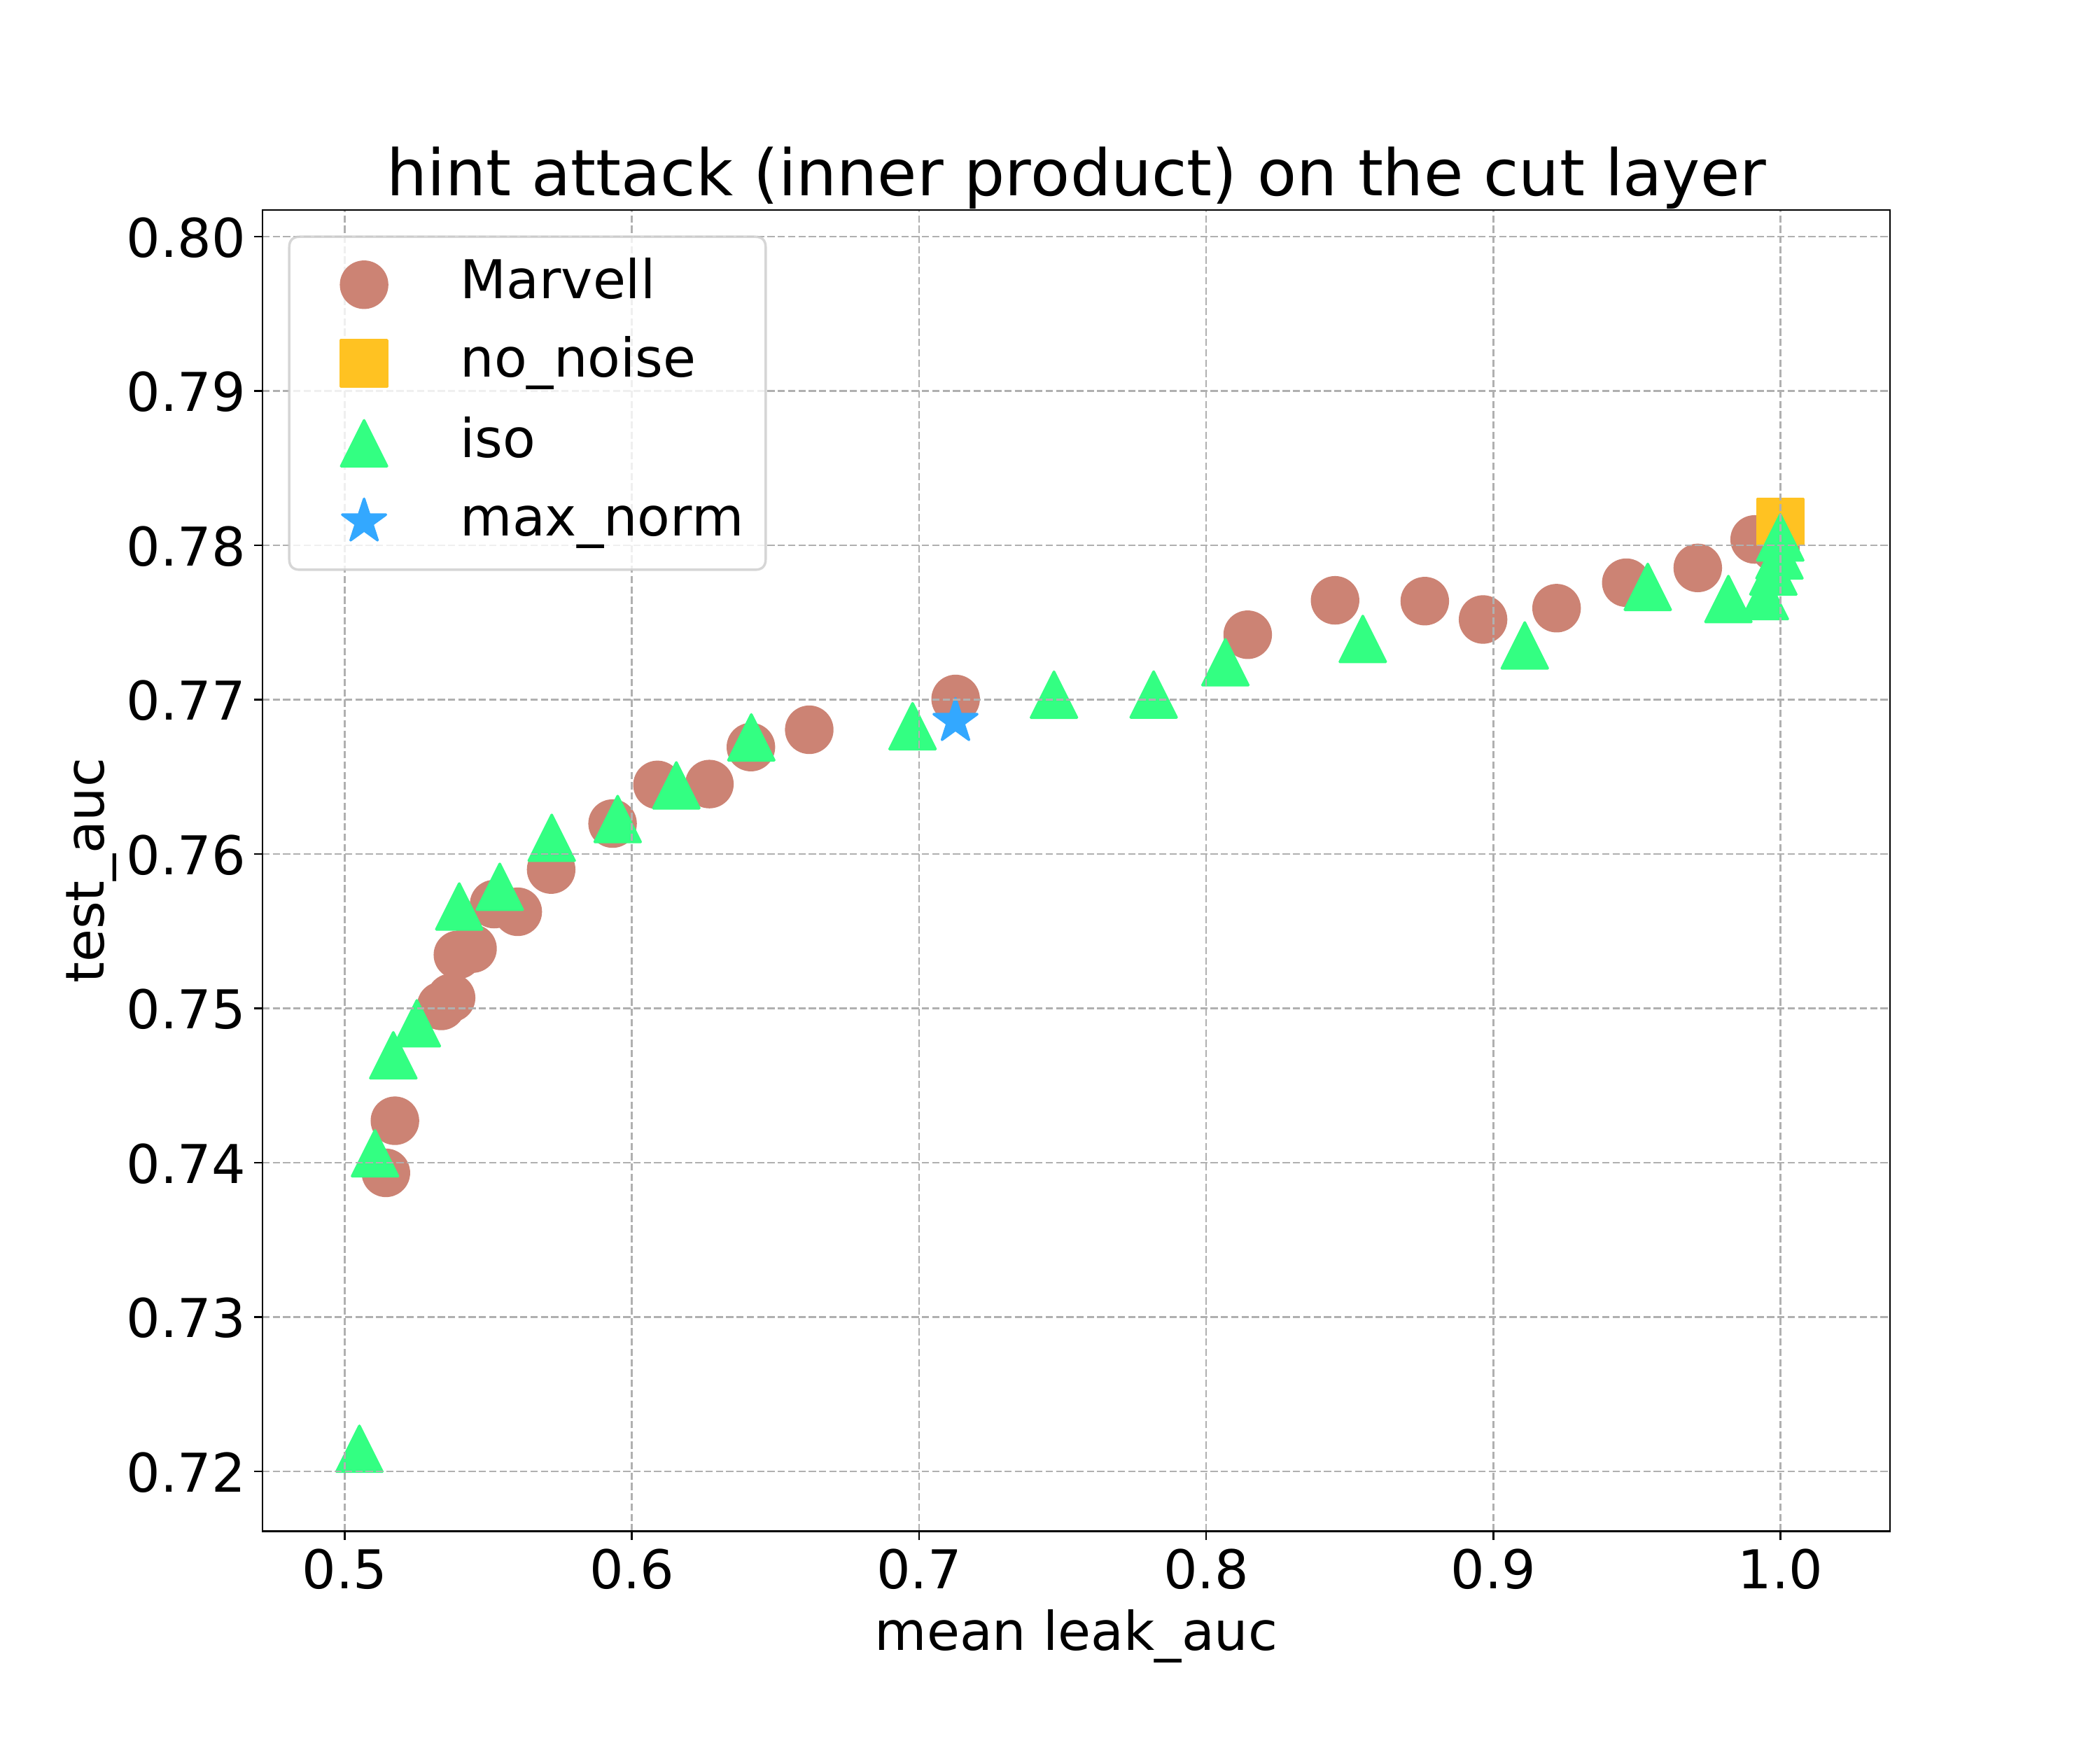}
      \caption*{ (c: )}
  \end{minipage}
 \vspace{-1.5em}
 \caption{Criteo: trade-off between test AUC and leak AUC. num hints = $5$.}
 \label{fig:criteo_tradeoff_test_auc_privacy} 
\end{figure*}

\begin{figure*}[t]
  \begin{minipage}[b]{0.33\linewidth}
  \centering
    \includegraphics[width=\linewidth]{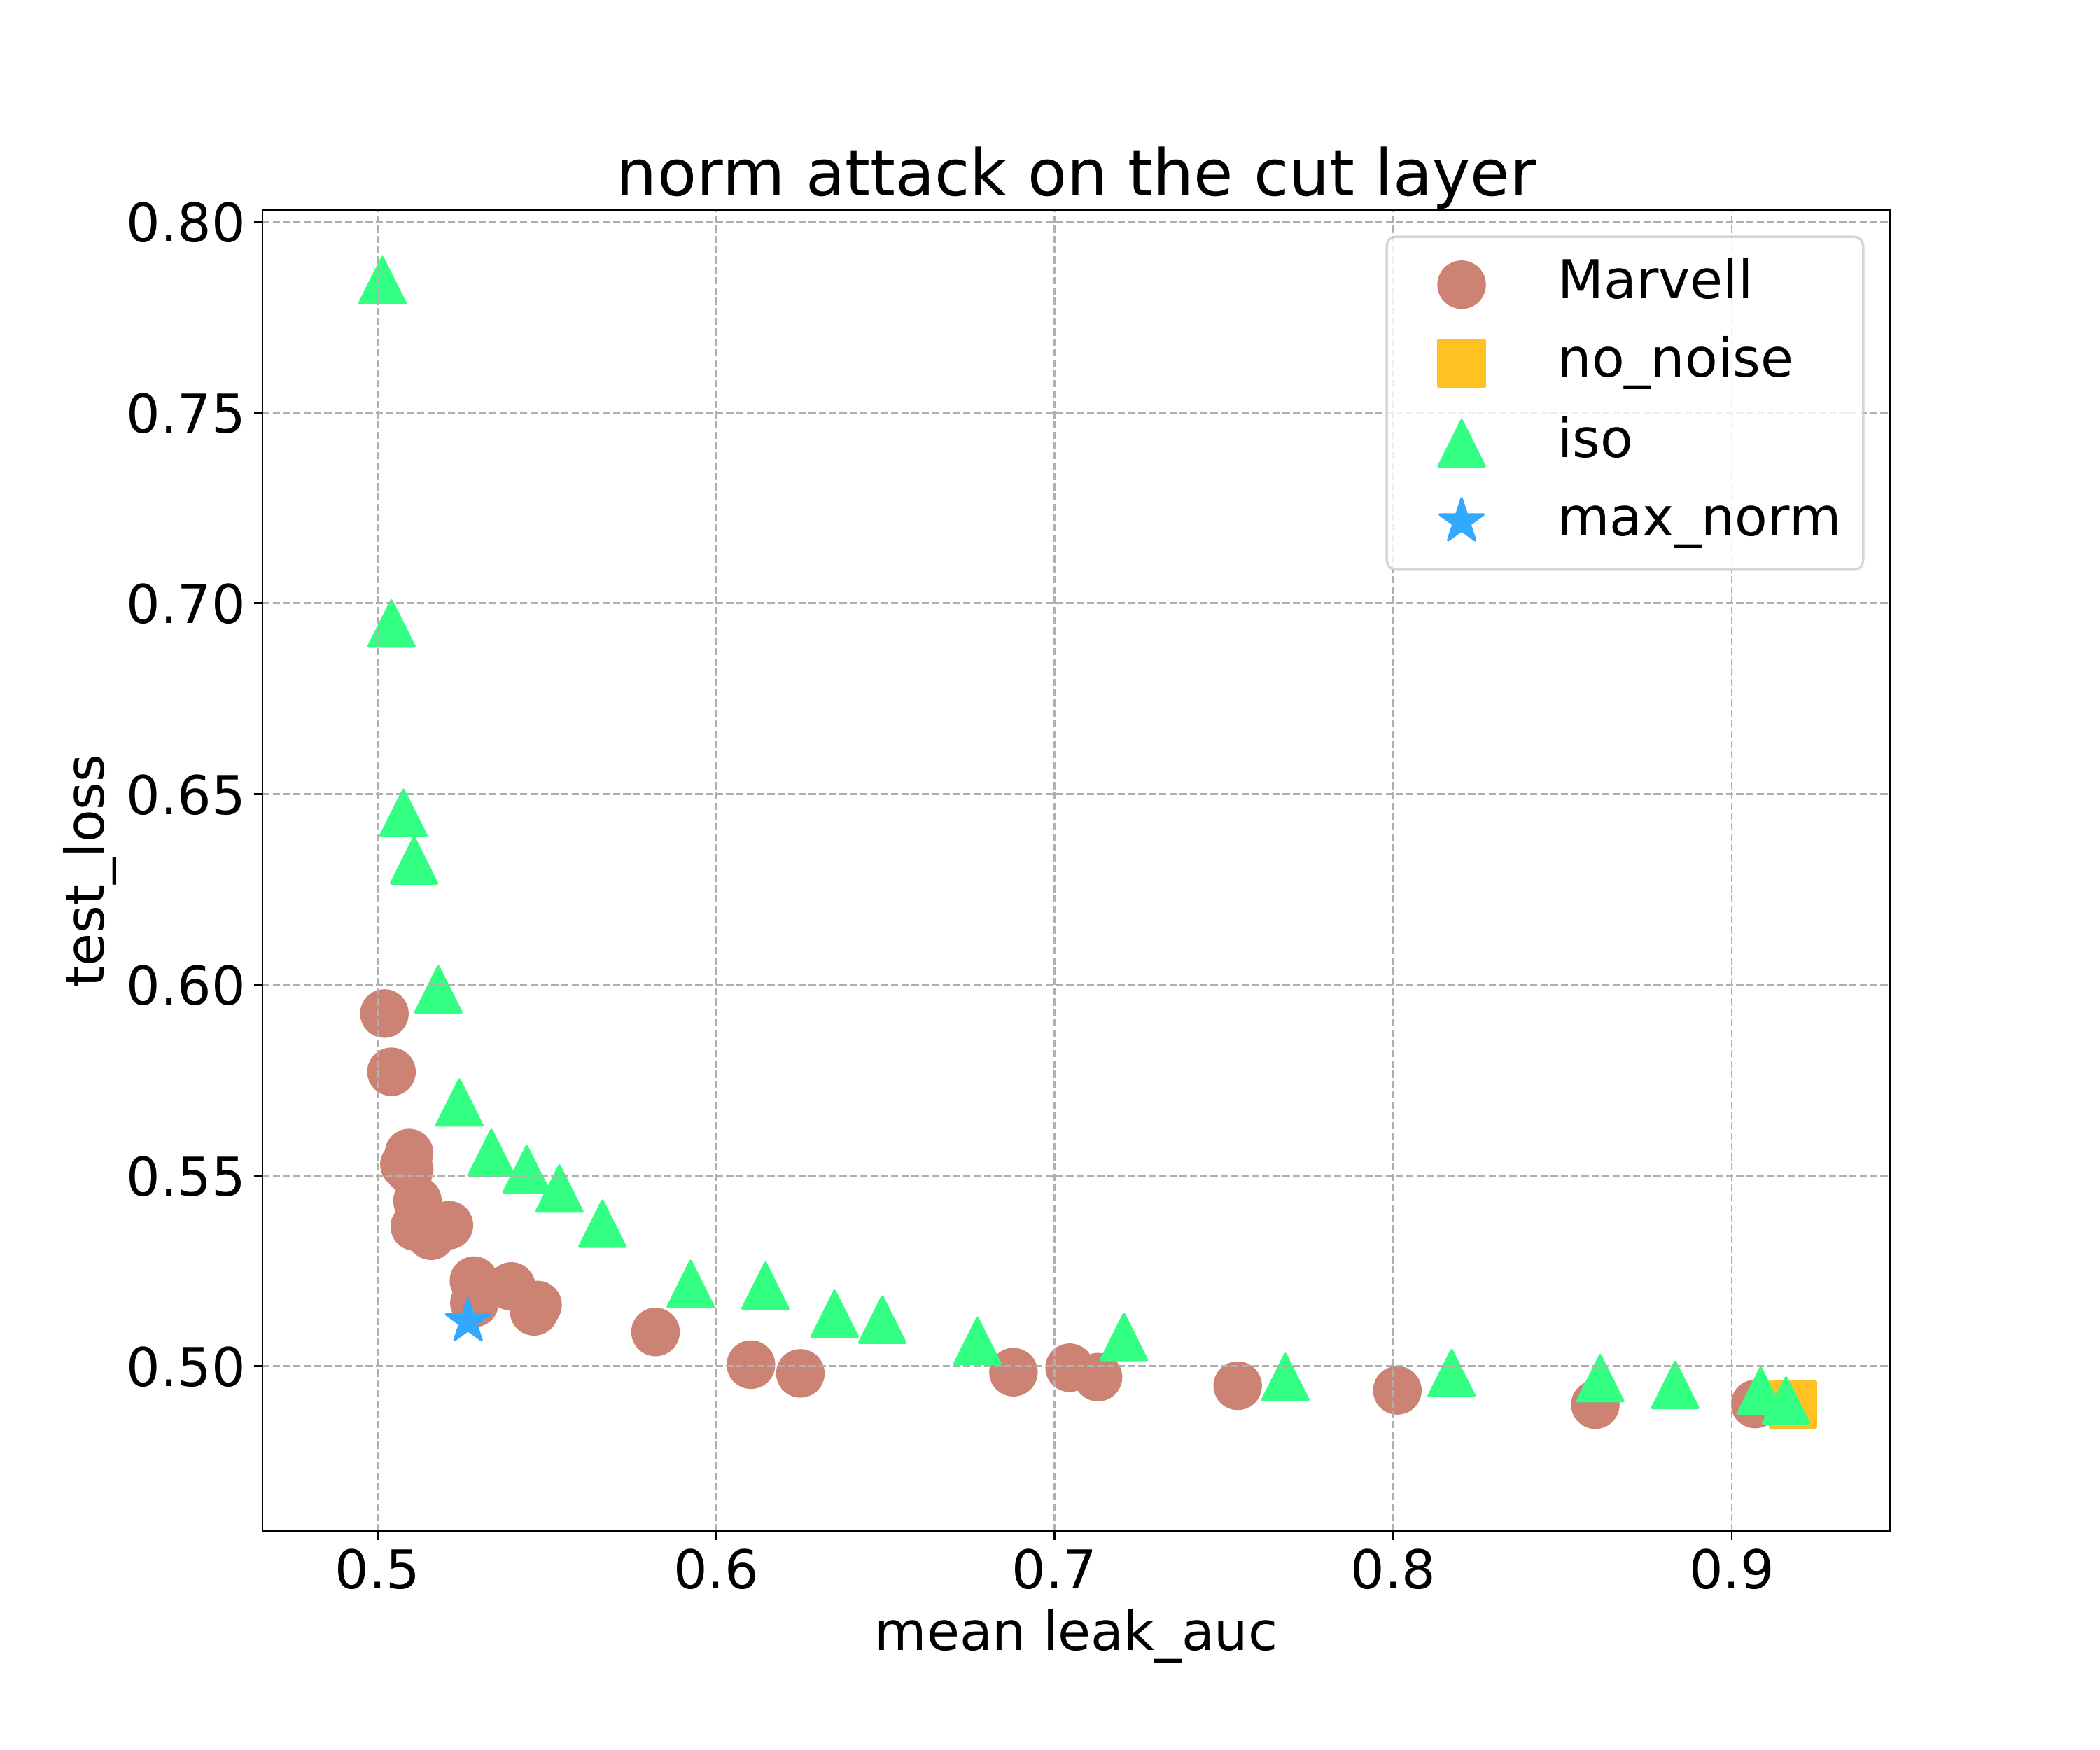}
      \caption*{ (a: )}
  \end{minipage}
  \begin{minipage}[b]{0.33\linewidth}
  \centering
    \includegraphics[width=\linewidth]{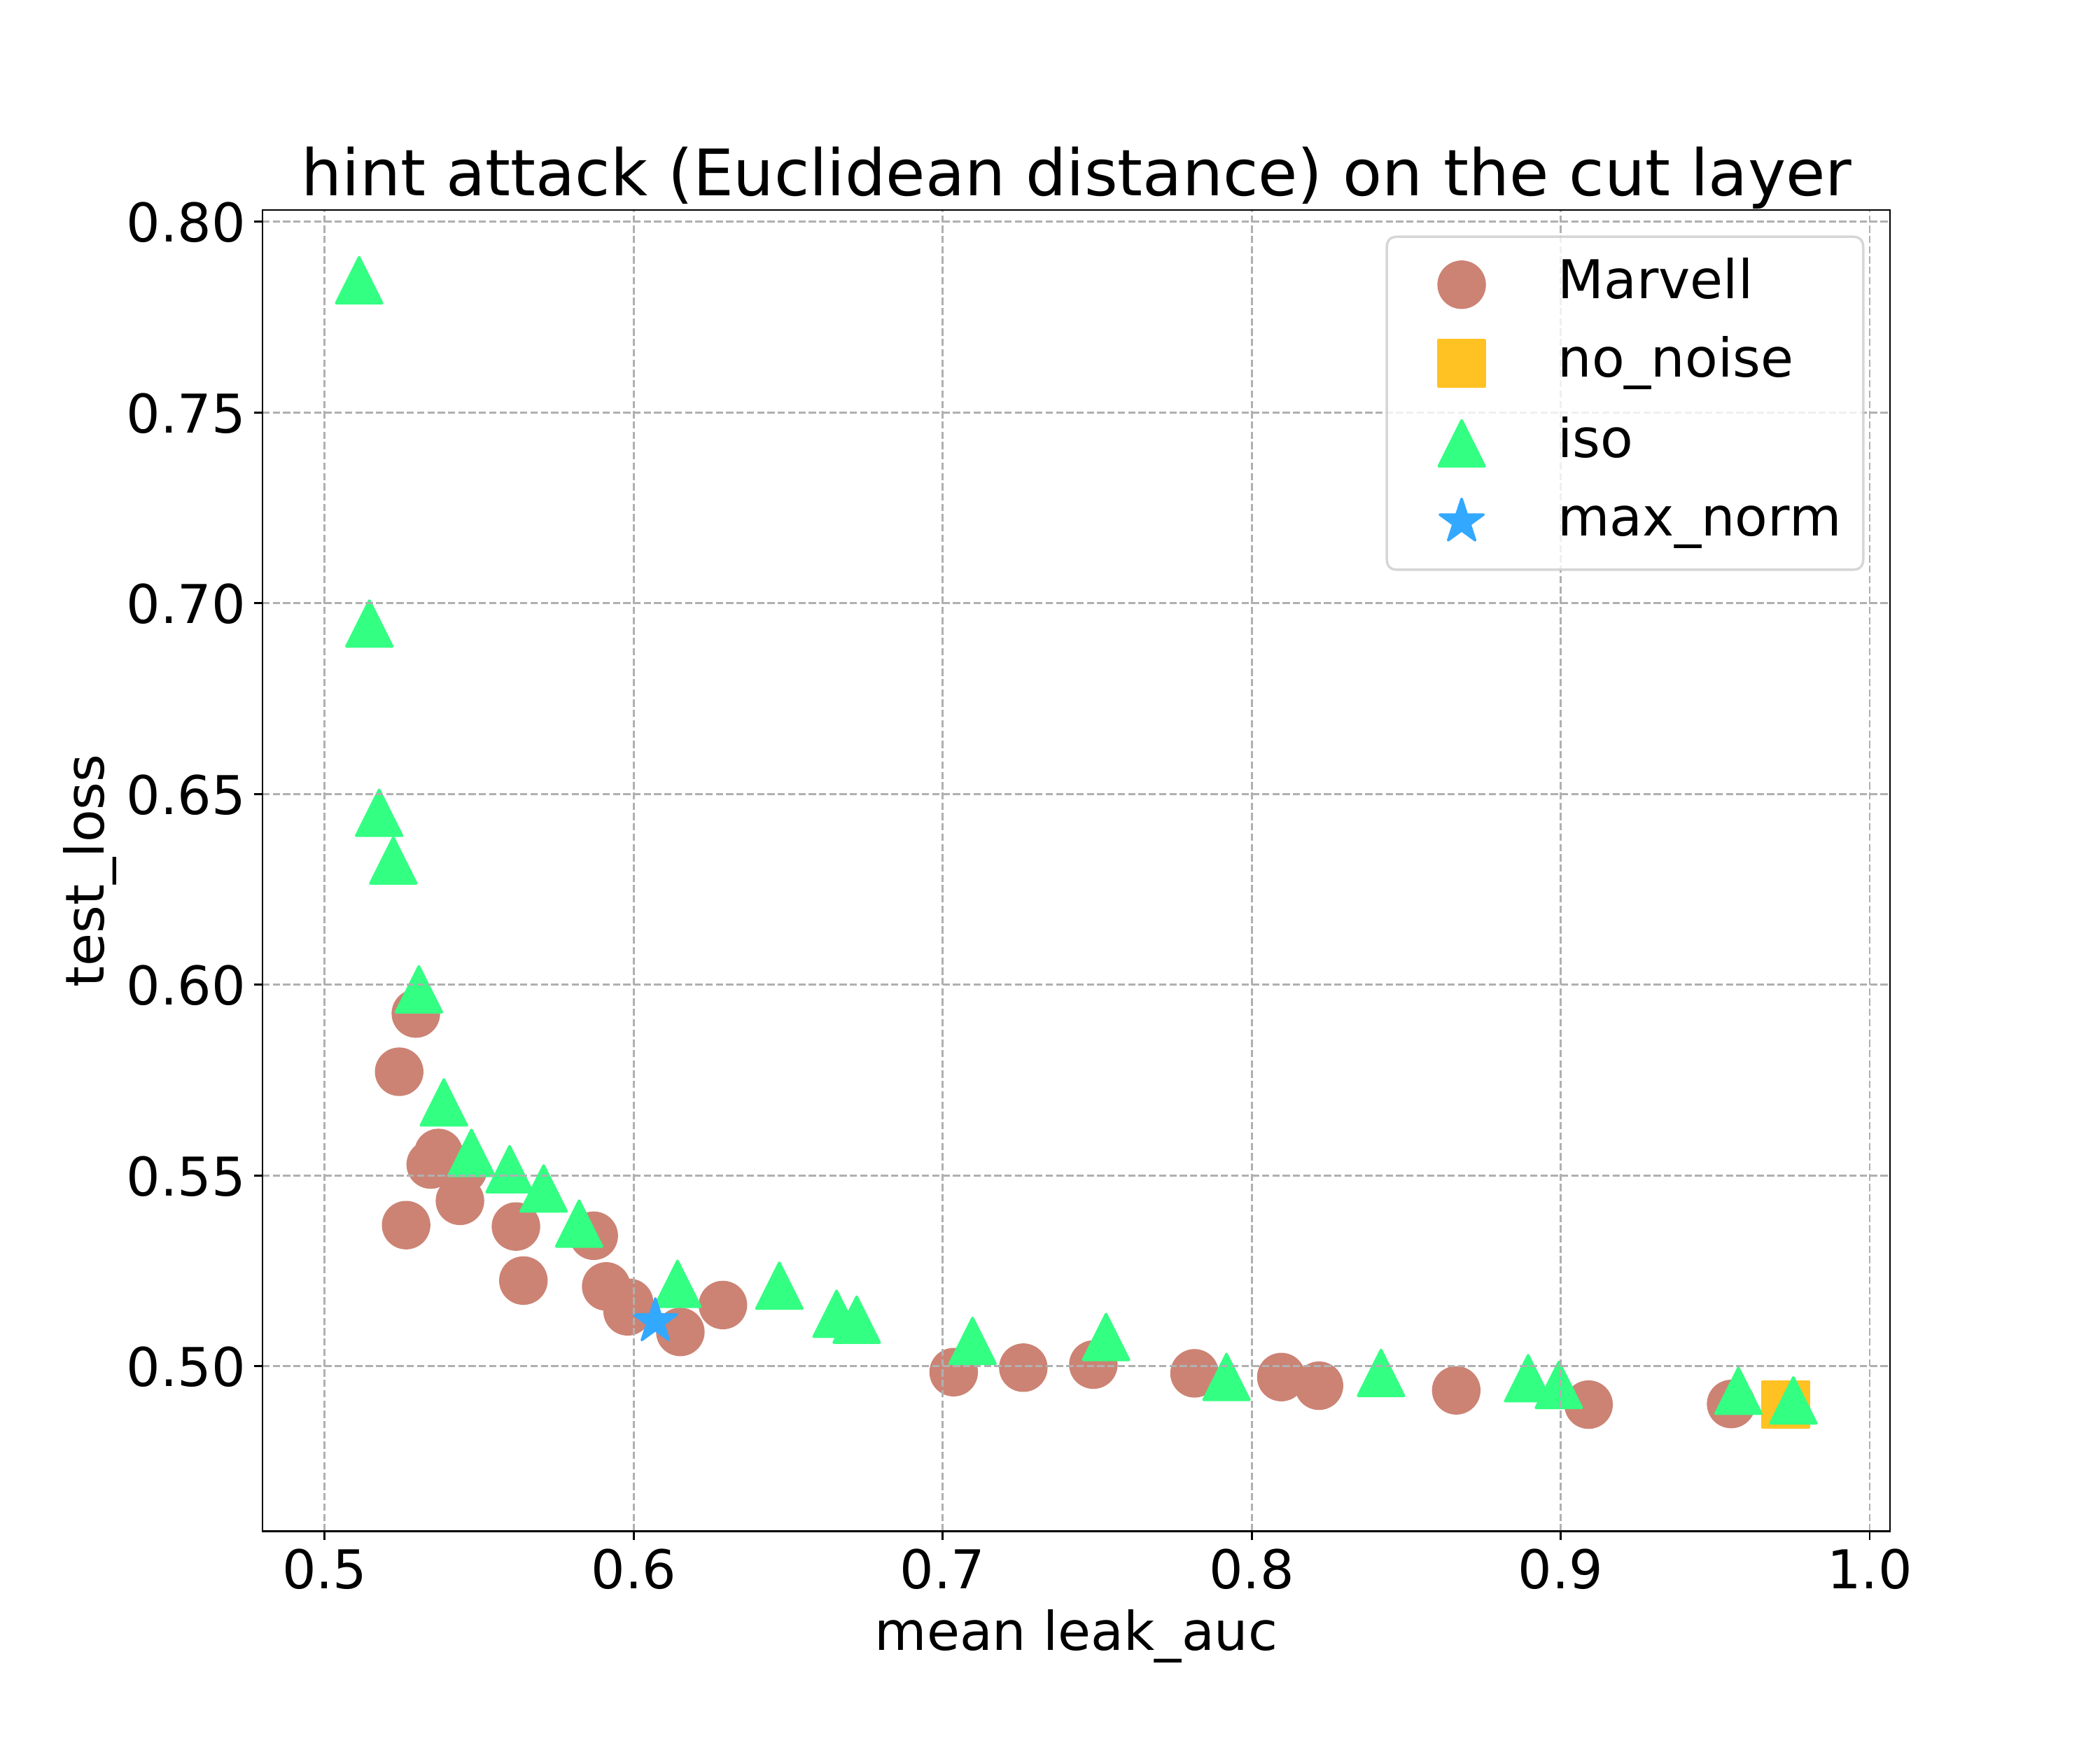}
    \caption*{(b: )}
  \end{minipage}
   \begin{minipage}[b]{0.33\linewidth}
  \centering
    \includegraphics[width=\linewidth]{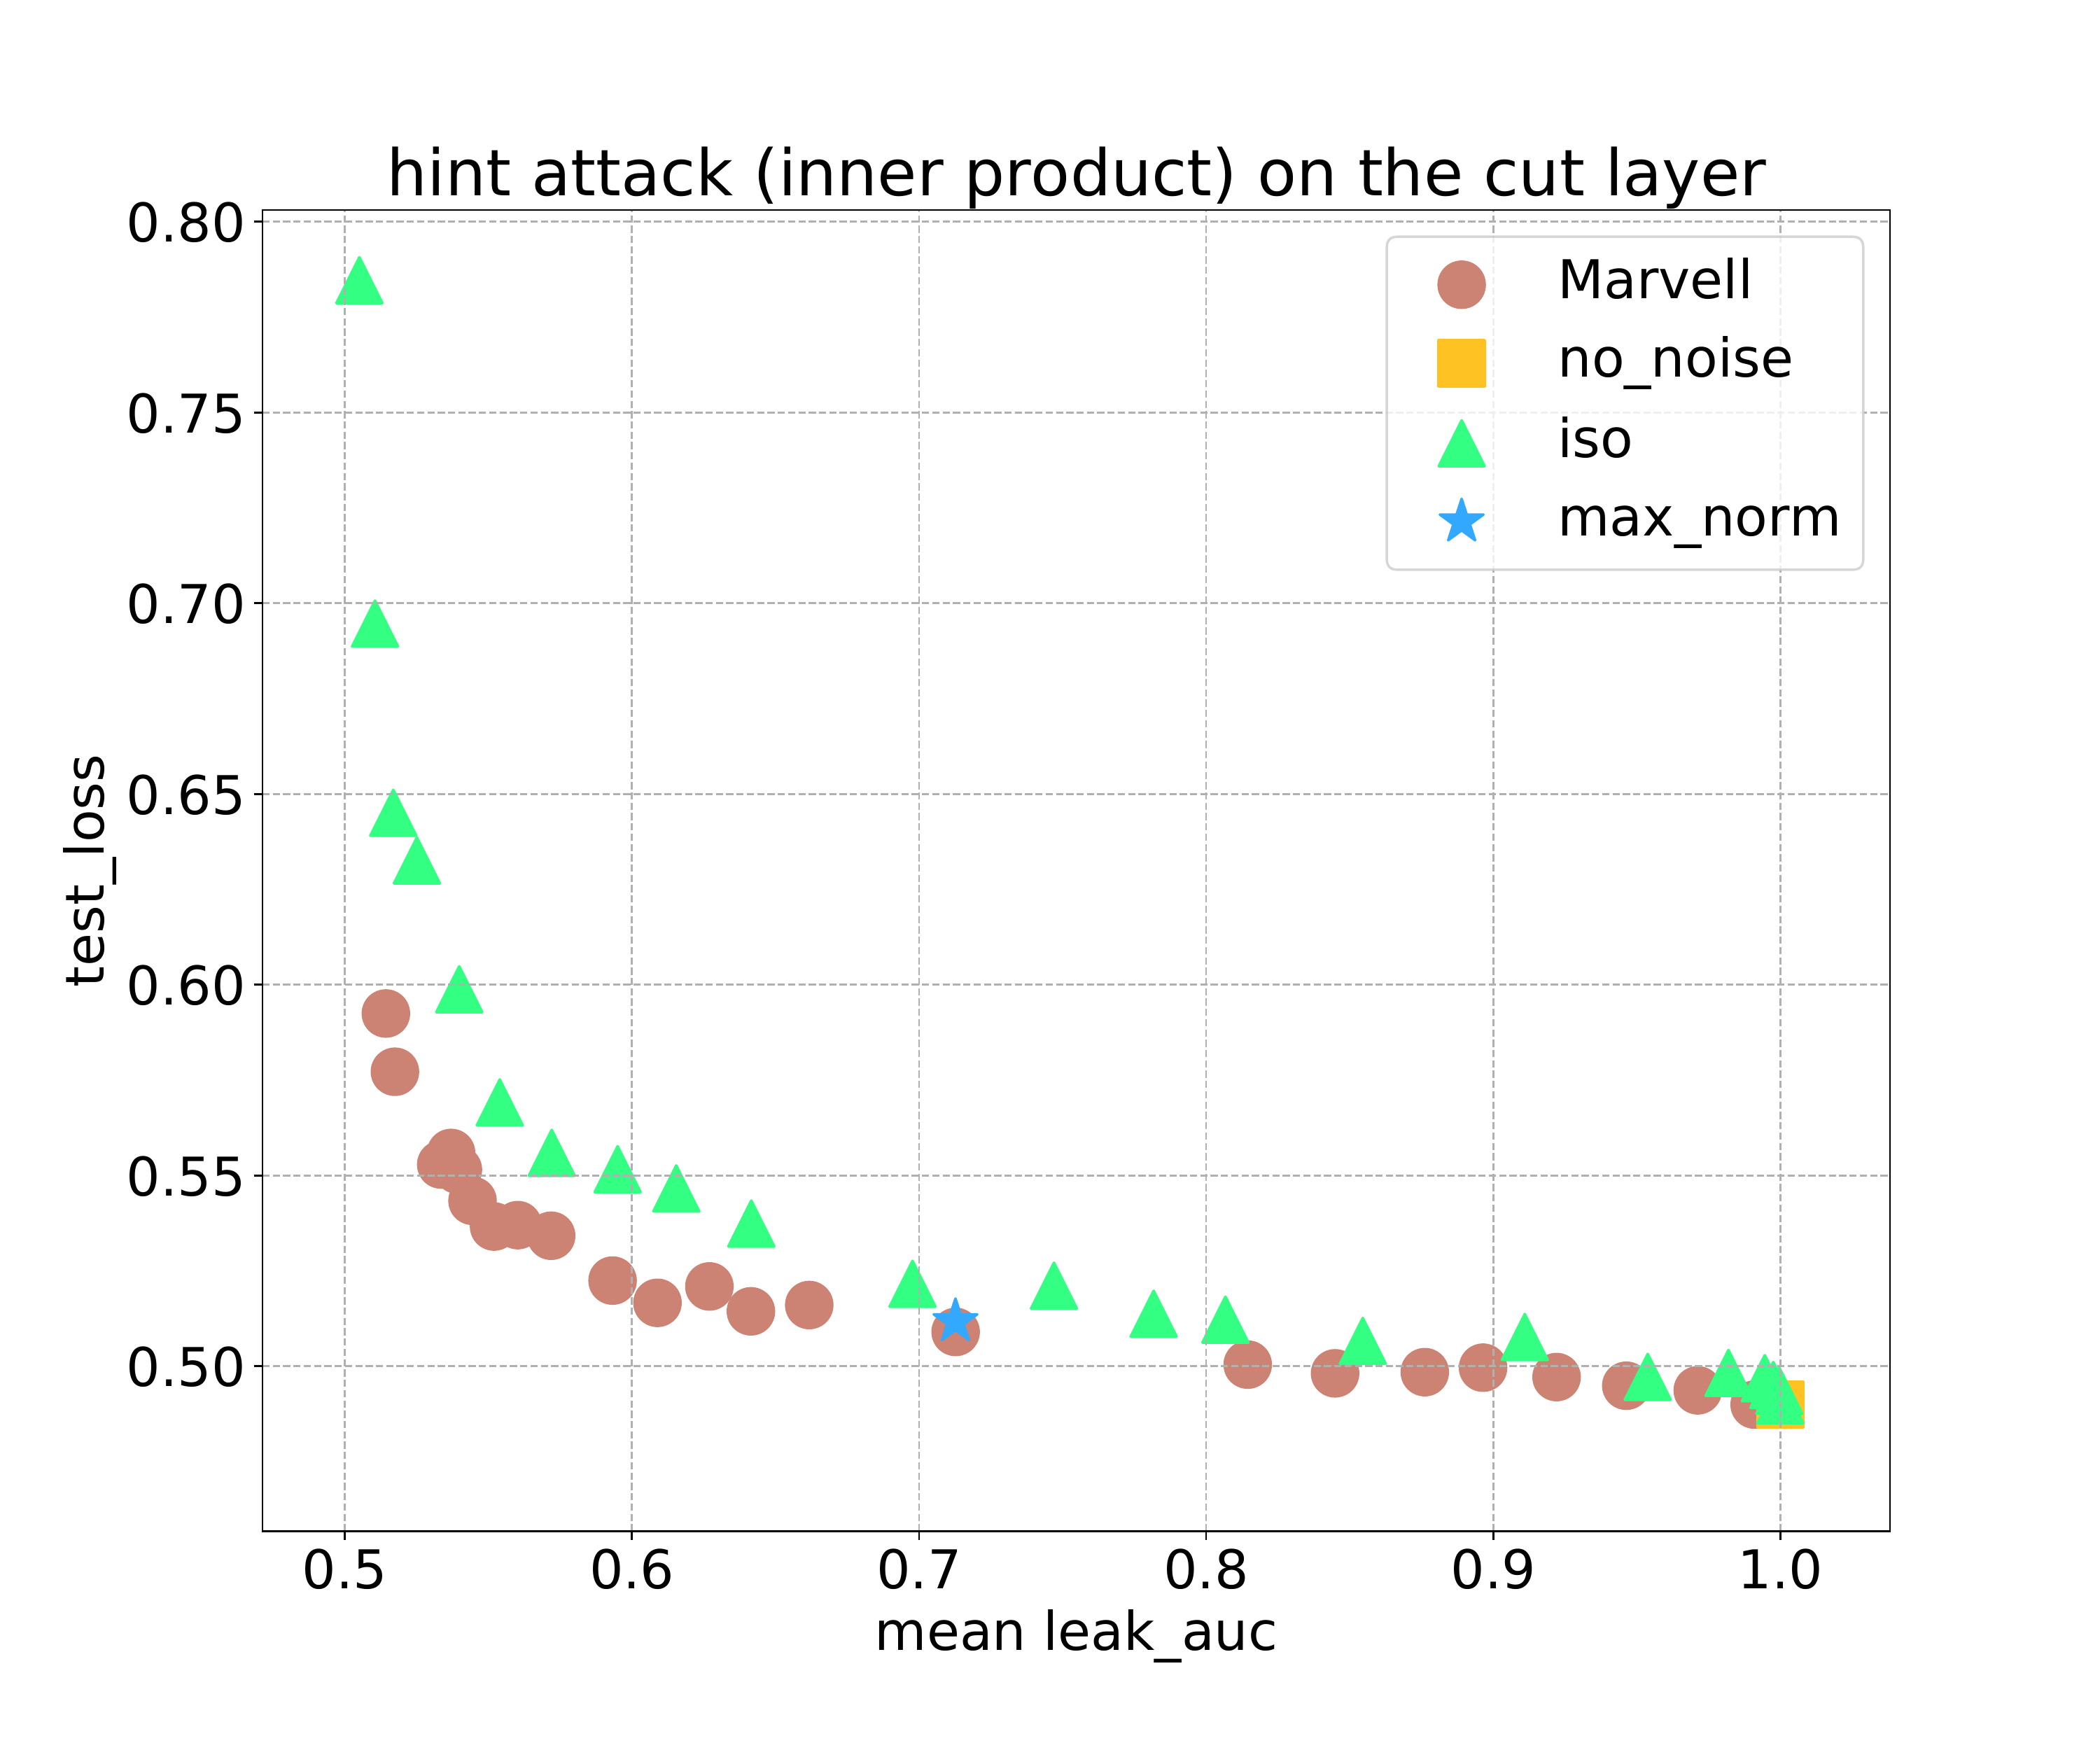}
      \caption*{ (c: )}
  \end{minipage}
 \vspace{-1.5em}
 \caption{Criteo: trade-off between test loss and leak AUC. num hints = $5$.}
 \label{fig:criteo_tradeoff_test_loss_privacy} 
\end{figure*}


\begin{figure*}[ht!]
  \begin{minipage}[b]{0.495\linewidth}
  \centering
    \includegraphics[width=\linewidth]{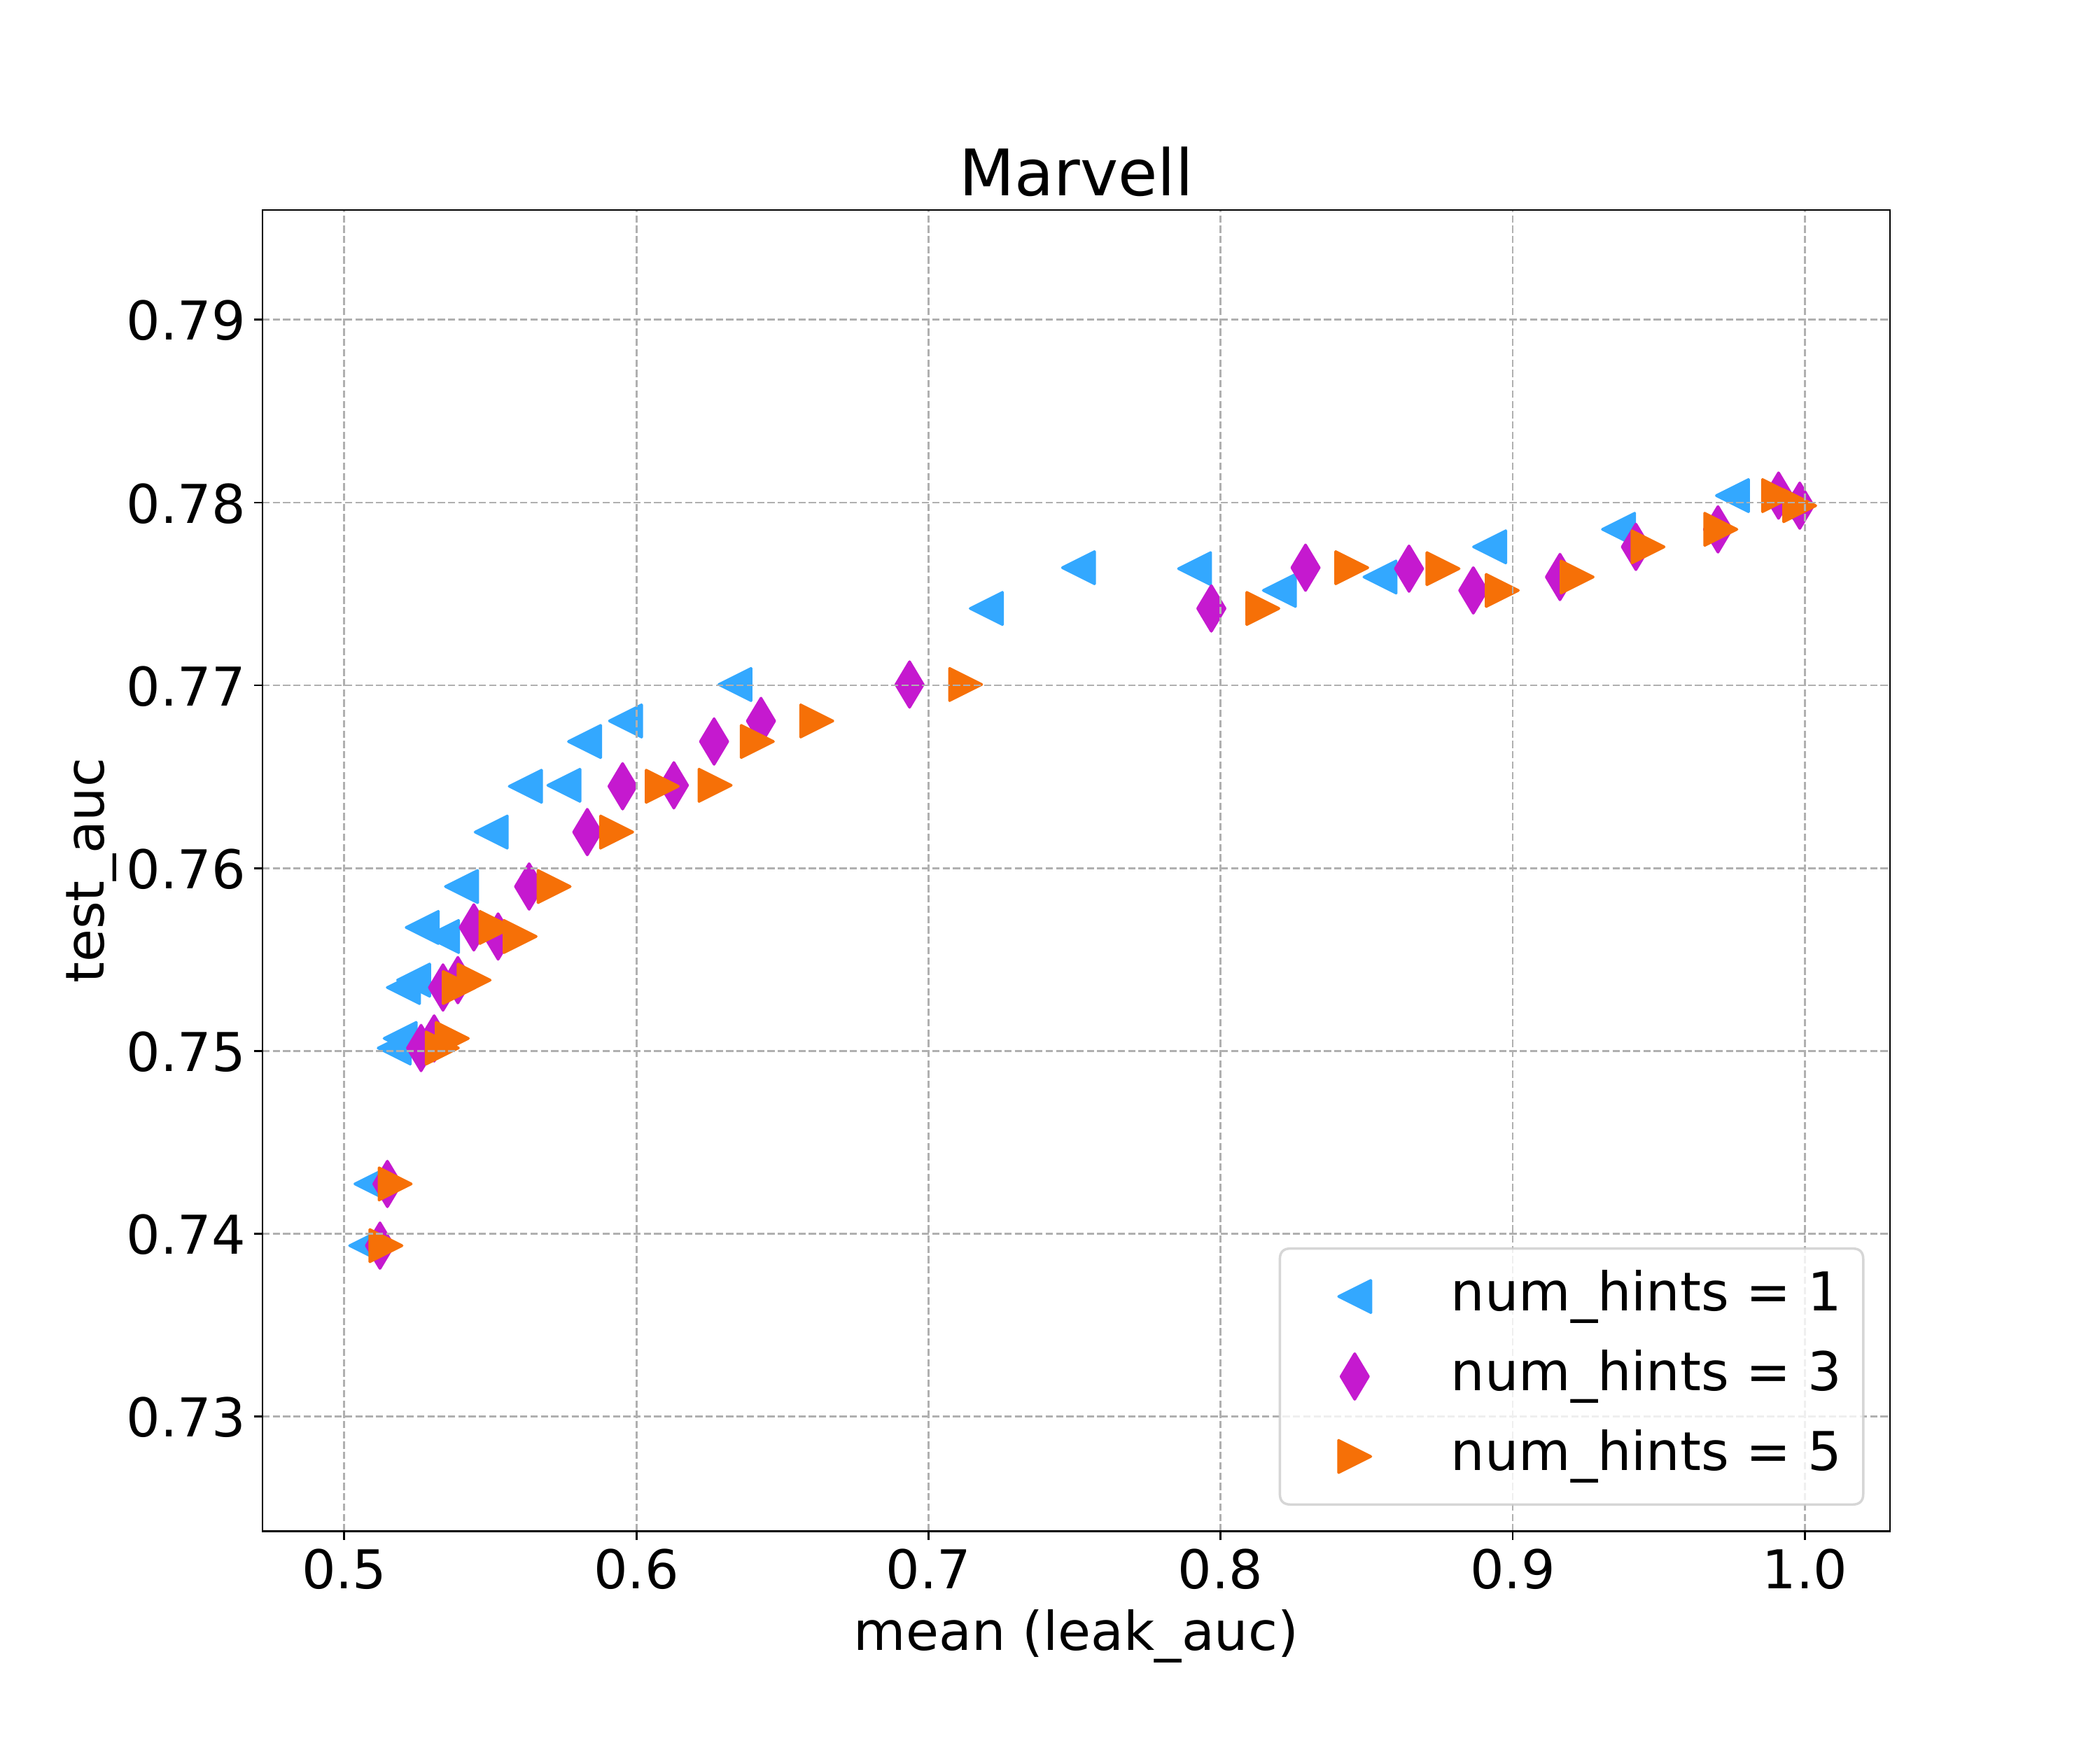}
      \caption*{ (a: )}
  \end{minipage}
  \begin{minipage}[b]{0.495\linewidth}
  \centering
    \includegraphics[width=\linewidth]{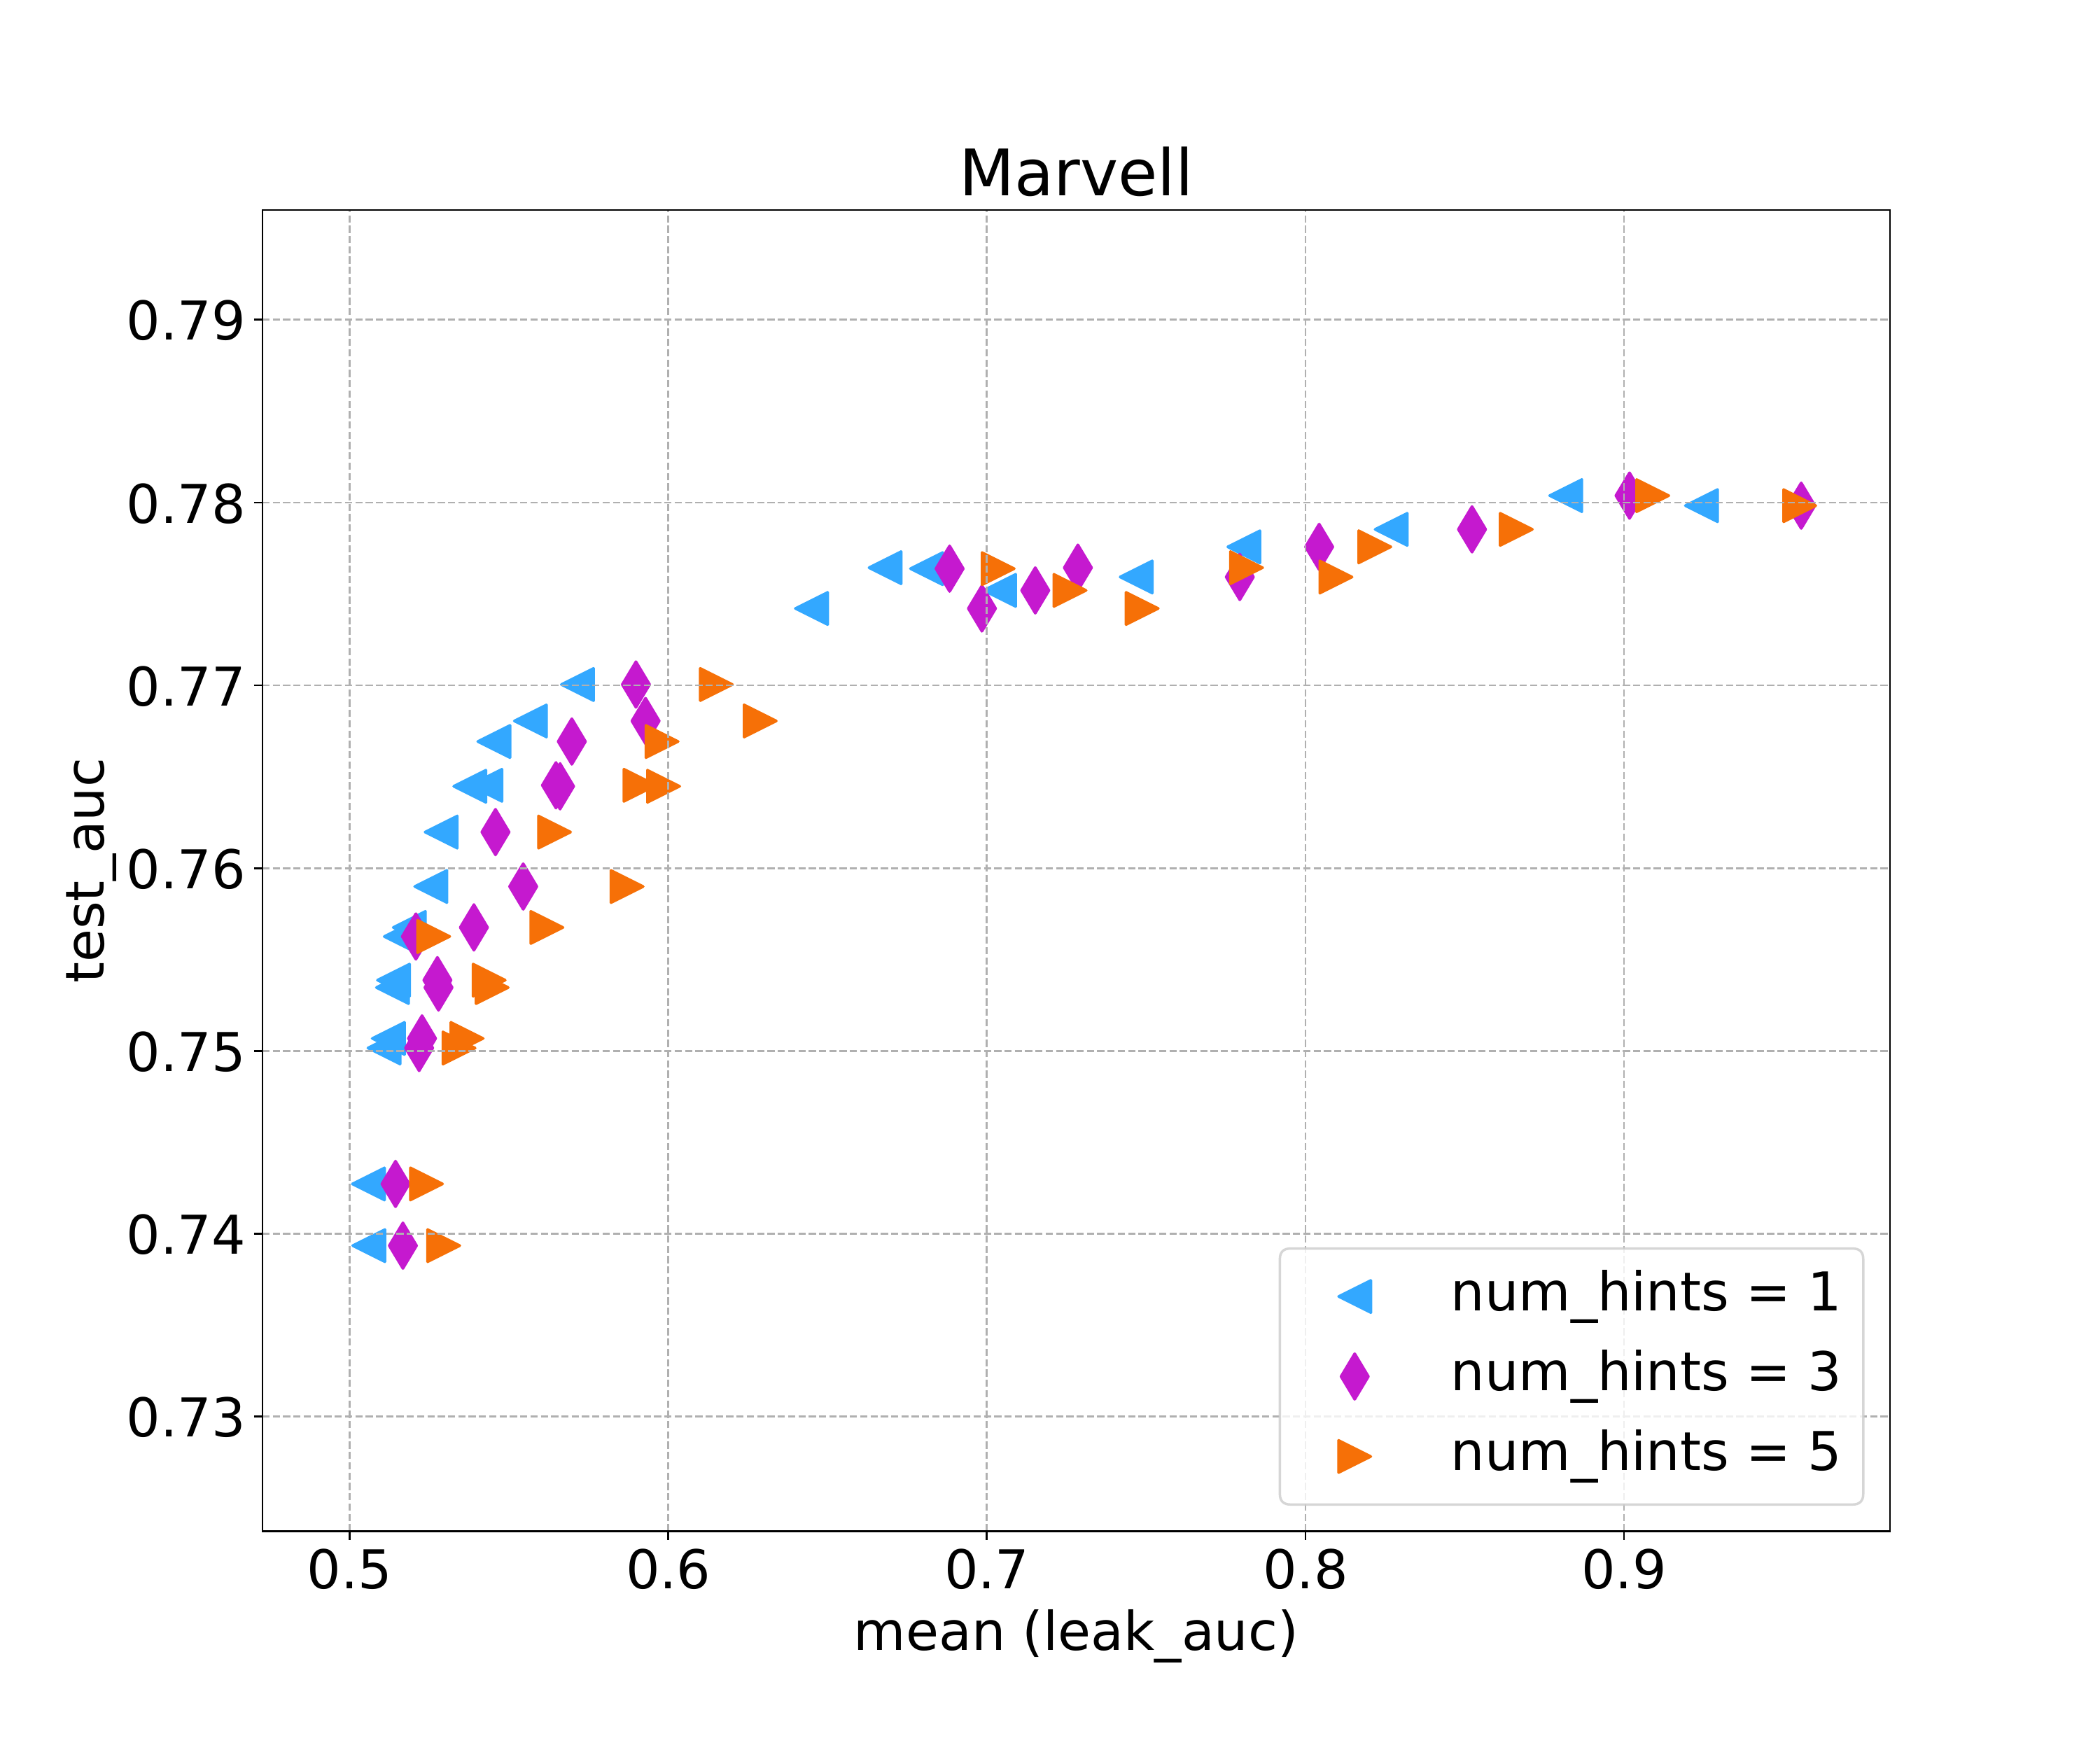}
    \caption*{(b: )}
  \end{minipage}
  \medskip
  \begin{minipage}[b]{0.495\linewidth}
  \centering
    \includegraphics[width=\linewidth]{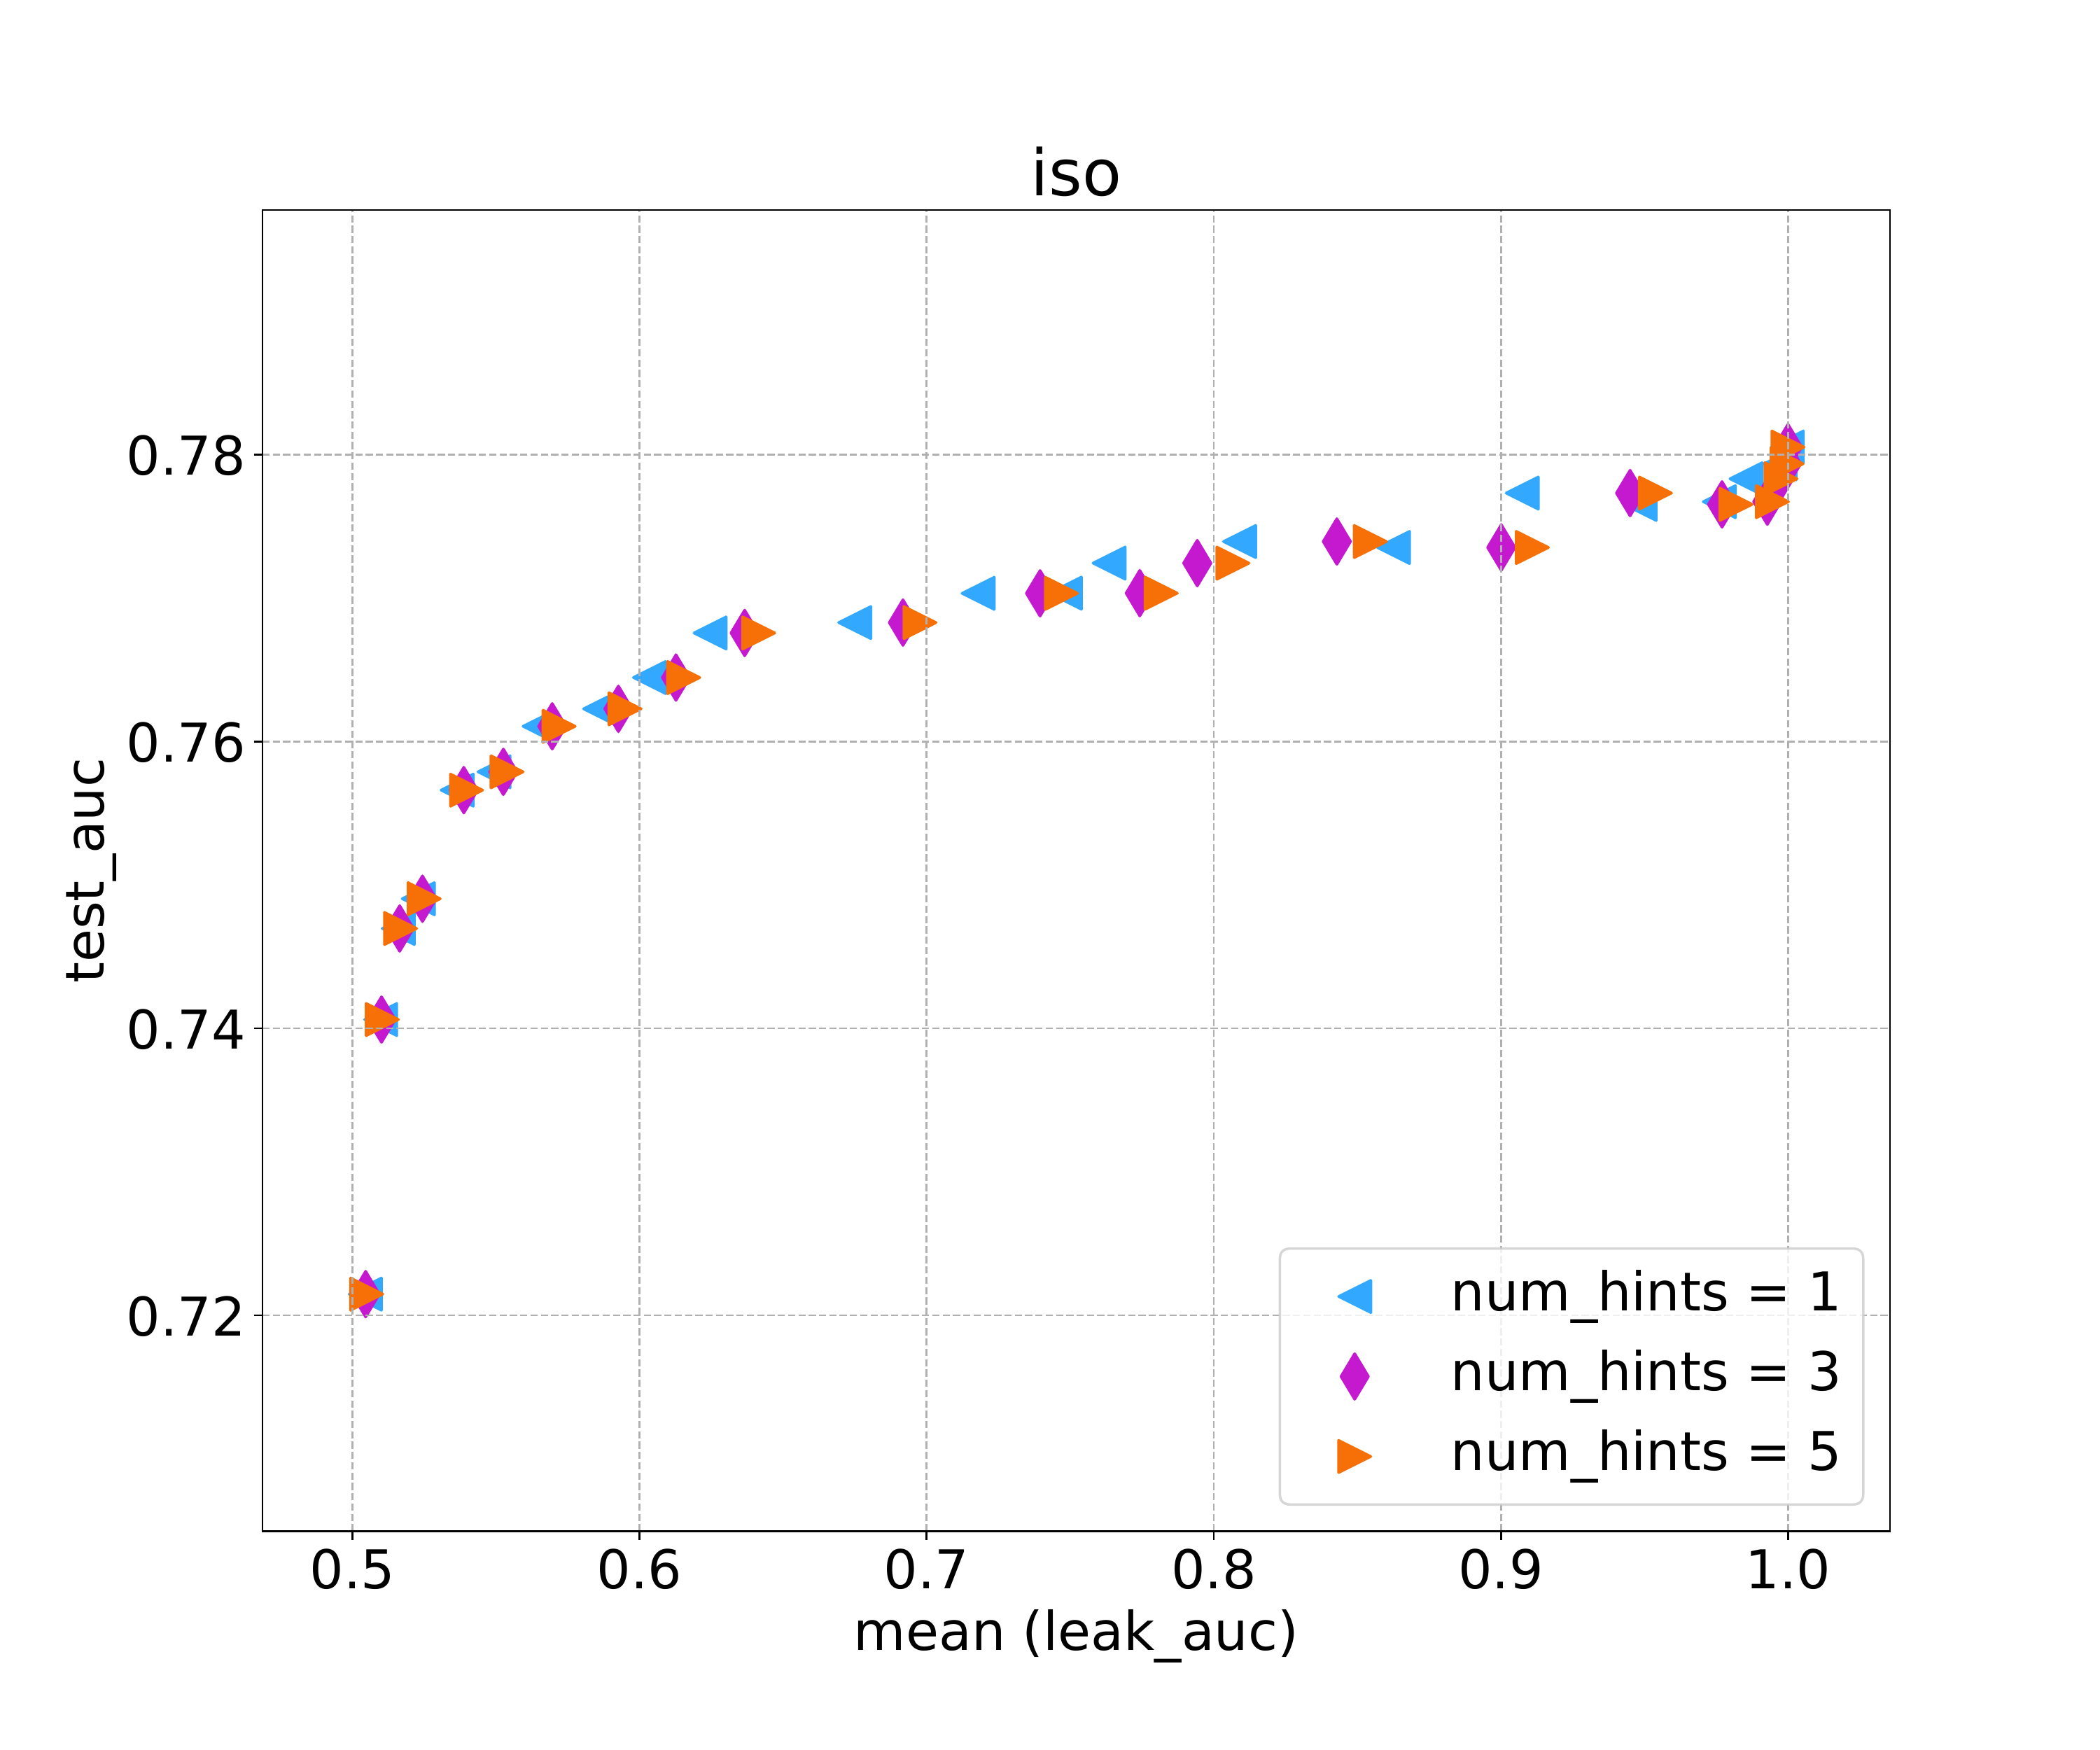}
      \caption*{ (c: )}
  \end{minipage}
  \begin{minipage}[b]{0.495\linewidth}
  \centering
    \includegraphics[width=\linewidth]{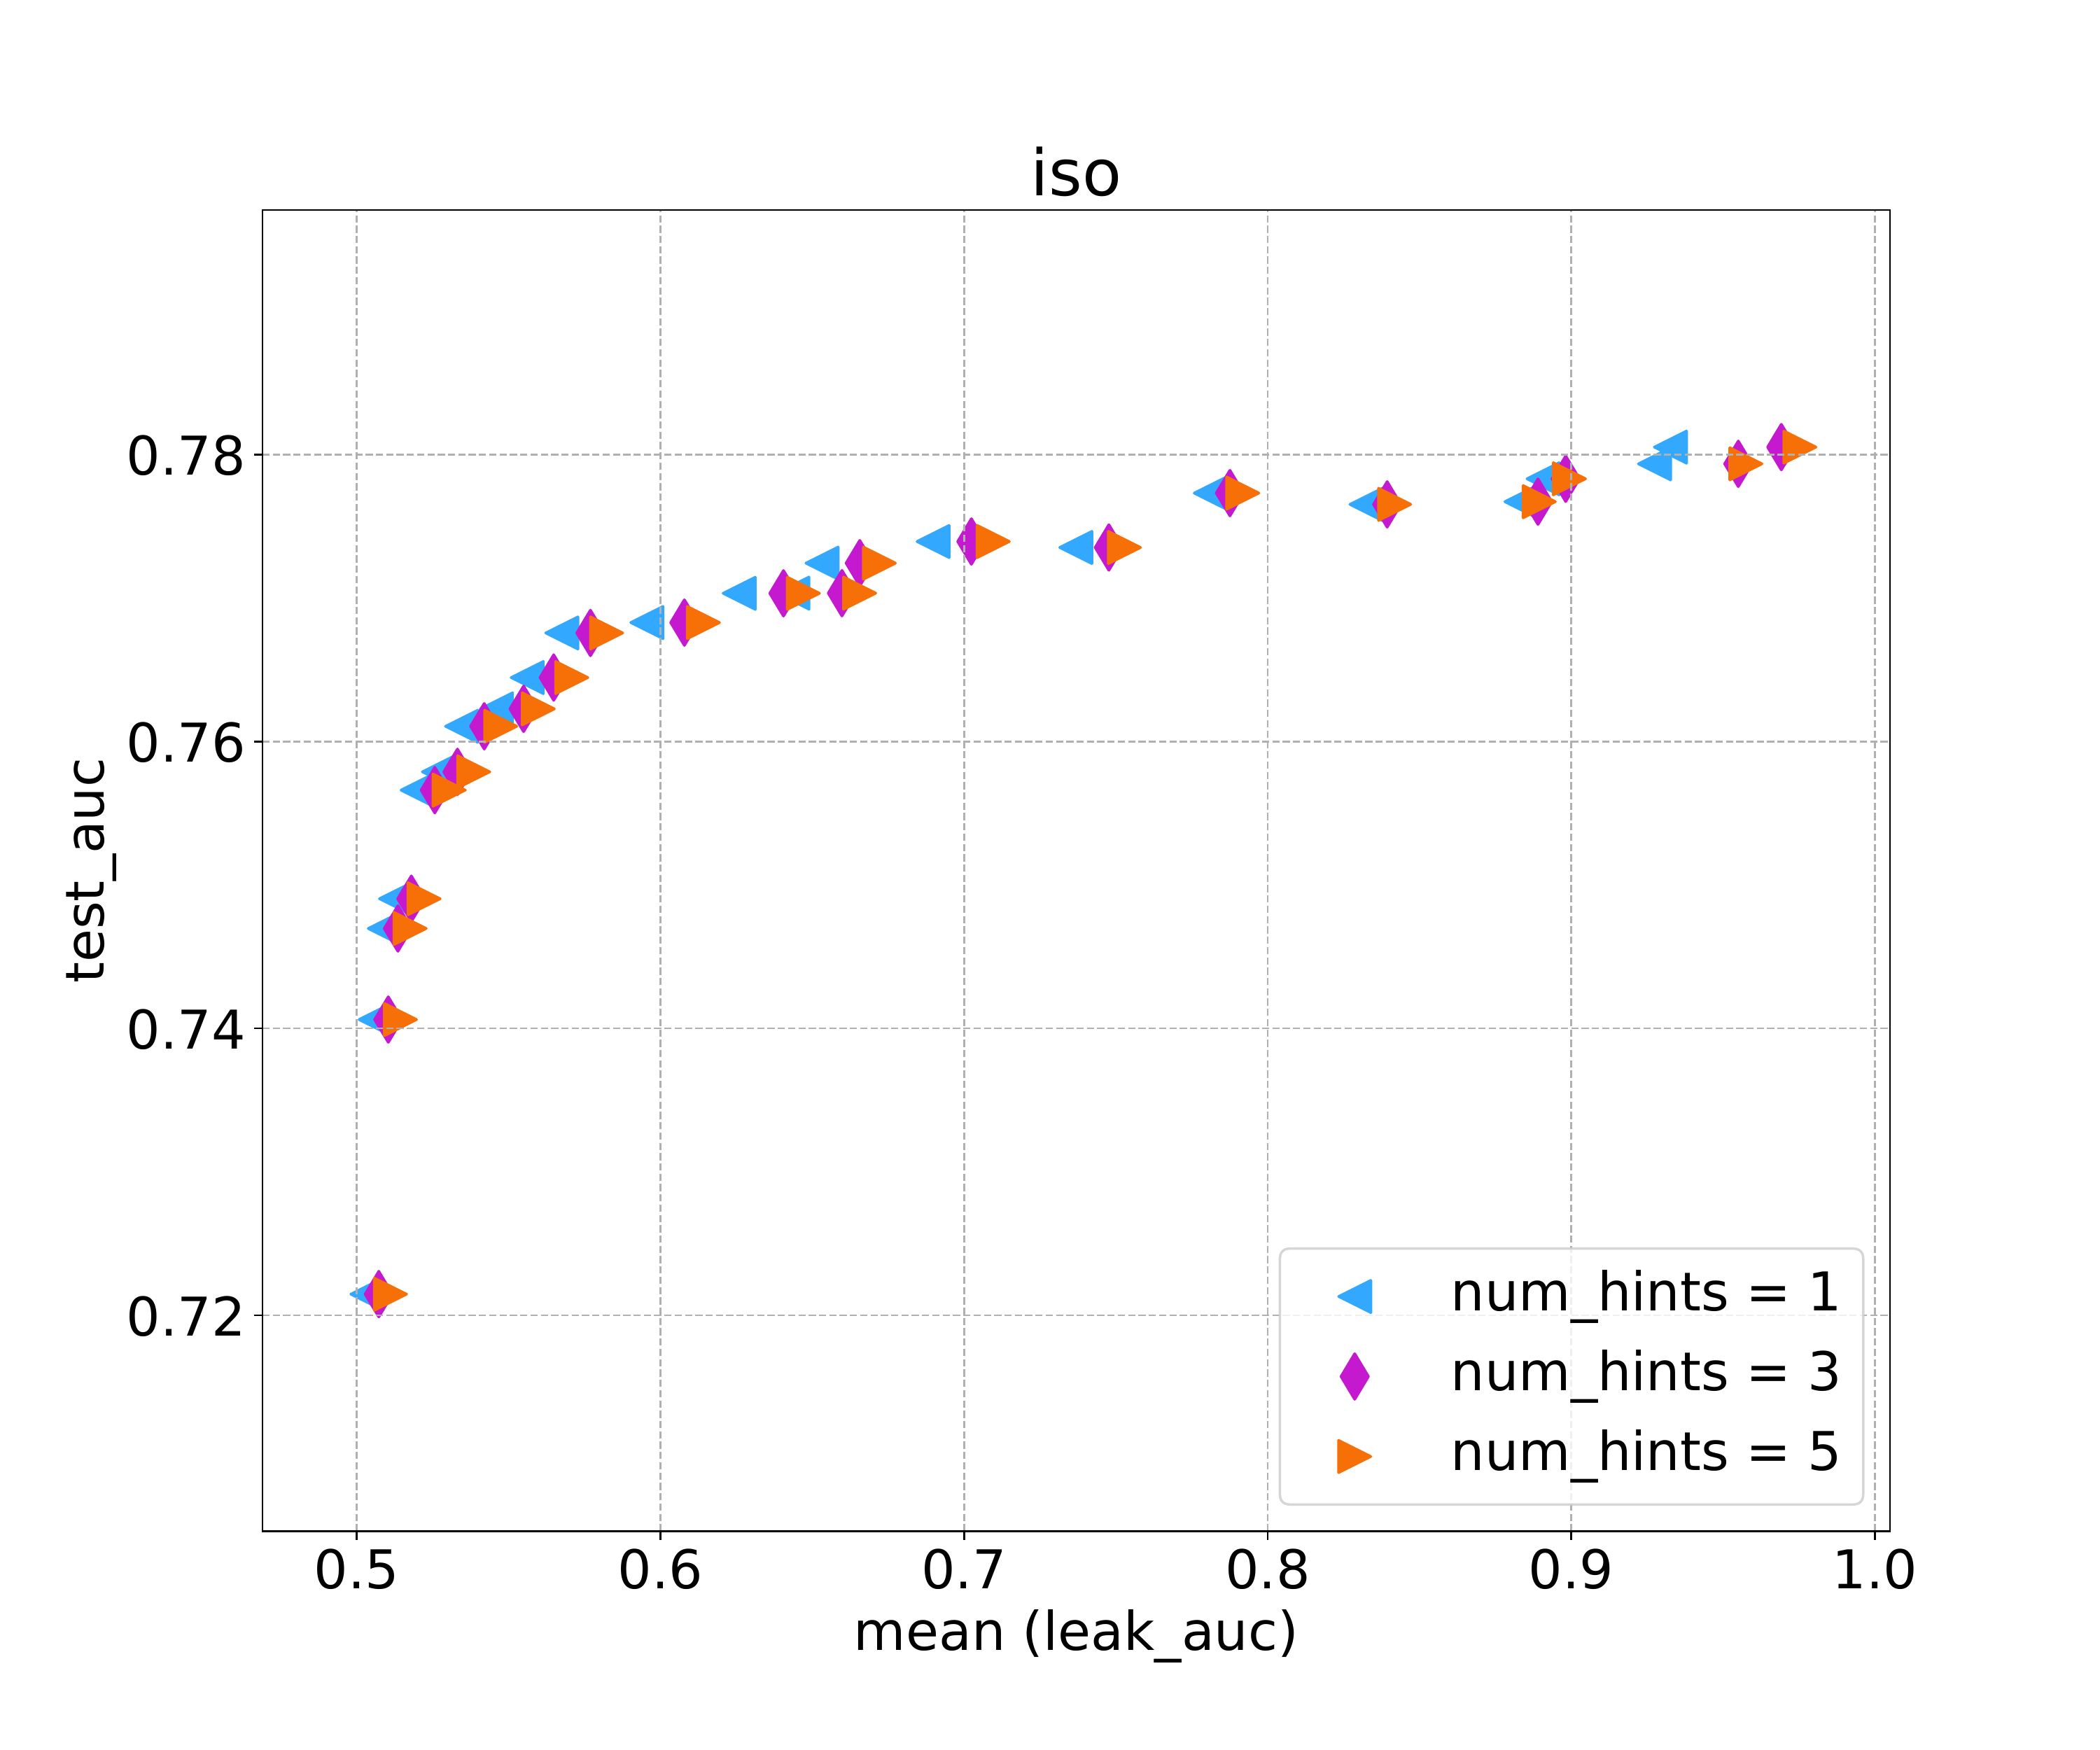}
    \caption*{(d: )}
  \end{minipage}
 \caption{Criteo: effects of num hints on the cut layer}
 \label{fig:criteo_num_hints} 
\end{figure*}


\begin{figure*}[ht!]
  \begin{minipage}[b]{0.495\linewidth}
  \centering
    \includegraphics[width=\linewidth]{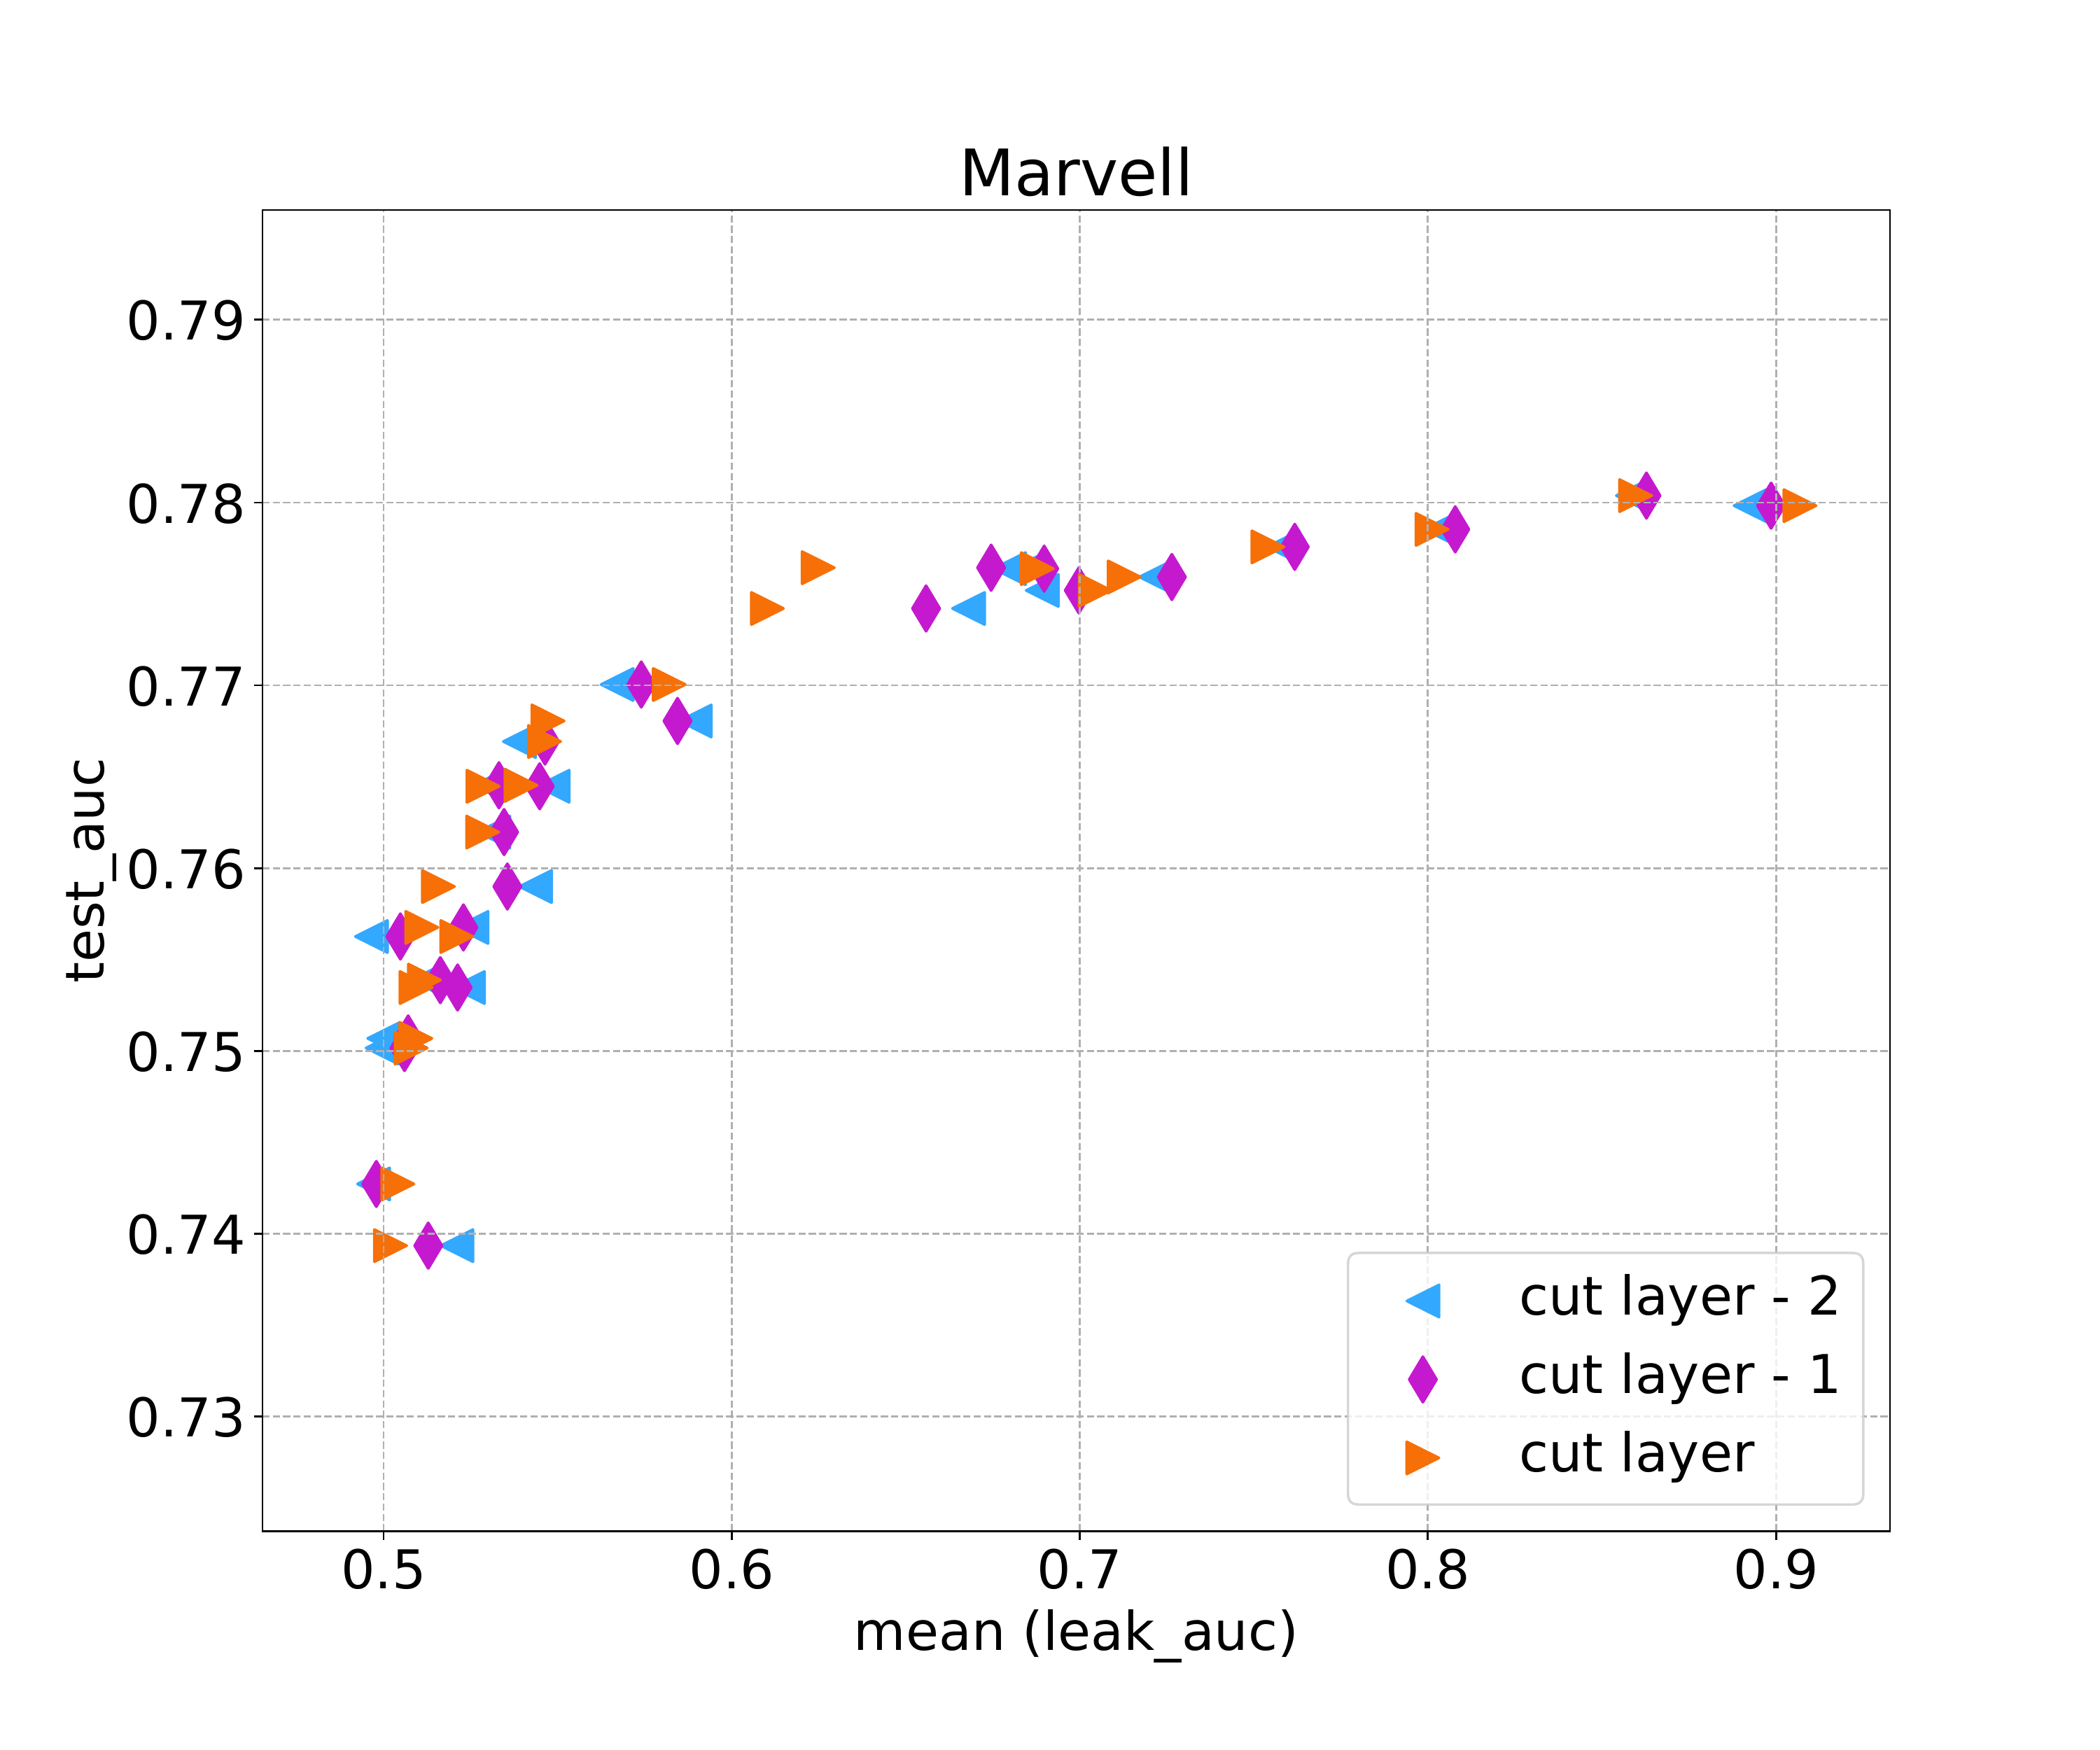}
      \caption*{ (a: norm\_attack\_sumKL\_layer\_position)}
  \end{minipage}
  \begin{minipage}[b]{0.495\linewidth}
  \centering
    \includegraphics[width=\linewidth]{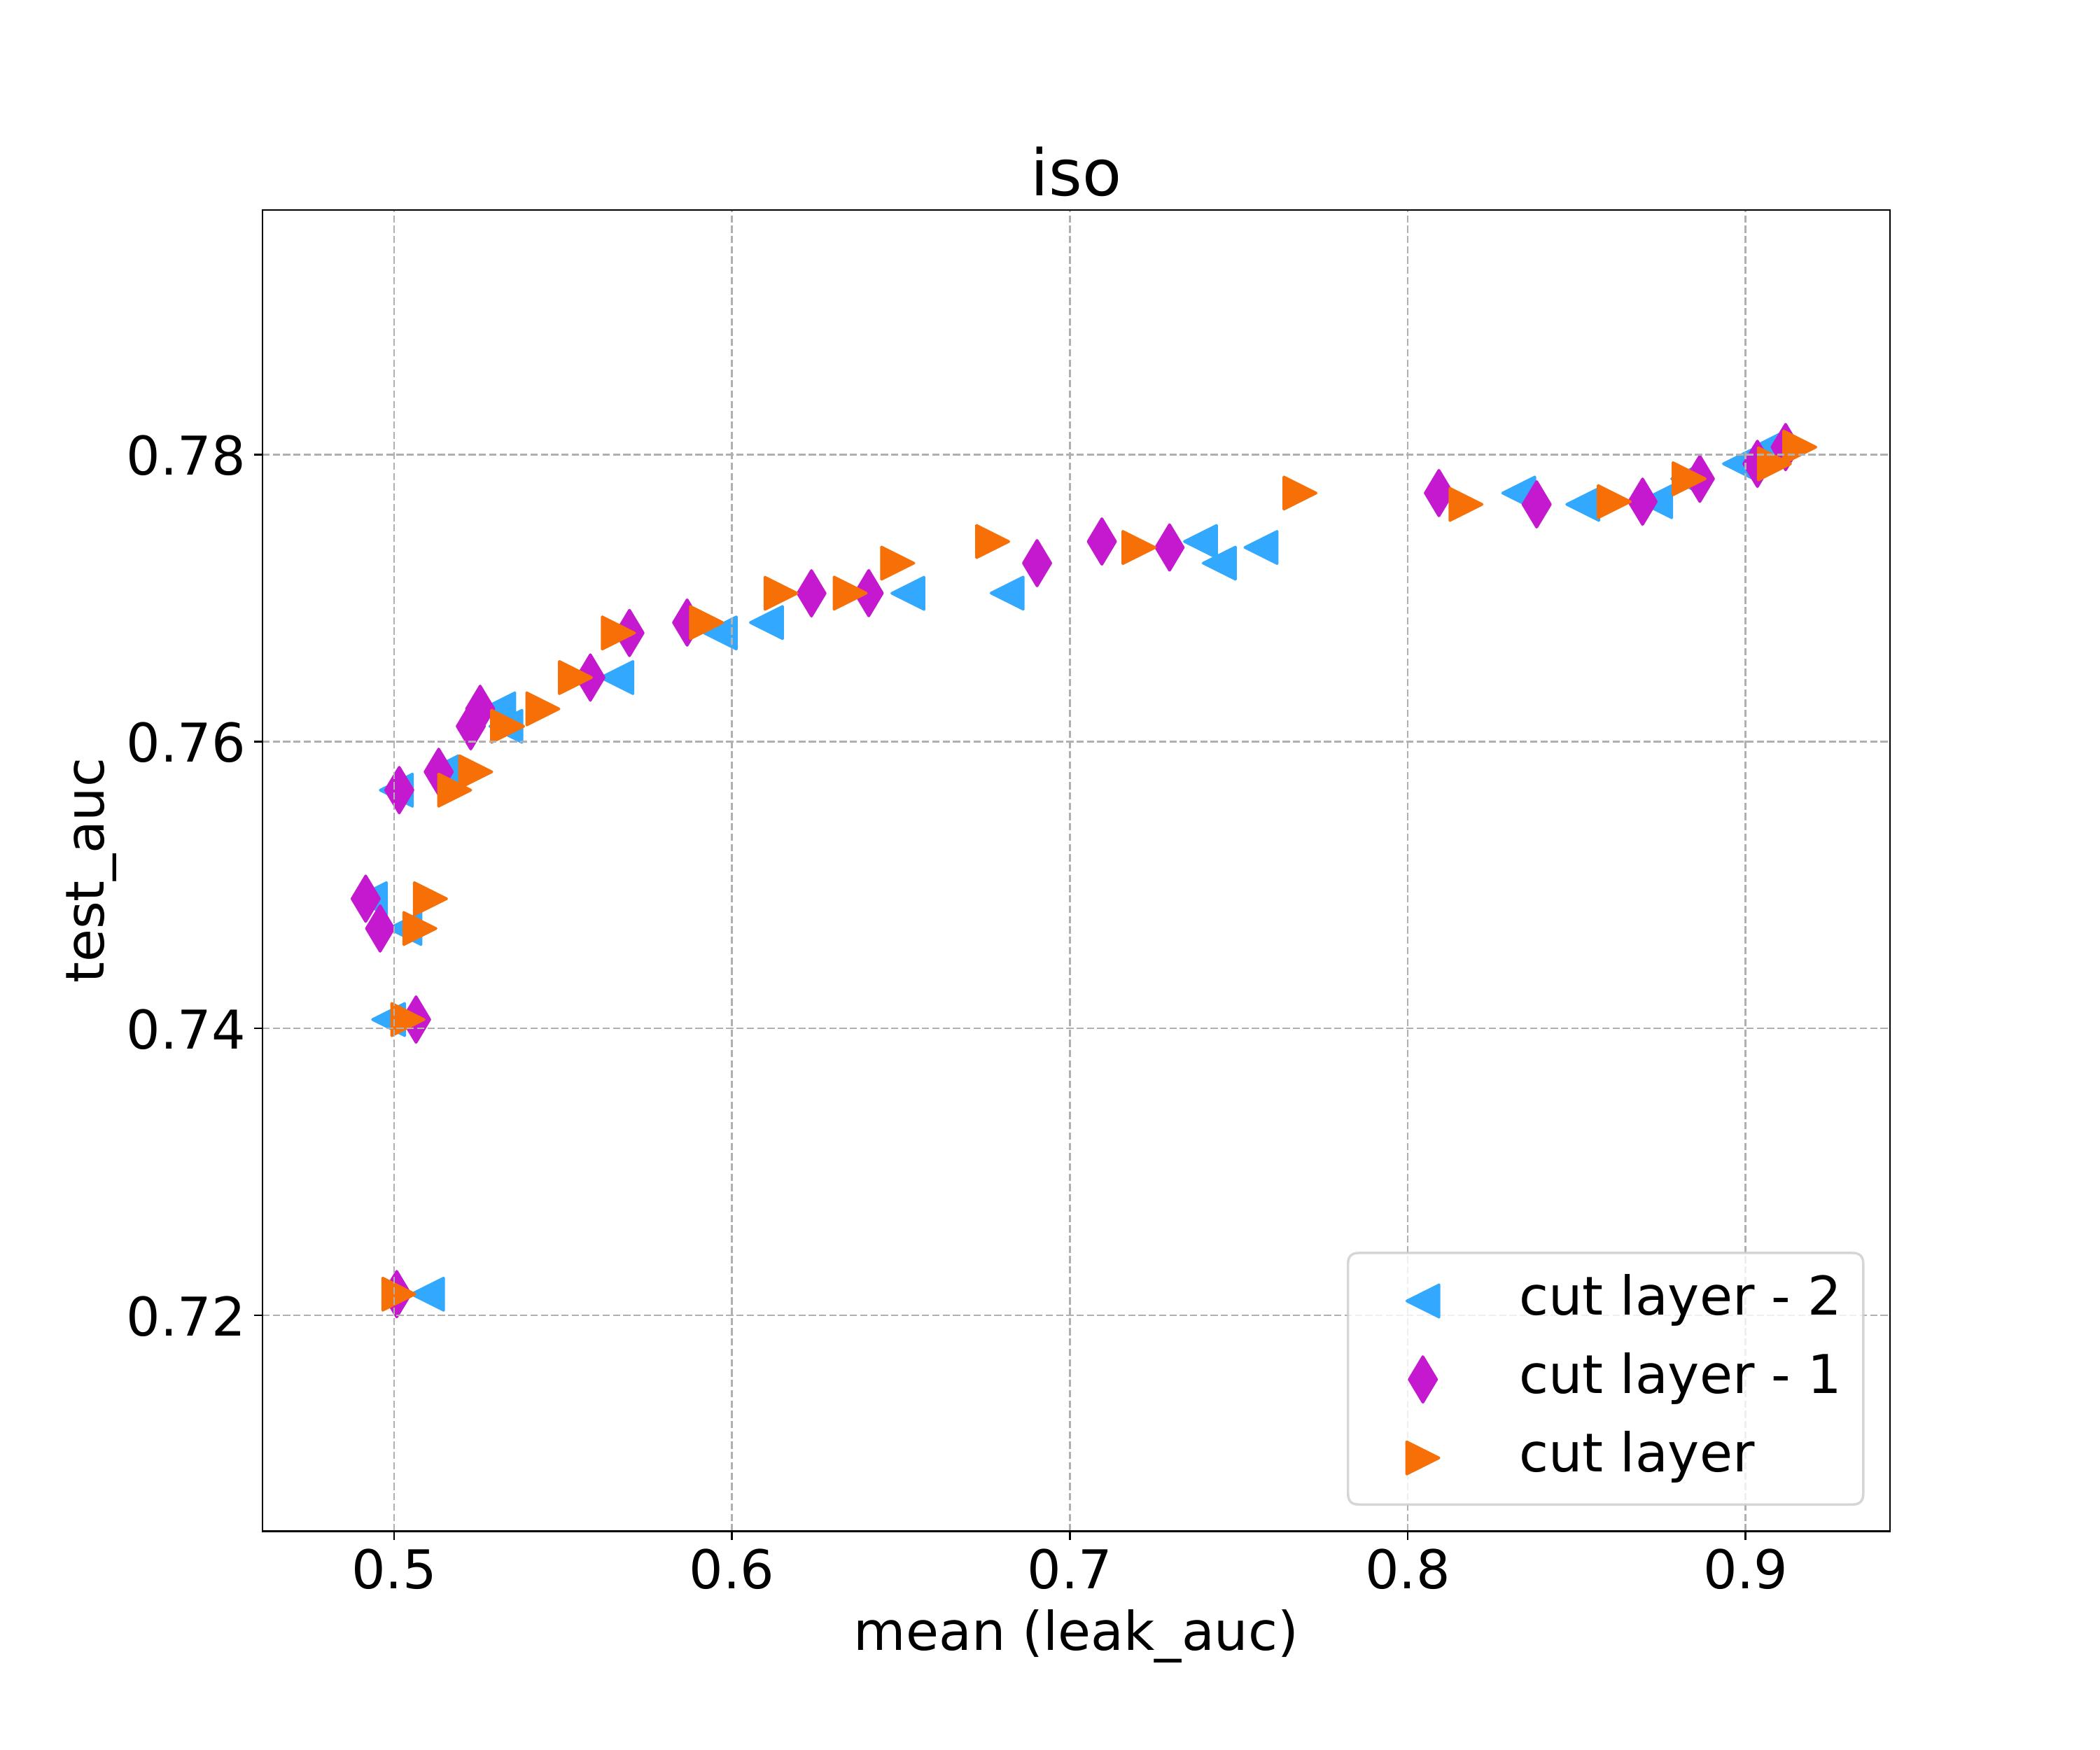}
    \caption*{(b: norm\_attack\_white\_gaussian\_layer\_position)}
  \end{minipage}
  \medskip
  \begin{minipage}[b]{0.495\linewidth}
  \centering
    \includegraphics[width=\linewidth]{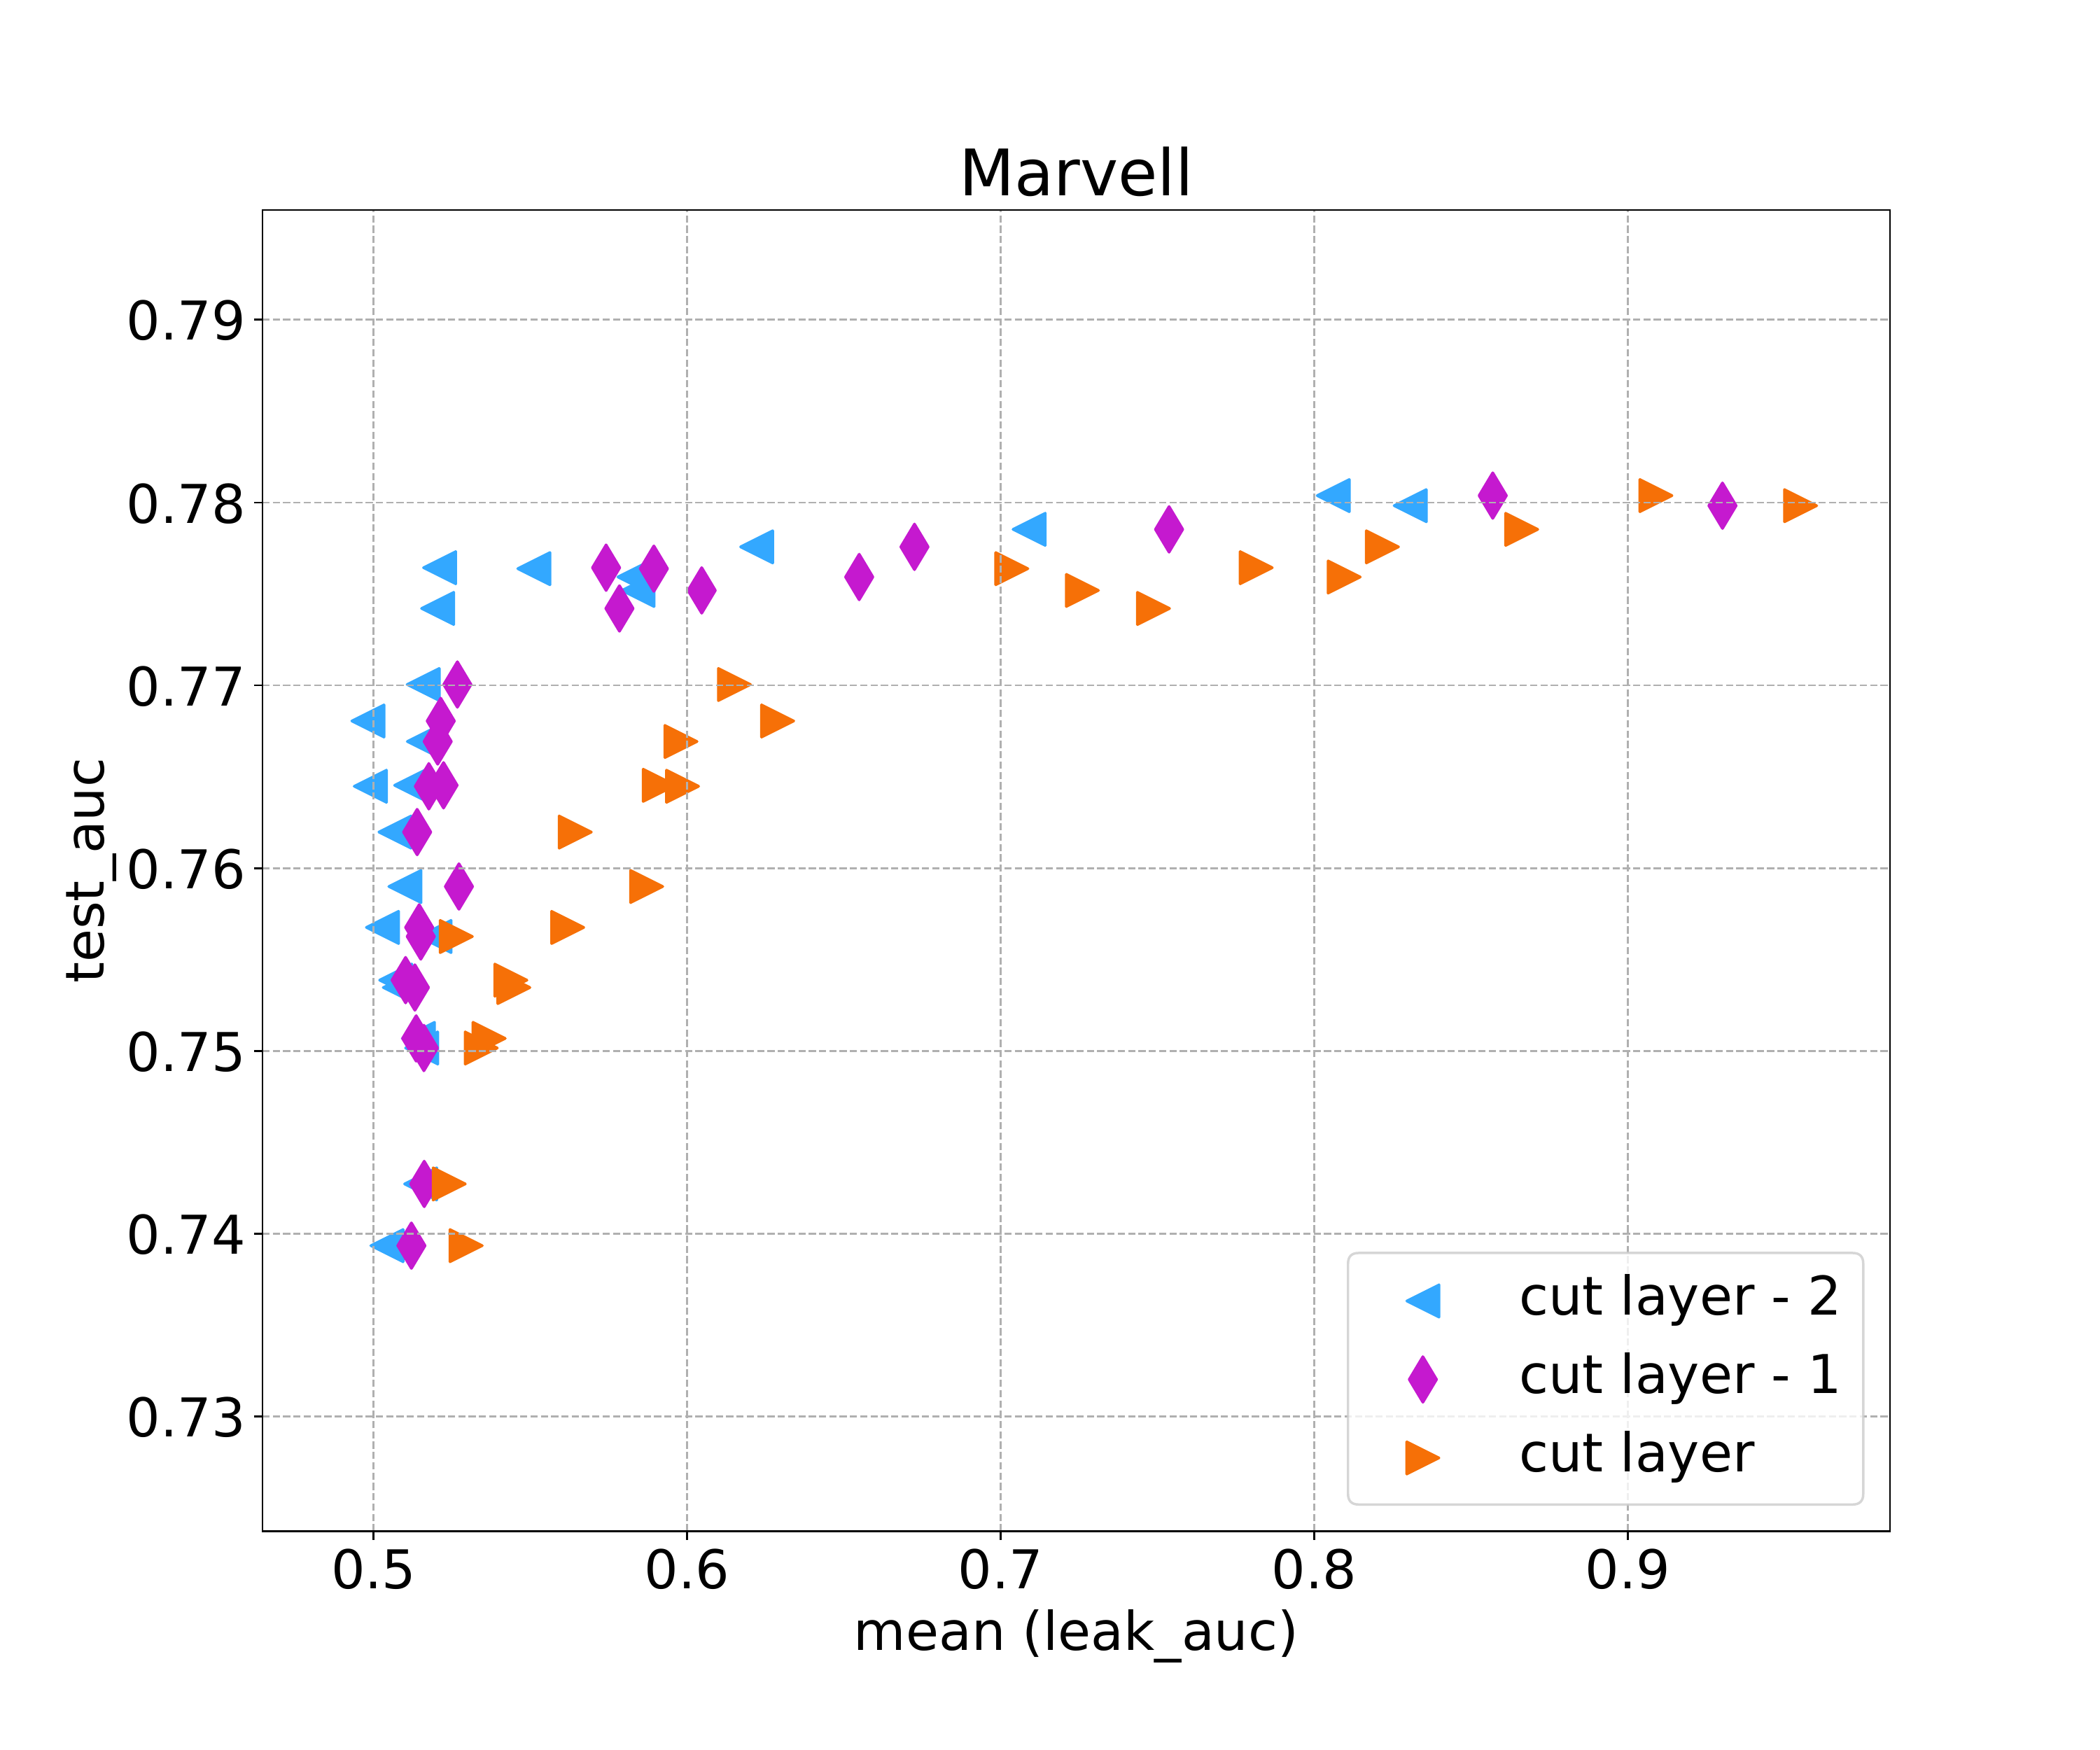}
      \caption*{ (c:sumKL\_mean\_hint\_norm\_attack\_layer\_position )}
  \end{minipage}
  \begin{minipage}[b]{0.495\linewidth}
  \centering
    \includegraphics[width=\linewidth]{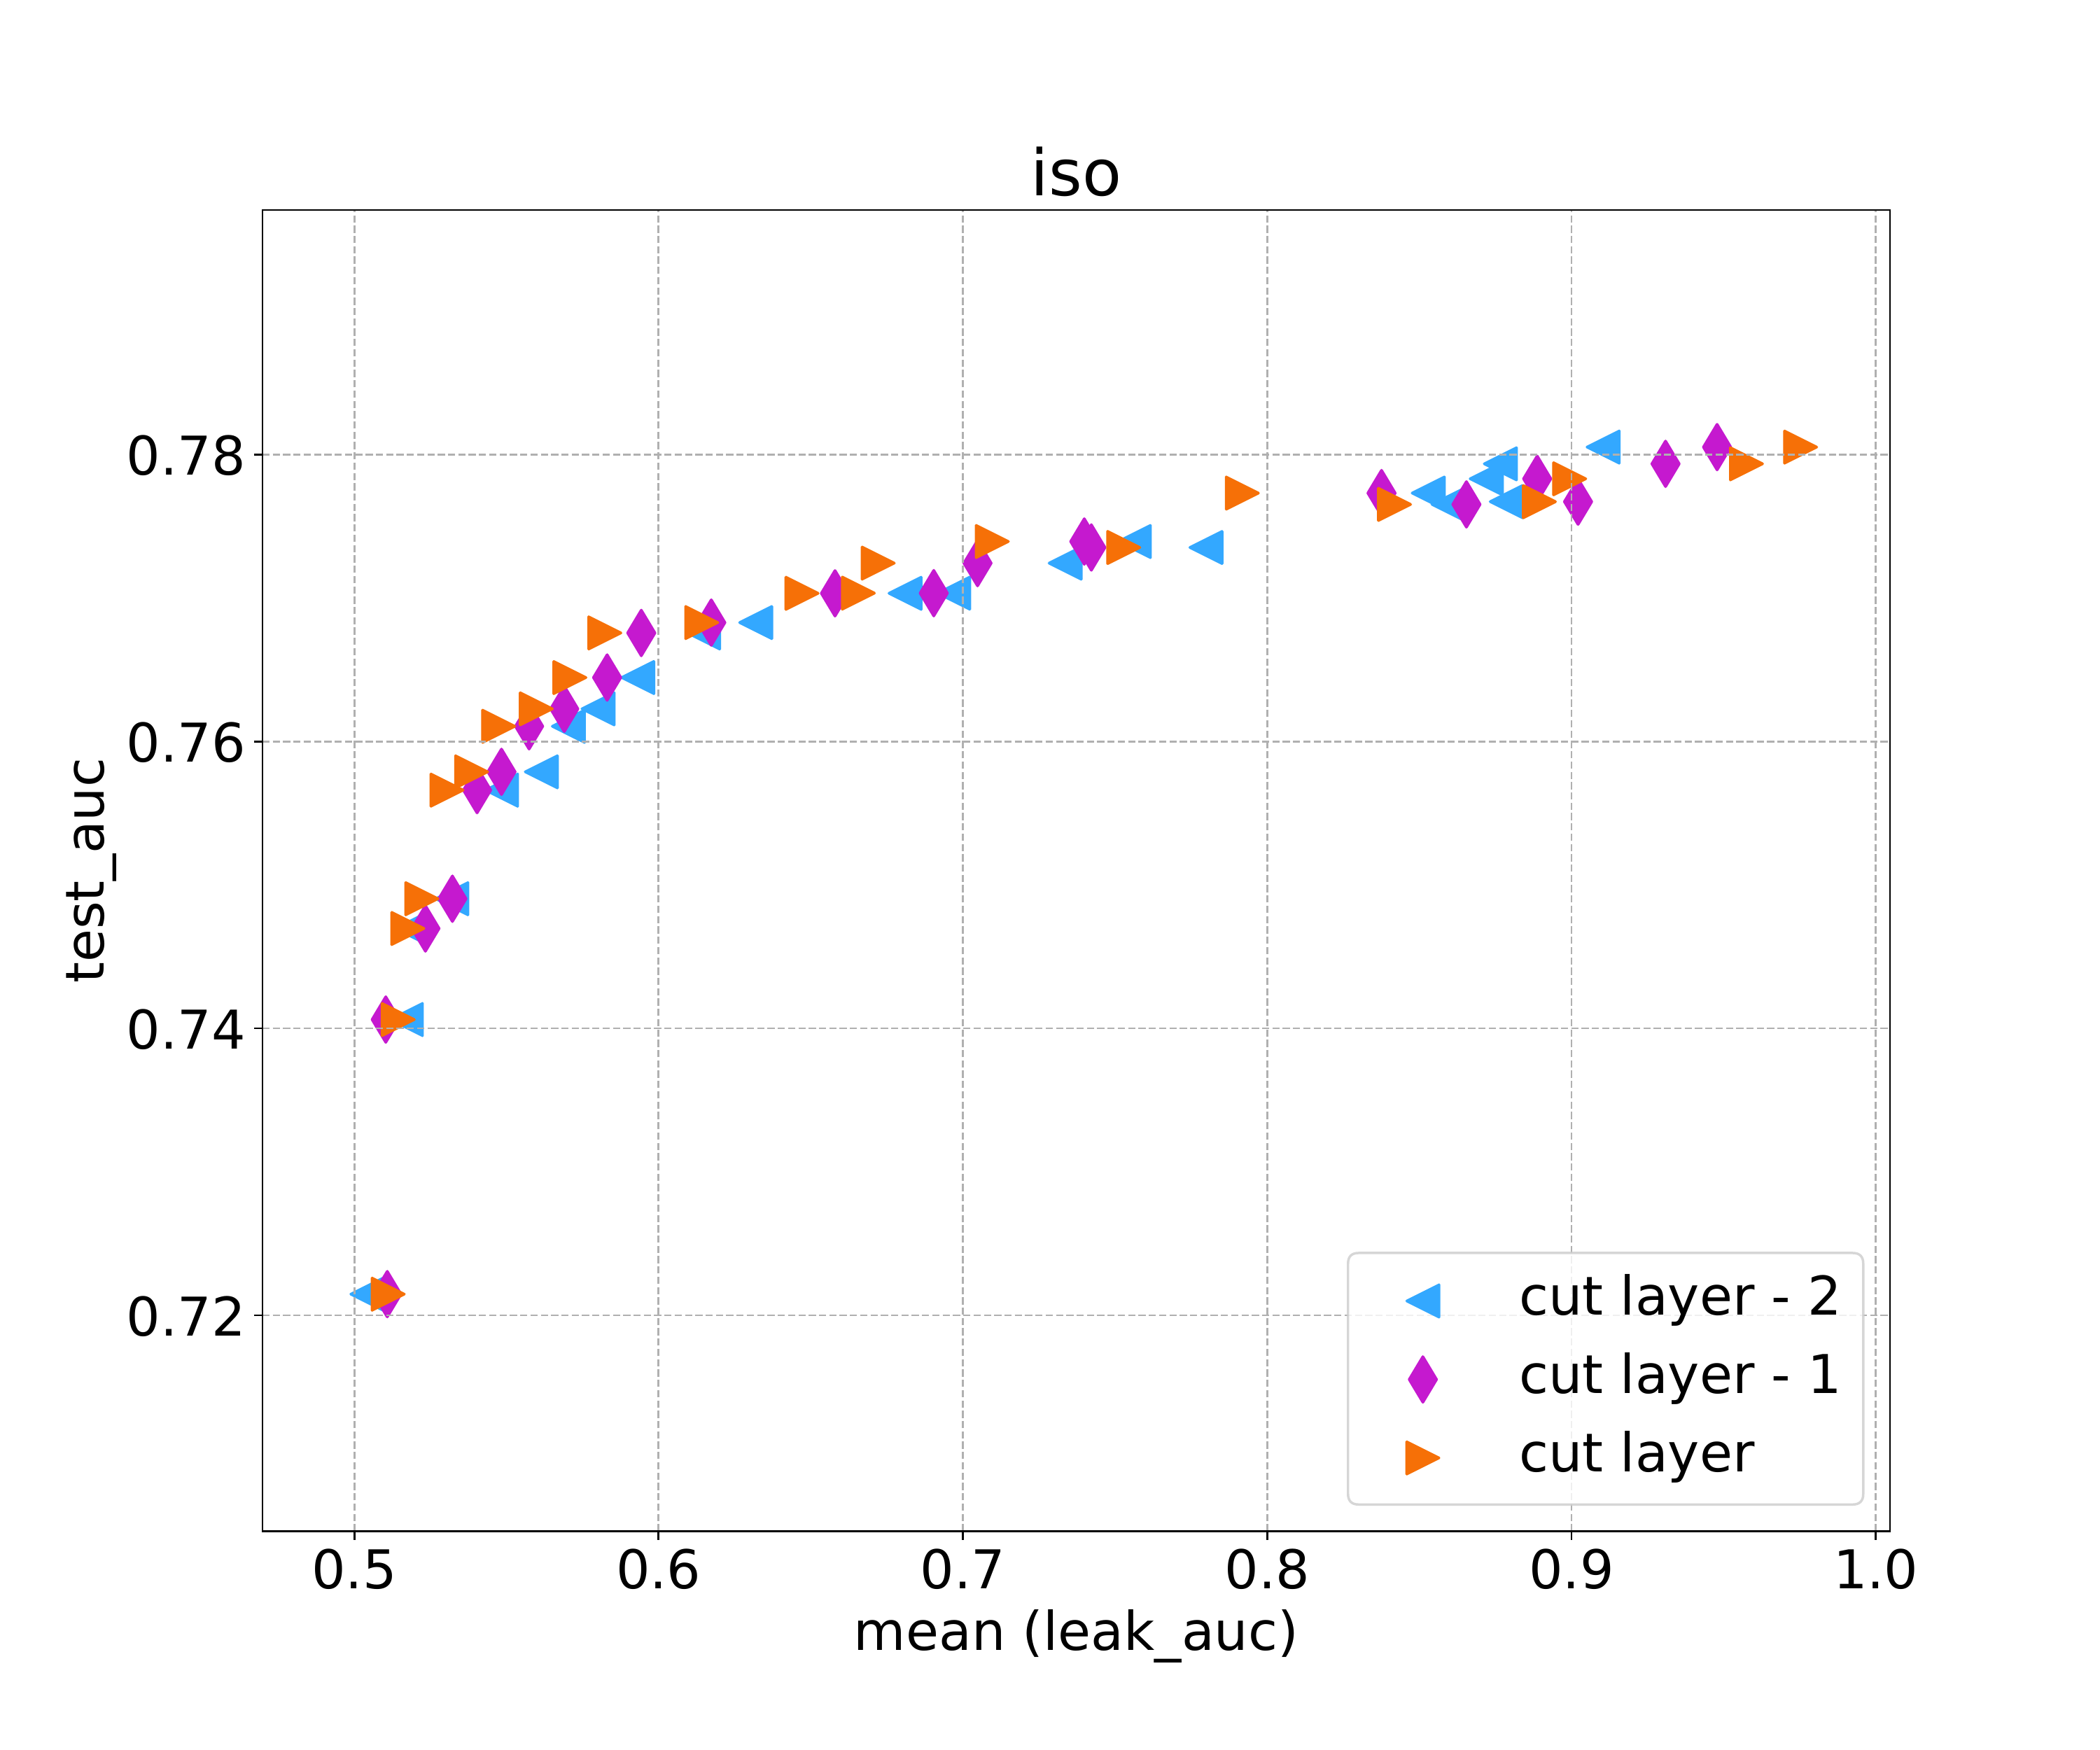}
    \caption*{(d: white\_gaussian\_mean\_hint\_norm\_attack\_layer\_position)}
  \end{minipage}
  \medskip
  \begin{minipage}[b]{0.495\linewidth}
  \centering
    \includegraphics[width=\linewidth]{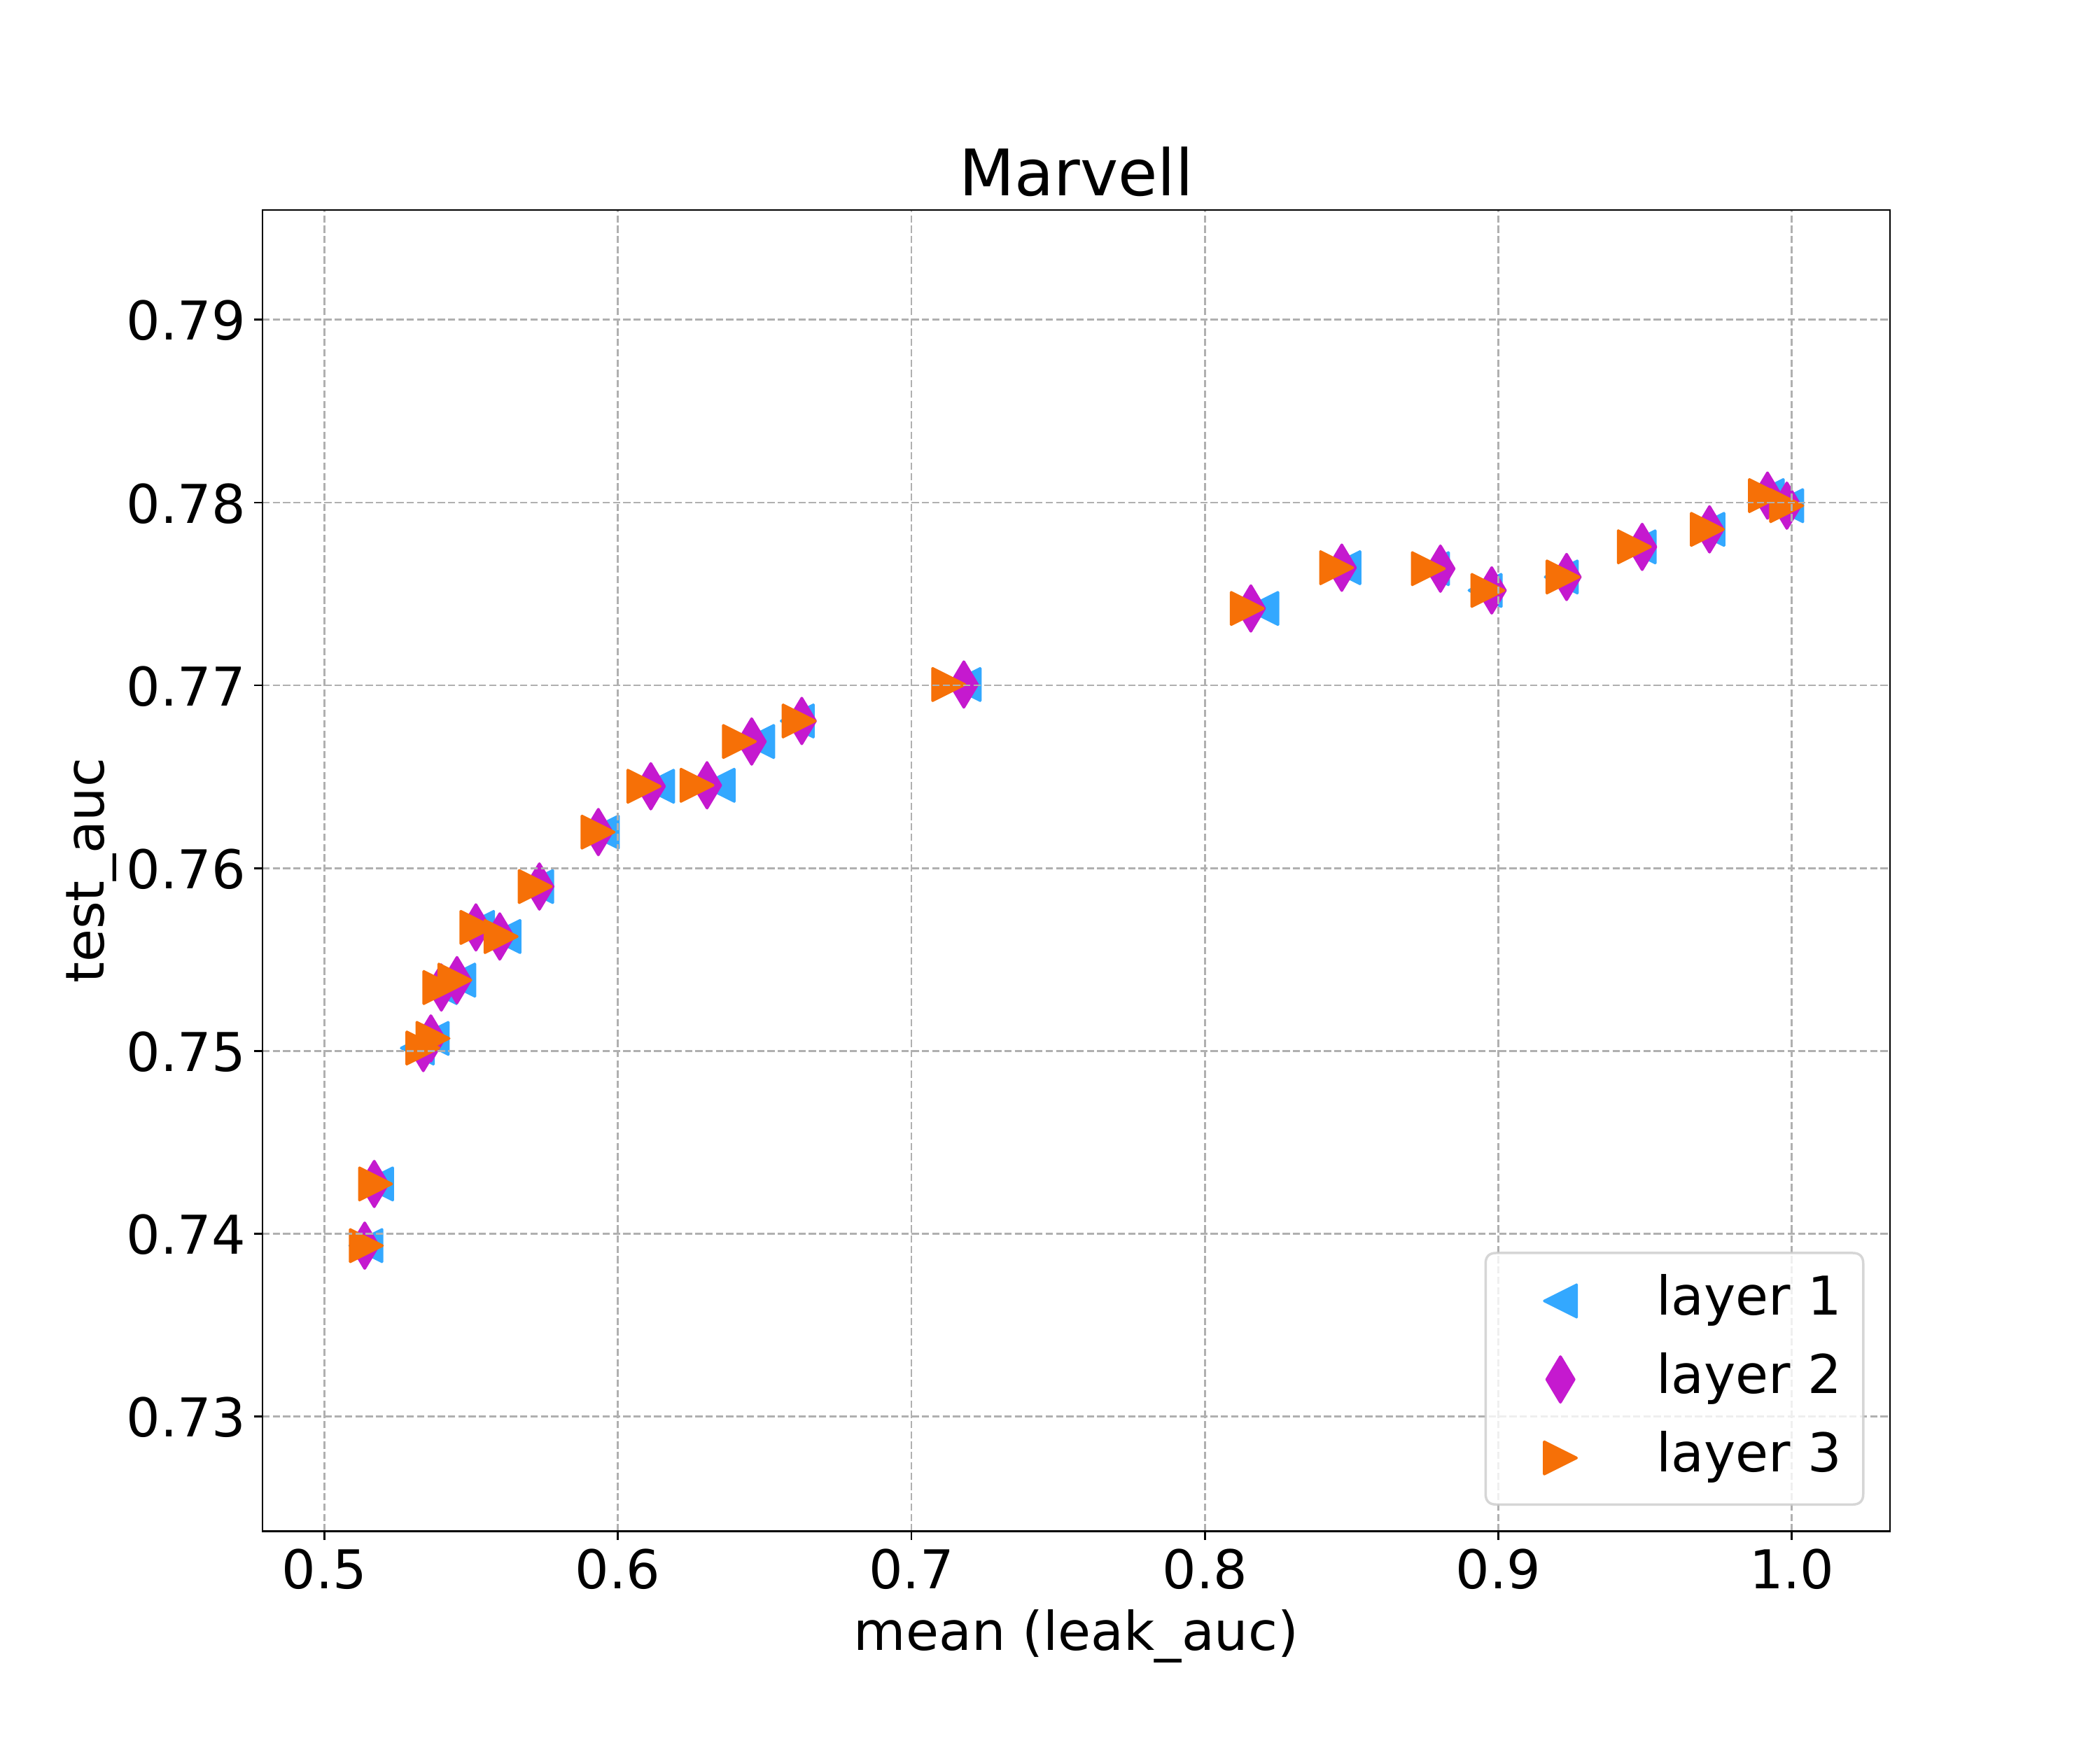}
      \caption*{ (e:sumKL\_mean\_hint\_ip\_attack\_layer\_position )}
  \end{minipage}
  \begin{minipage}[b]{0.495\linewidth}
  \centering
    \includegraphics[width=\linewidth]{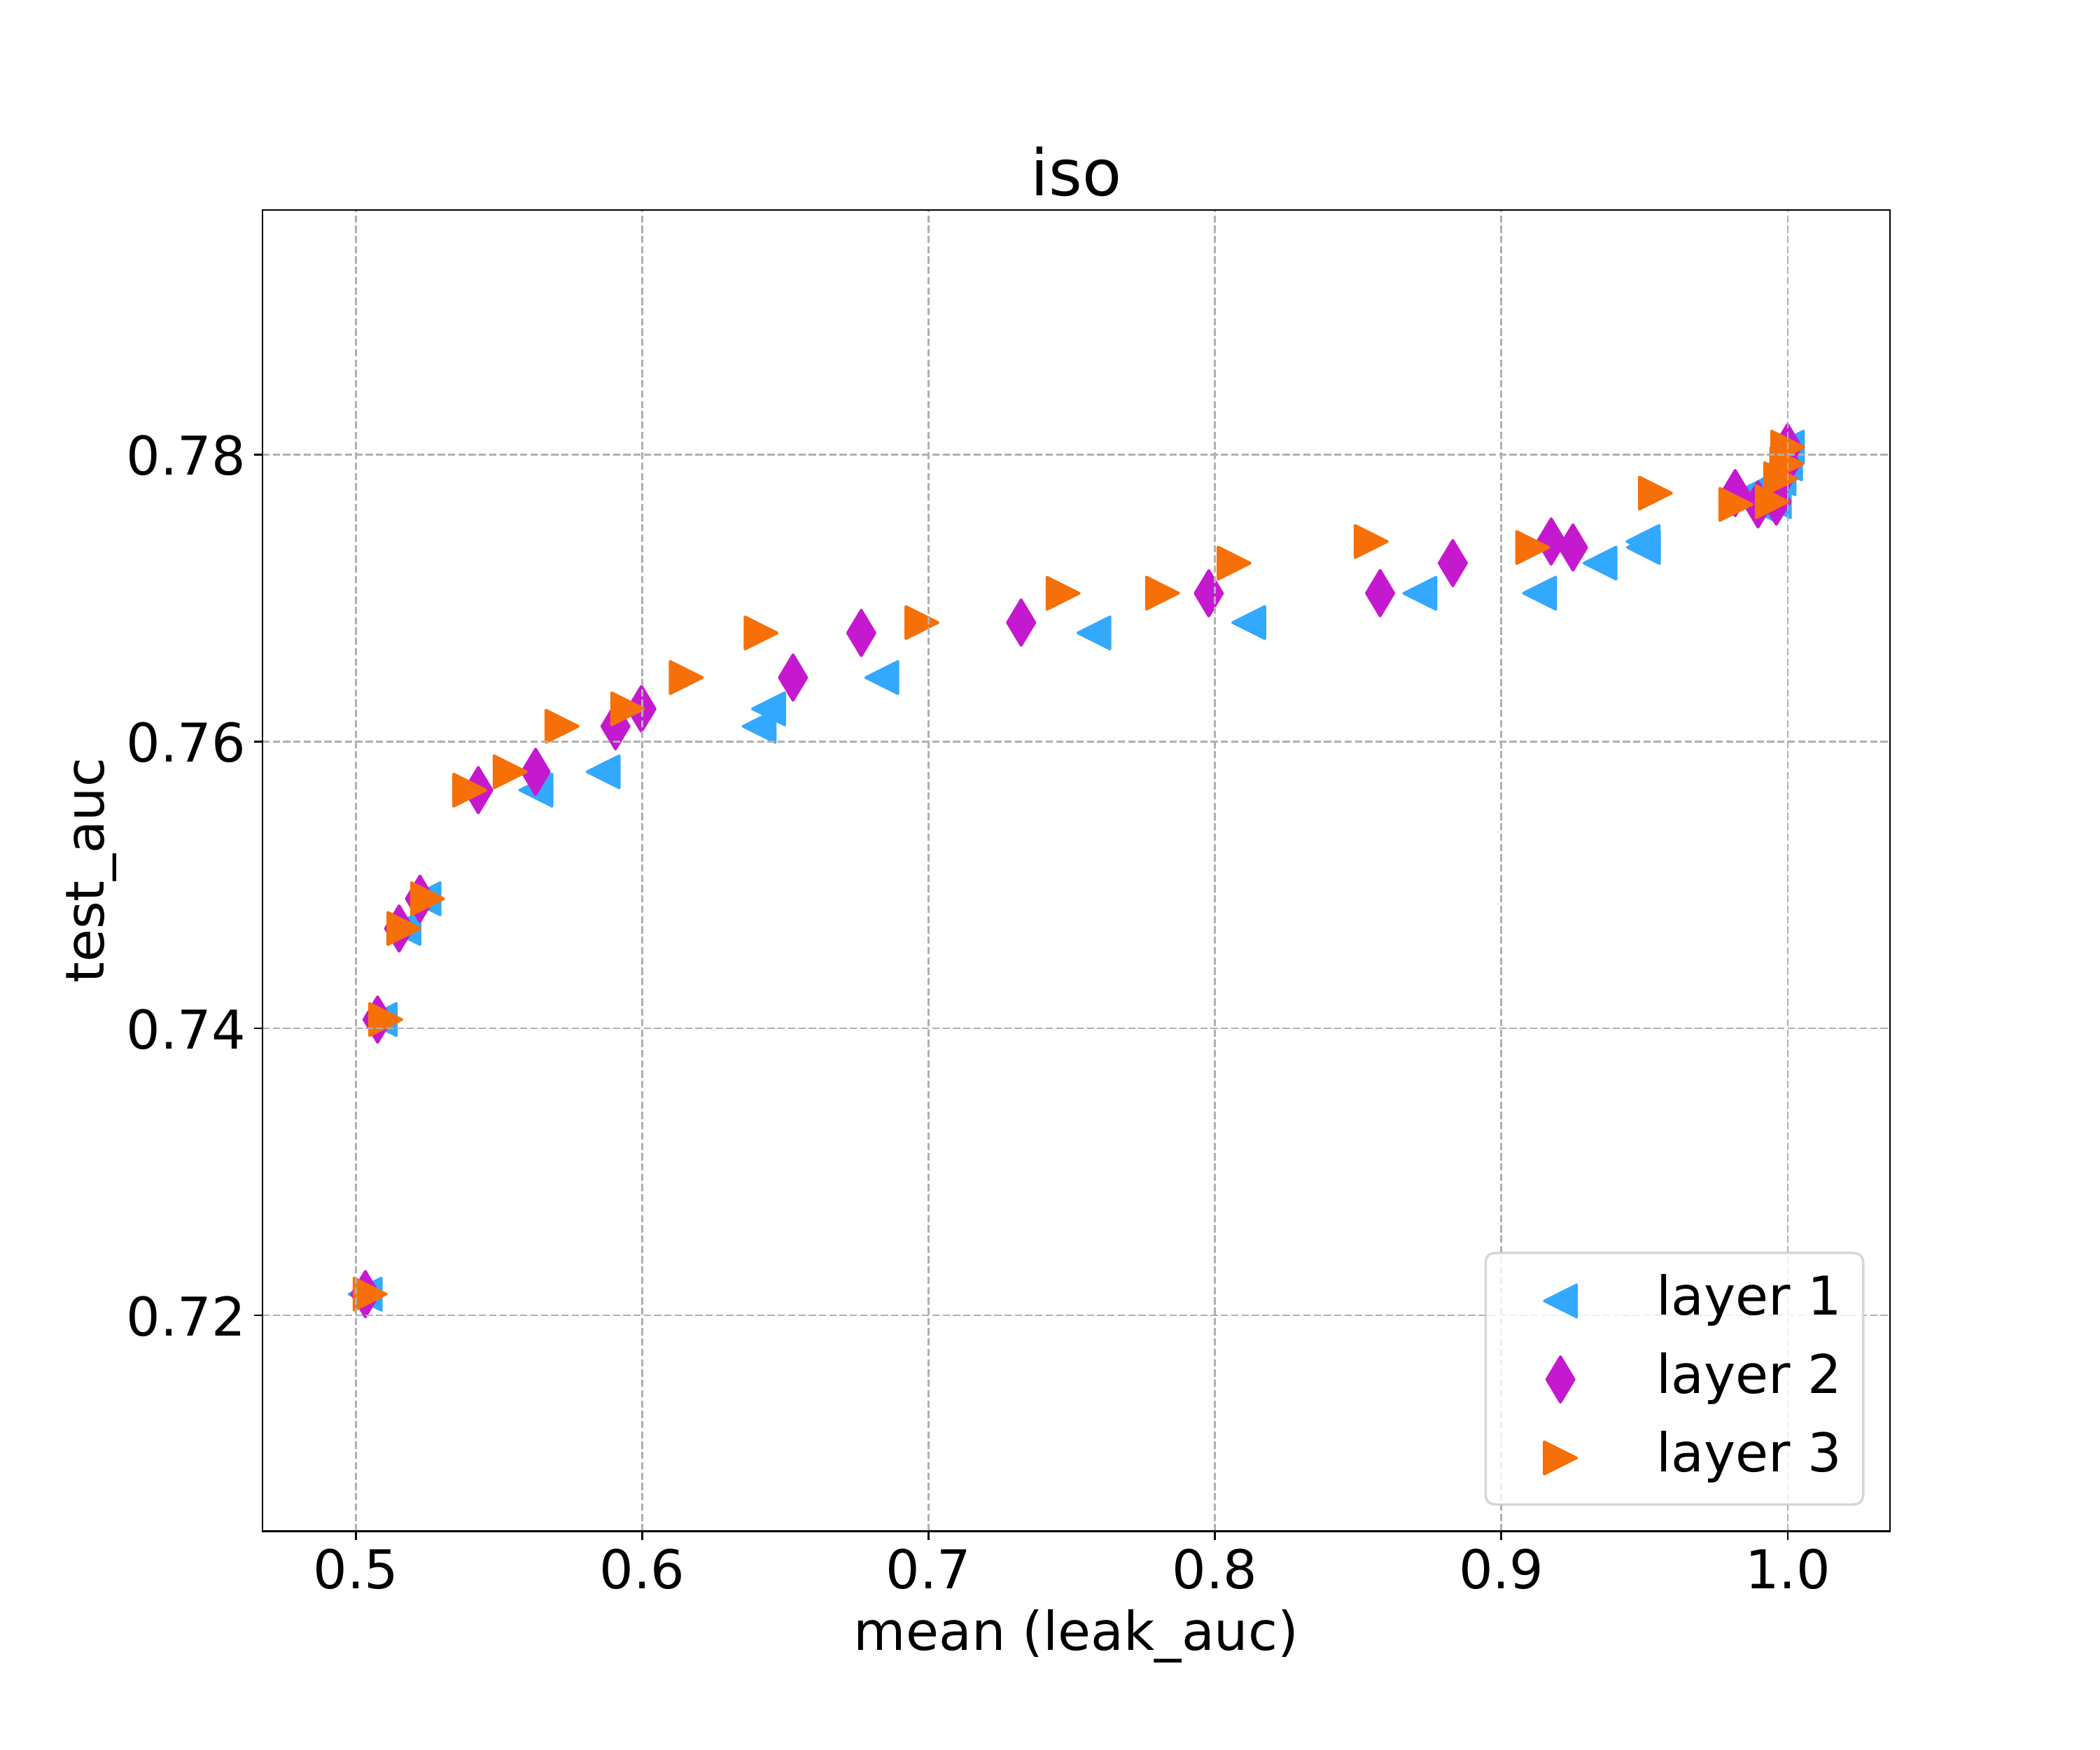}
    \caption*{(f: white\_gaussian\_mean\_hint\_ip\_attack\_layer\_position)}
  \end{minipage}
 \caption{Criteo: effects of layer position}
 \label{fig:criteo_layer_position} 
\end{figure*}

\begin{figure*}[ht!]
  \begin{minipage}[b]{0.495\linewidth}
  \centering
    \includegraphics[width=\linewidth]{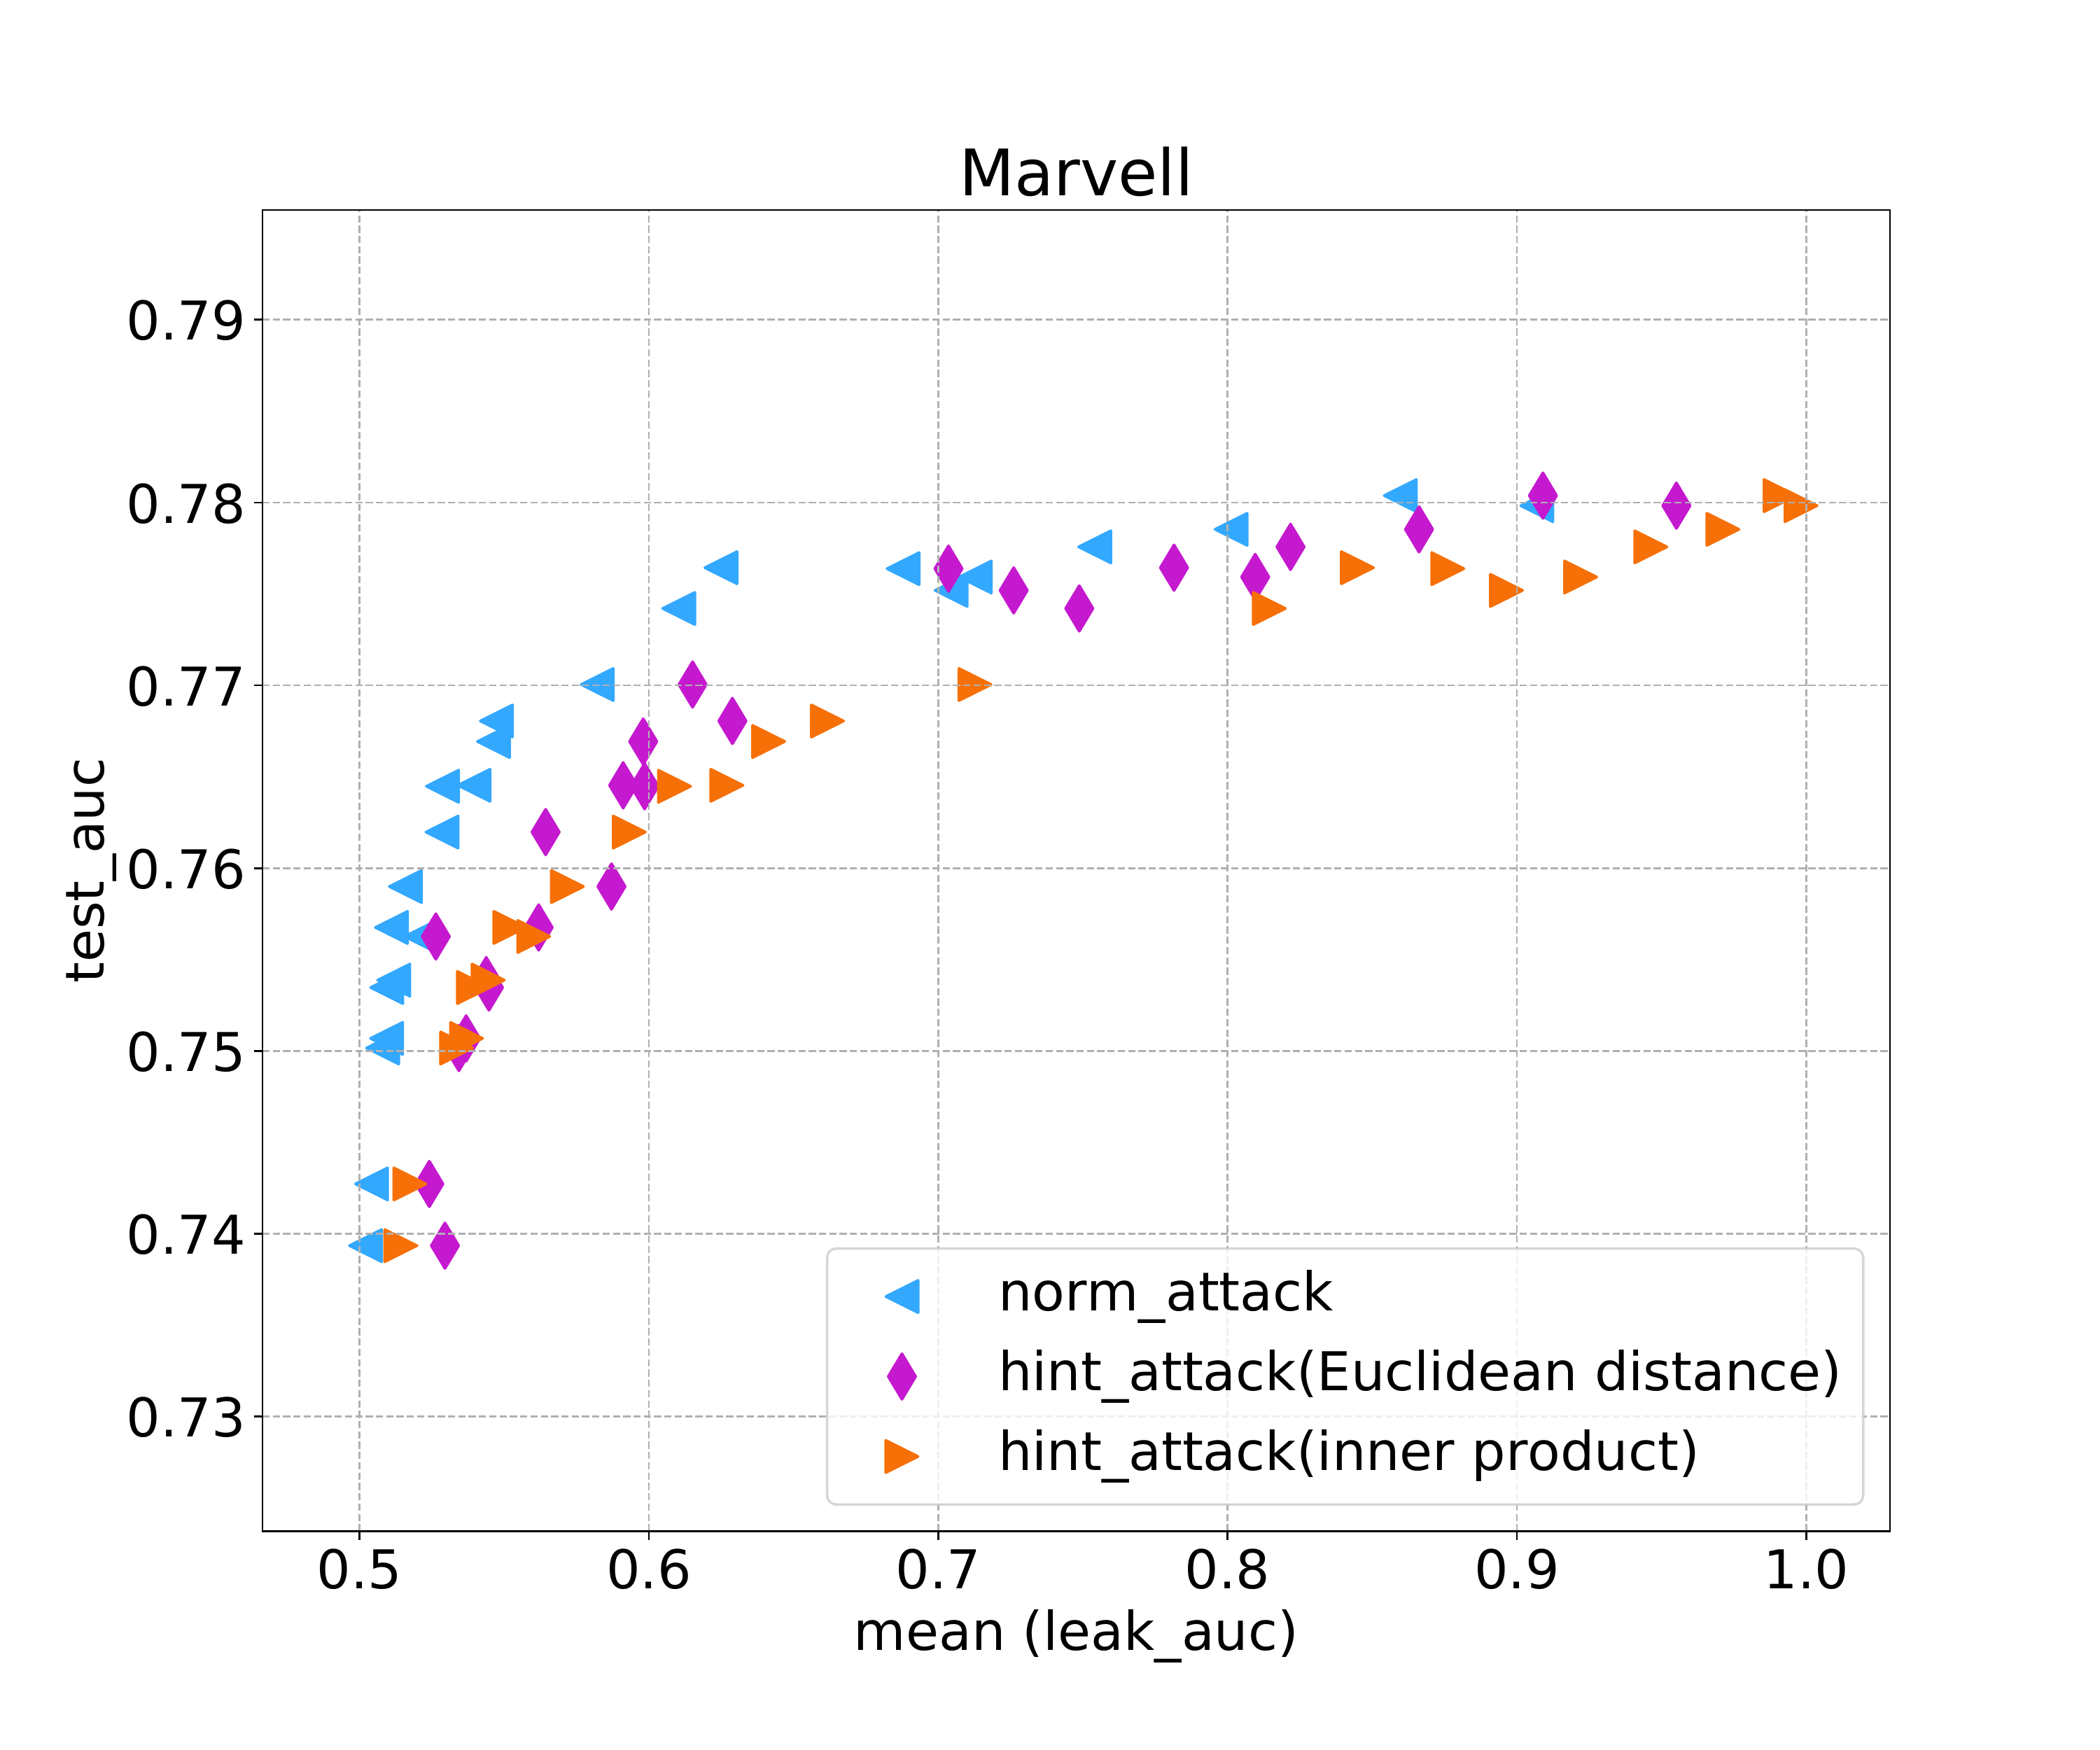}
      \caption*{ (a: sumKL_against_different_attack_methods)}
  \end{minipage}
  \begin{minipage}[b]{0.495\linewidth}
  \centering
    \includegraphics[width=\linewidth]{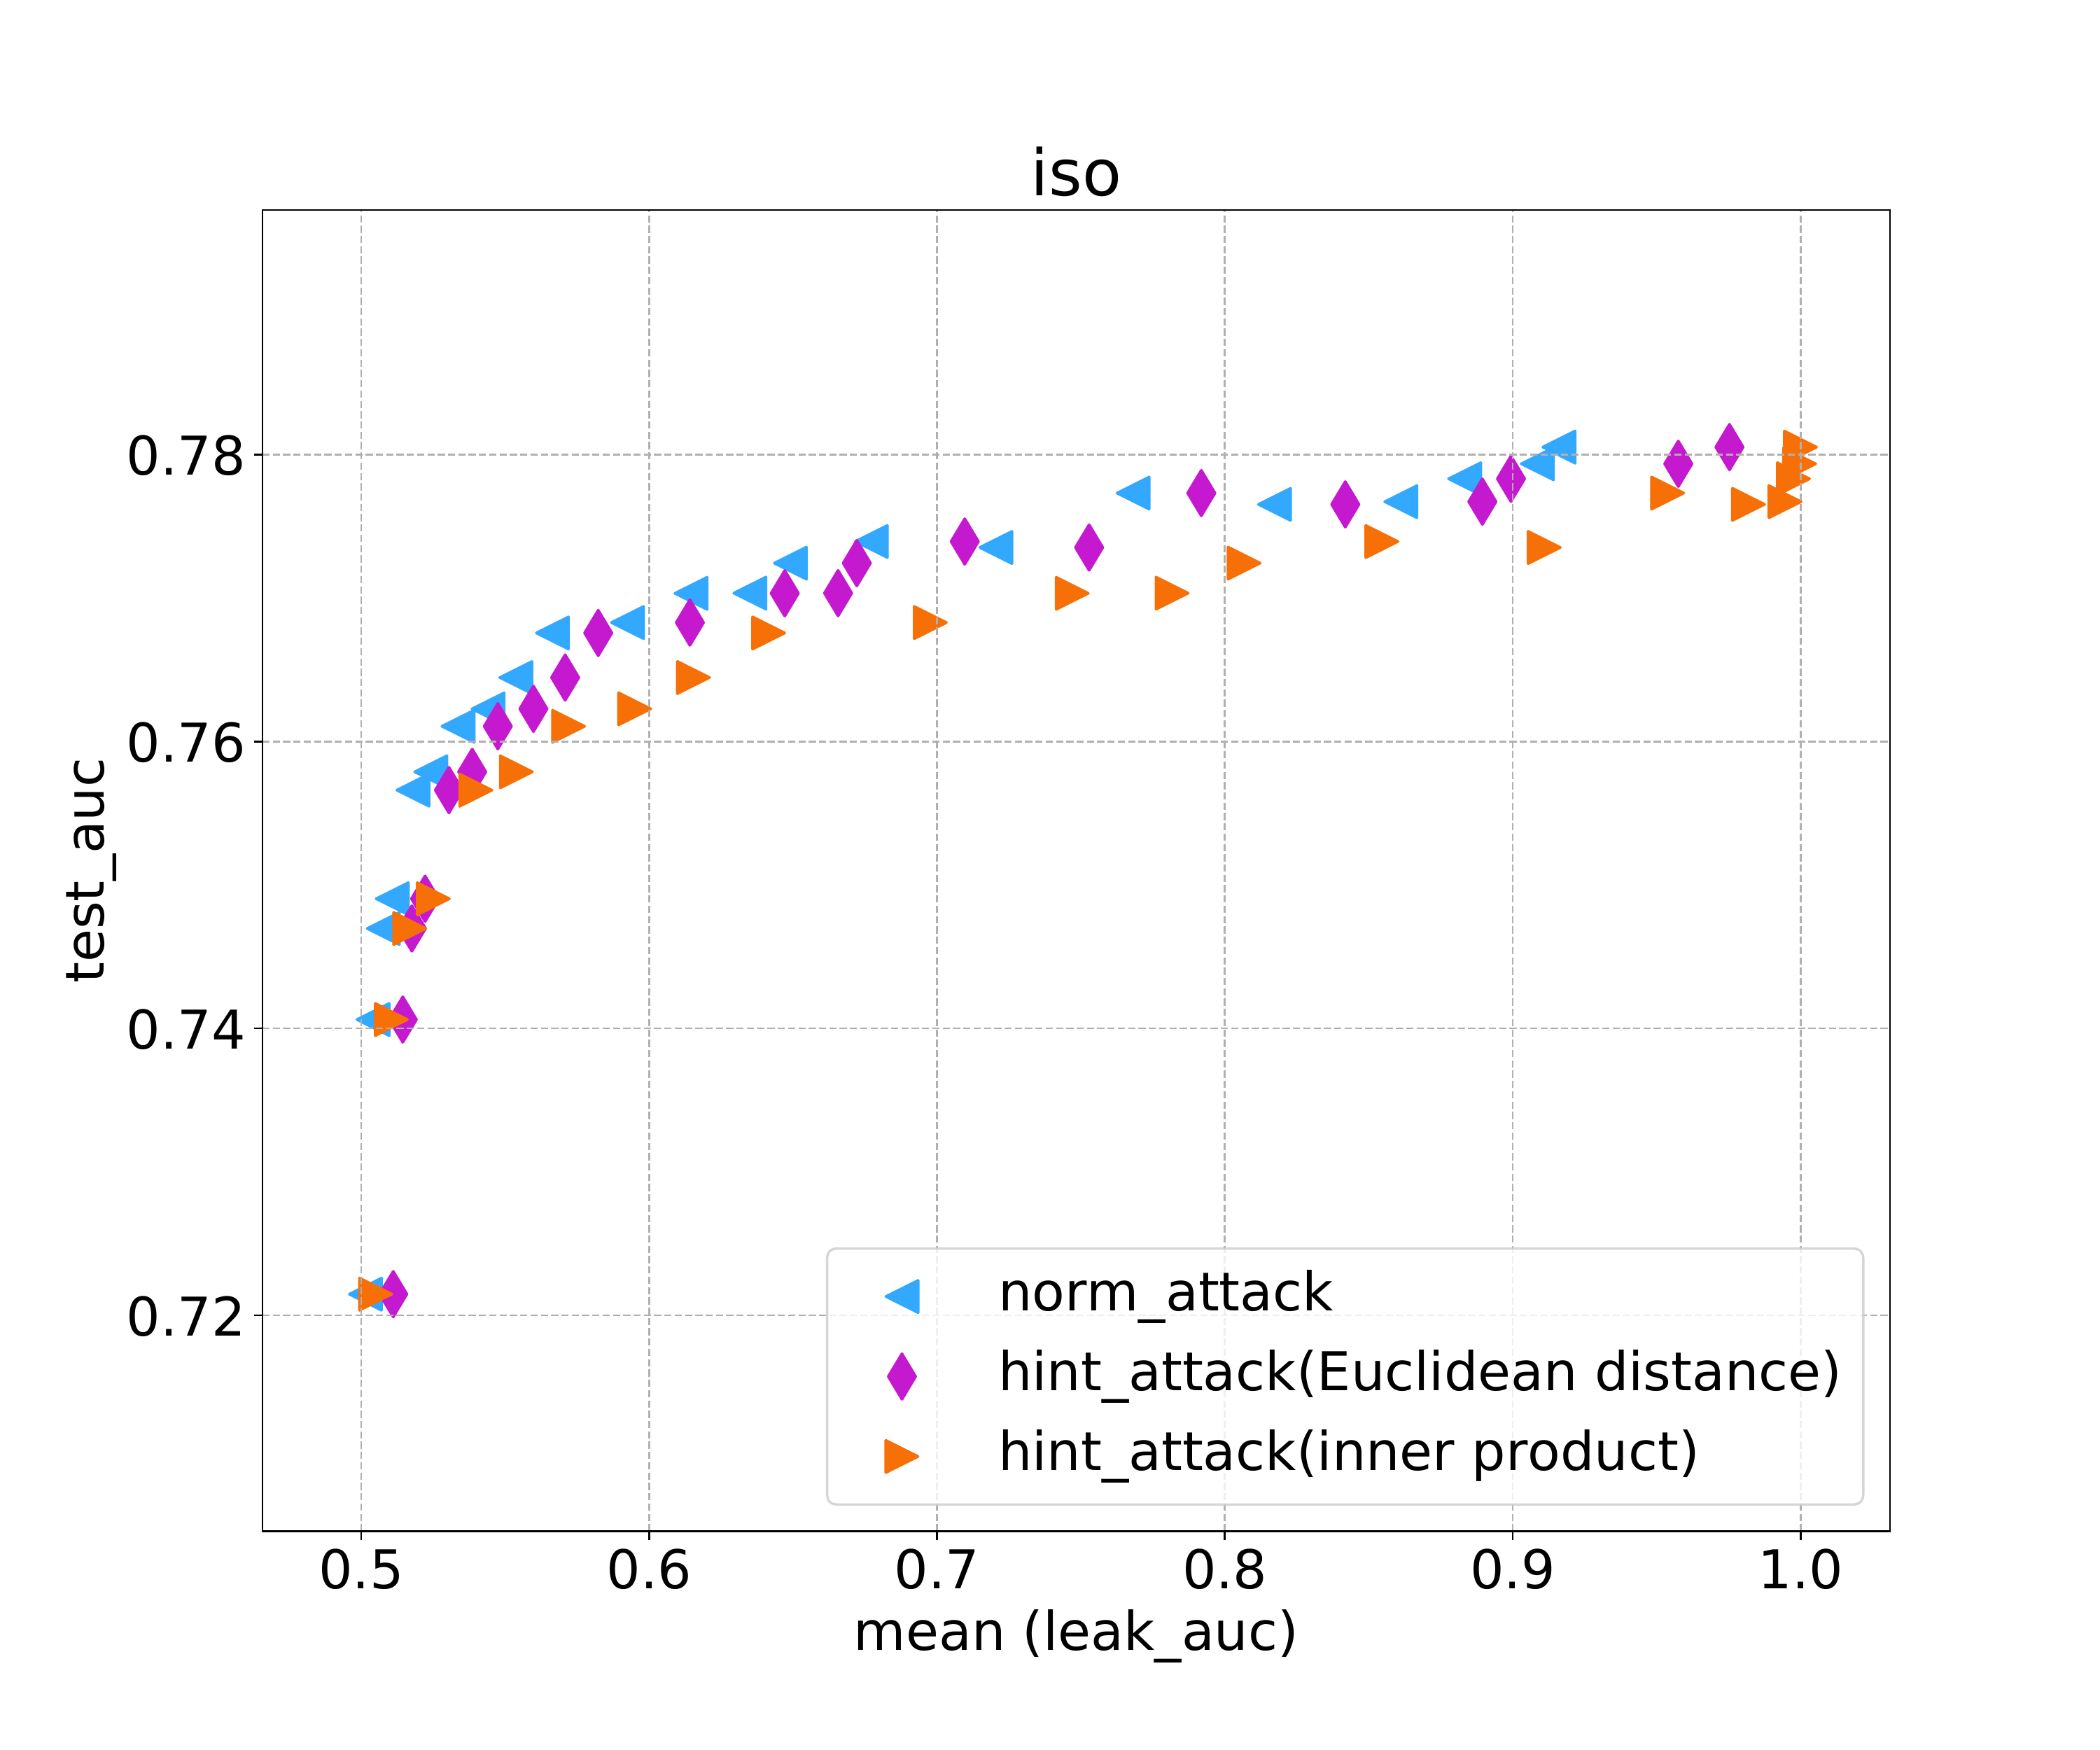}
    \caption*{(b: white_gaussian_against_different_attack_methods)}
  \end{minipage}
 \caption{Criteo: against different attack methods}
 \label{fig:criteo_aginst_different_attack_methods} 
\end{figure*}



\begin{figure*}[t]
  \begin{minipage}[b]{0.33\linewidth}
  \centering
    \includegraphics[width=\linewidth]{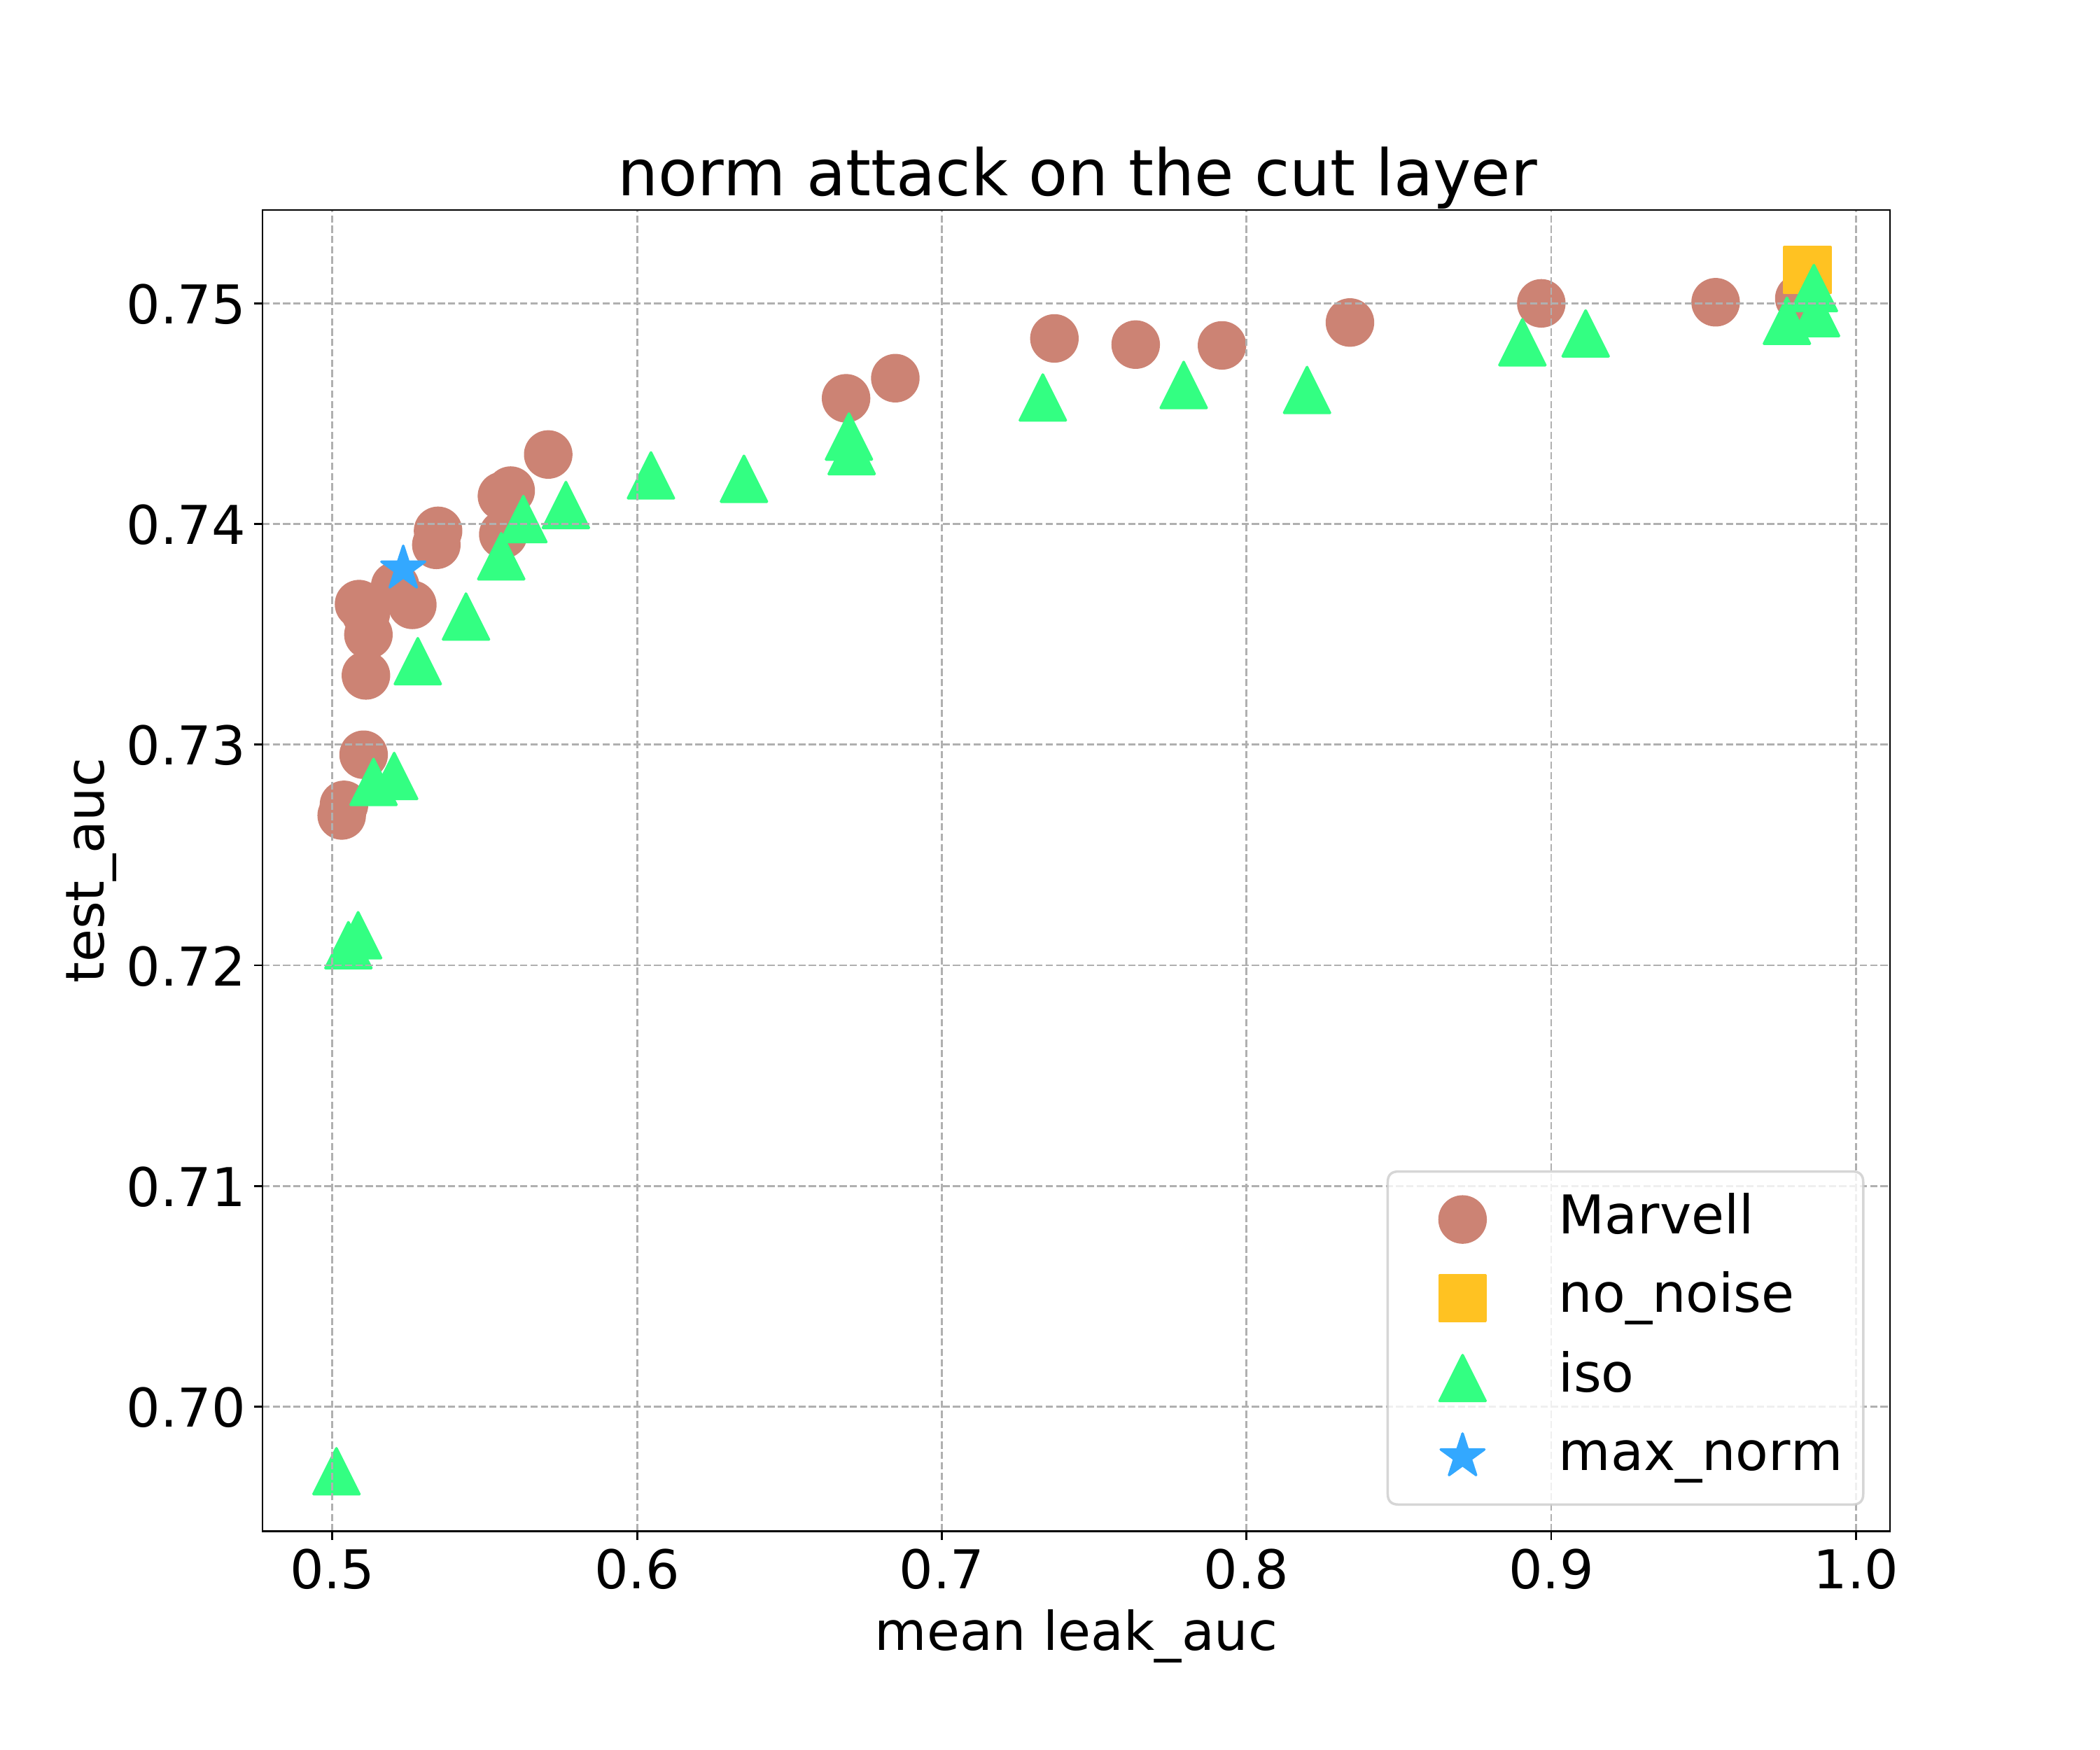}
      \caption*{ (a: )}
  \end{minipage}
  \begin{minipage}[b]{0.33\linewidth}
  \centering
    \includegraphics[width=\linewidth]{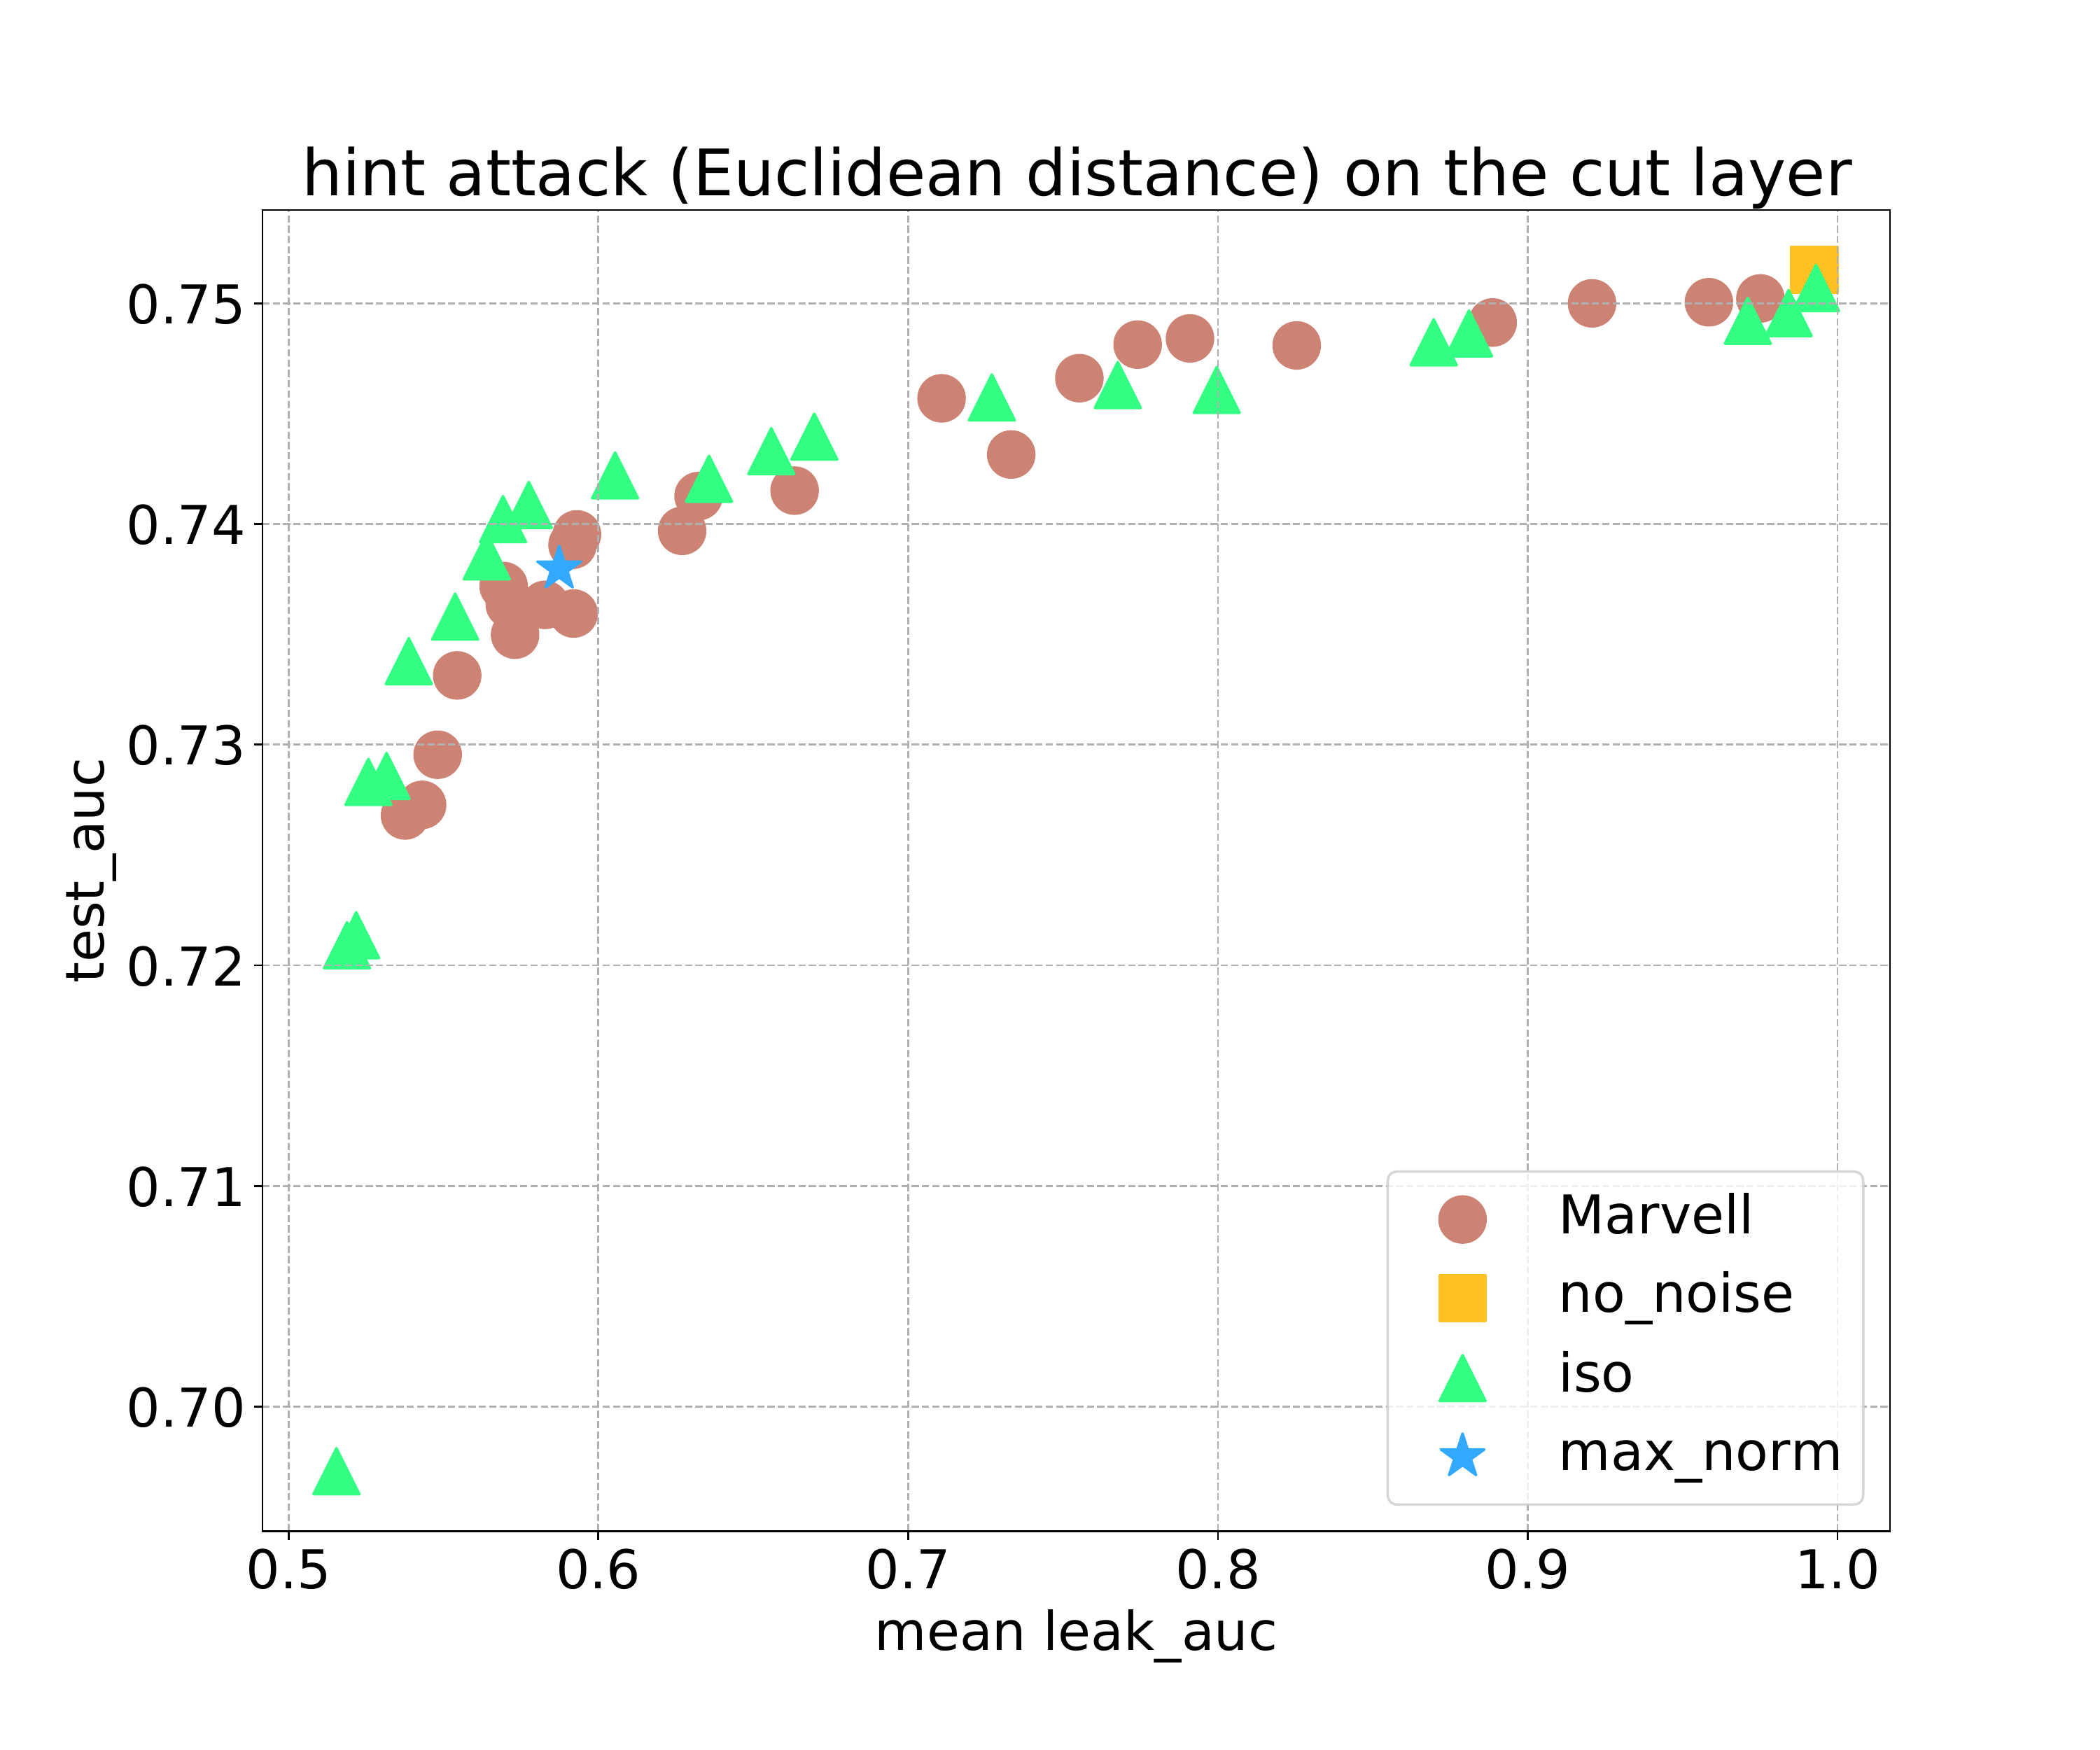}
    \caption*{(b: )}
  \end{minipage}
   \begin{minipage}[b]{0.33\linewidth}
  \centering
    \includegraphics[width=\linewidth]{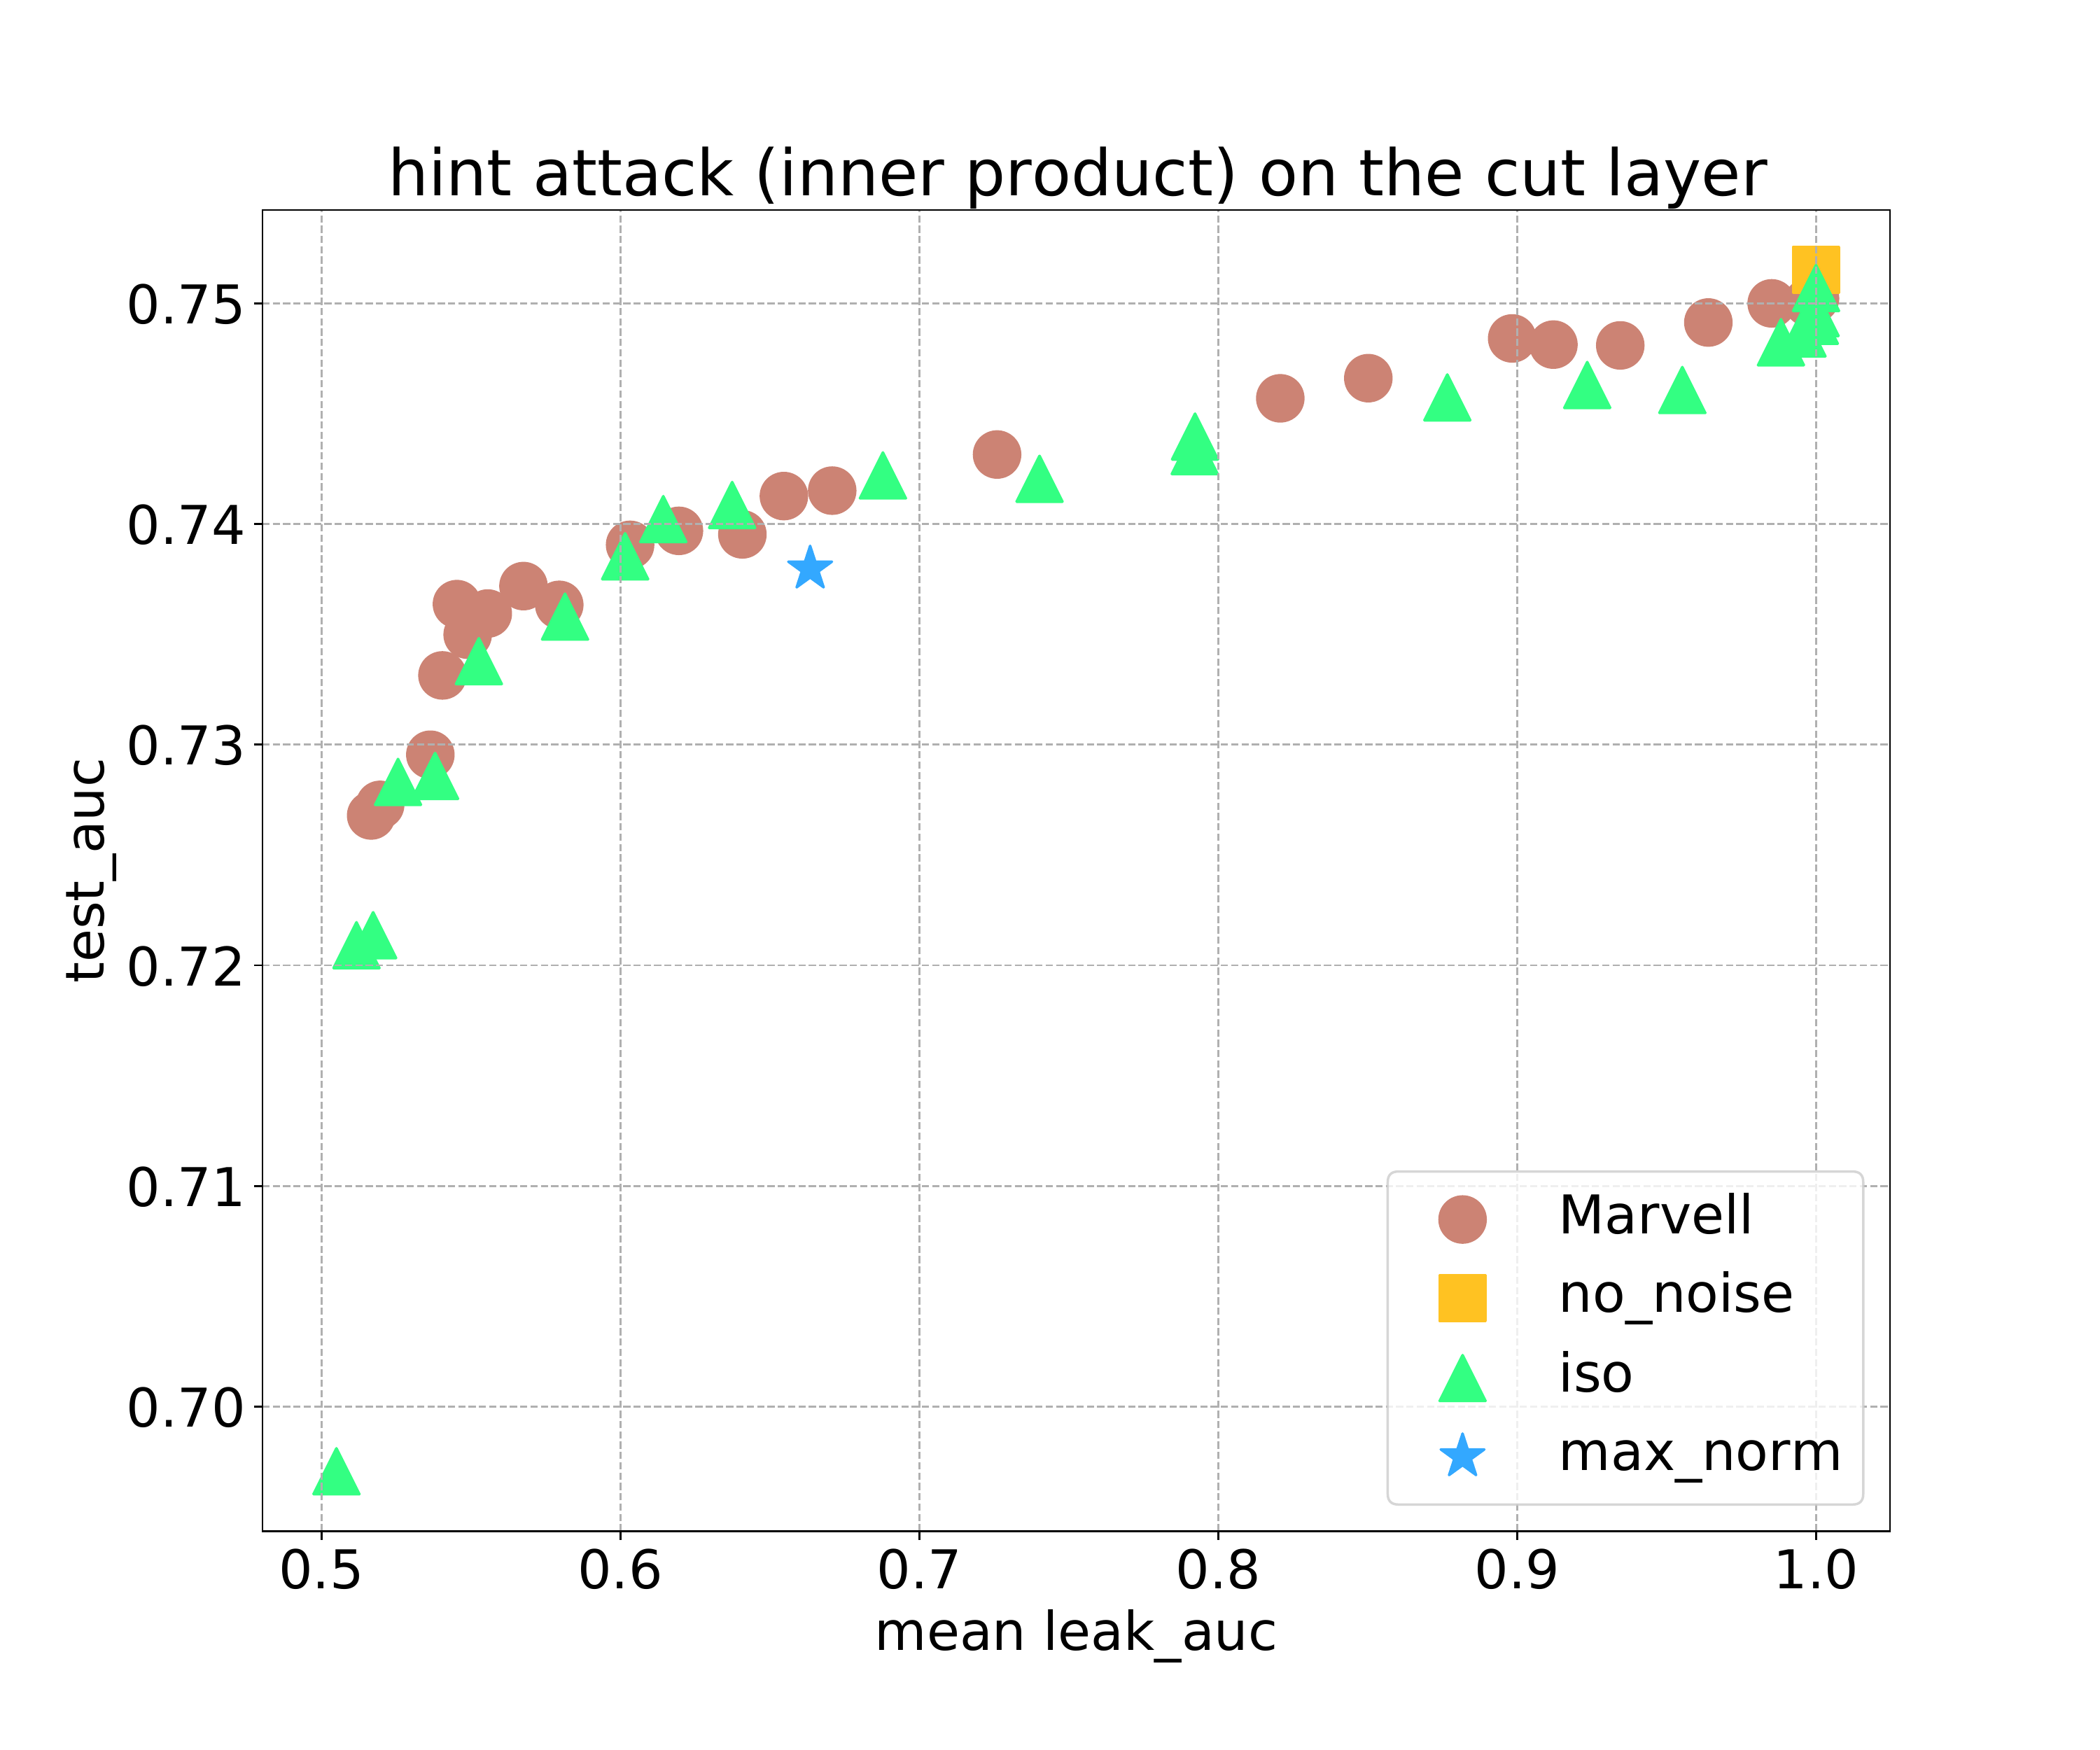}
      \caption*{ (c: )}
  \end{minipage}
 \vspace{-1.5em}
 \caption{Avazu: trade-off between test AUC and leak AUC. num hints = $5$.}
 \label{fig:avazu_tradeoff_test_auc_privacy} 
\end{figure*}



\begin{figure*}[t]
  \begin{minipage}[b]{0.33\linewidth}
  \centering
    \includegraphics[width=\linewidth]{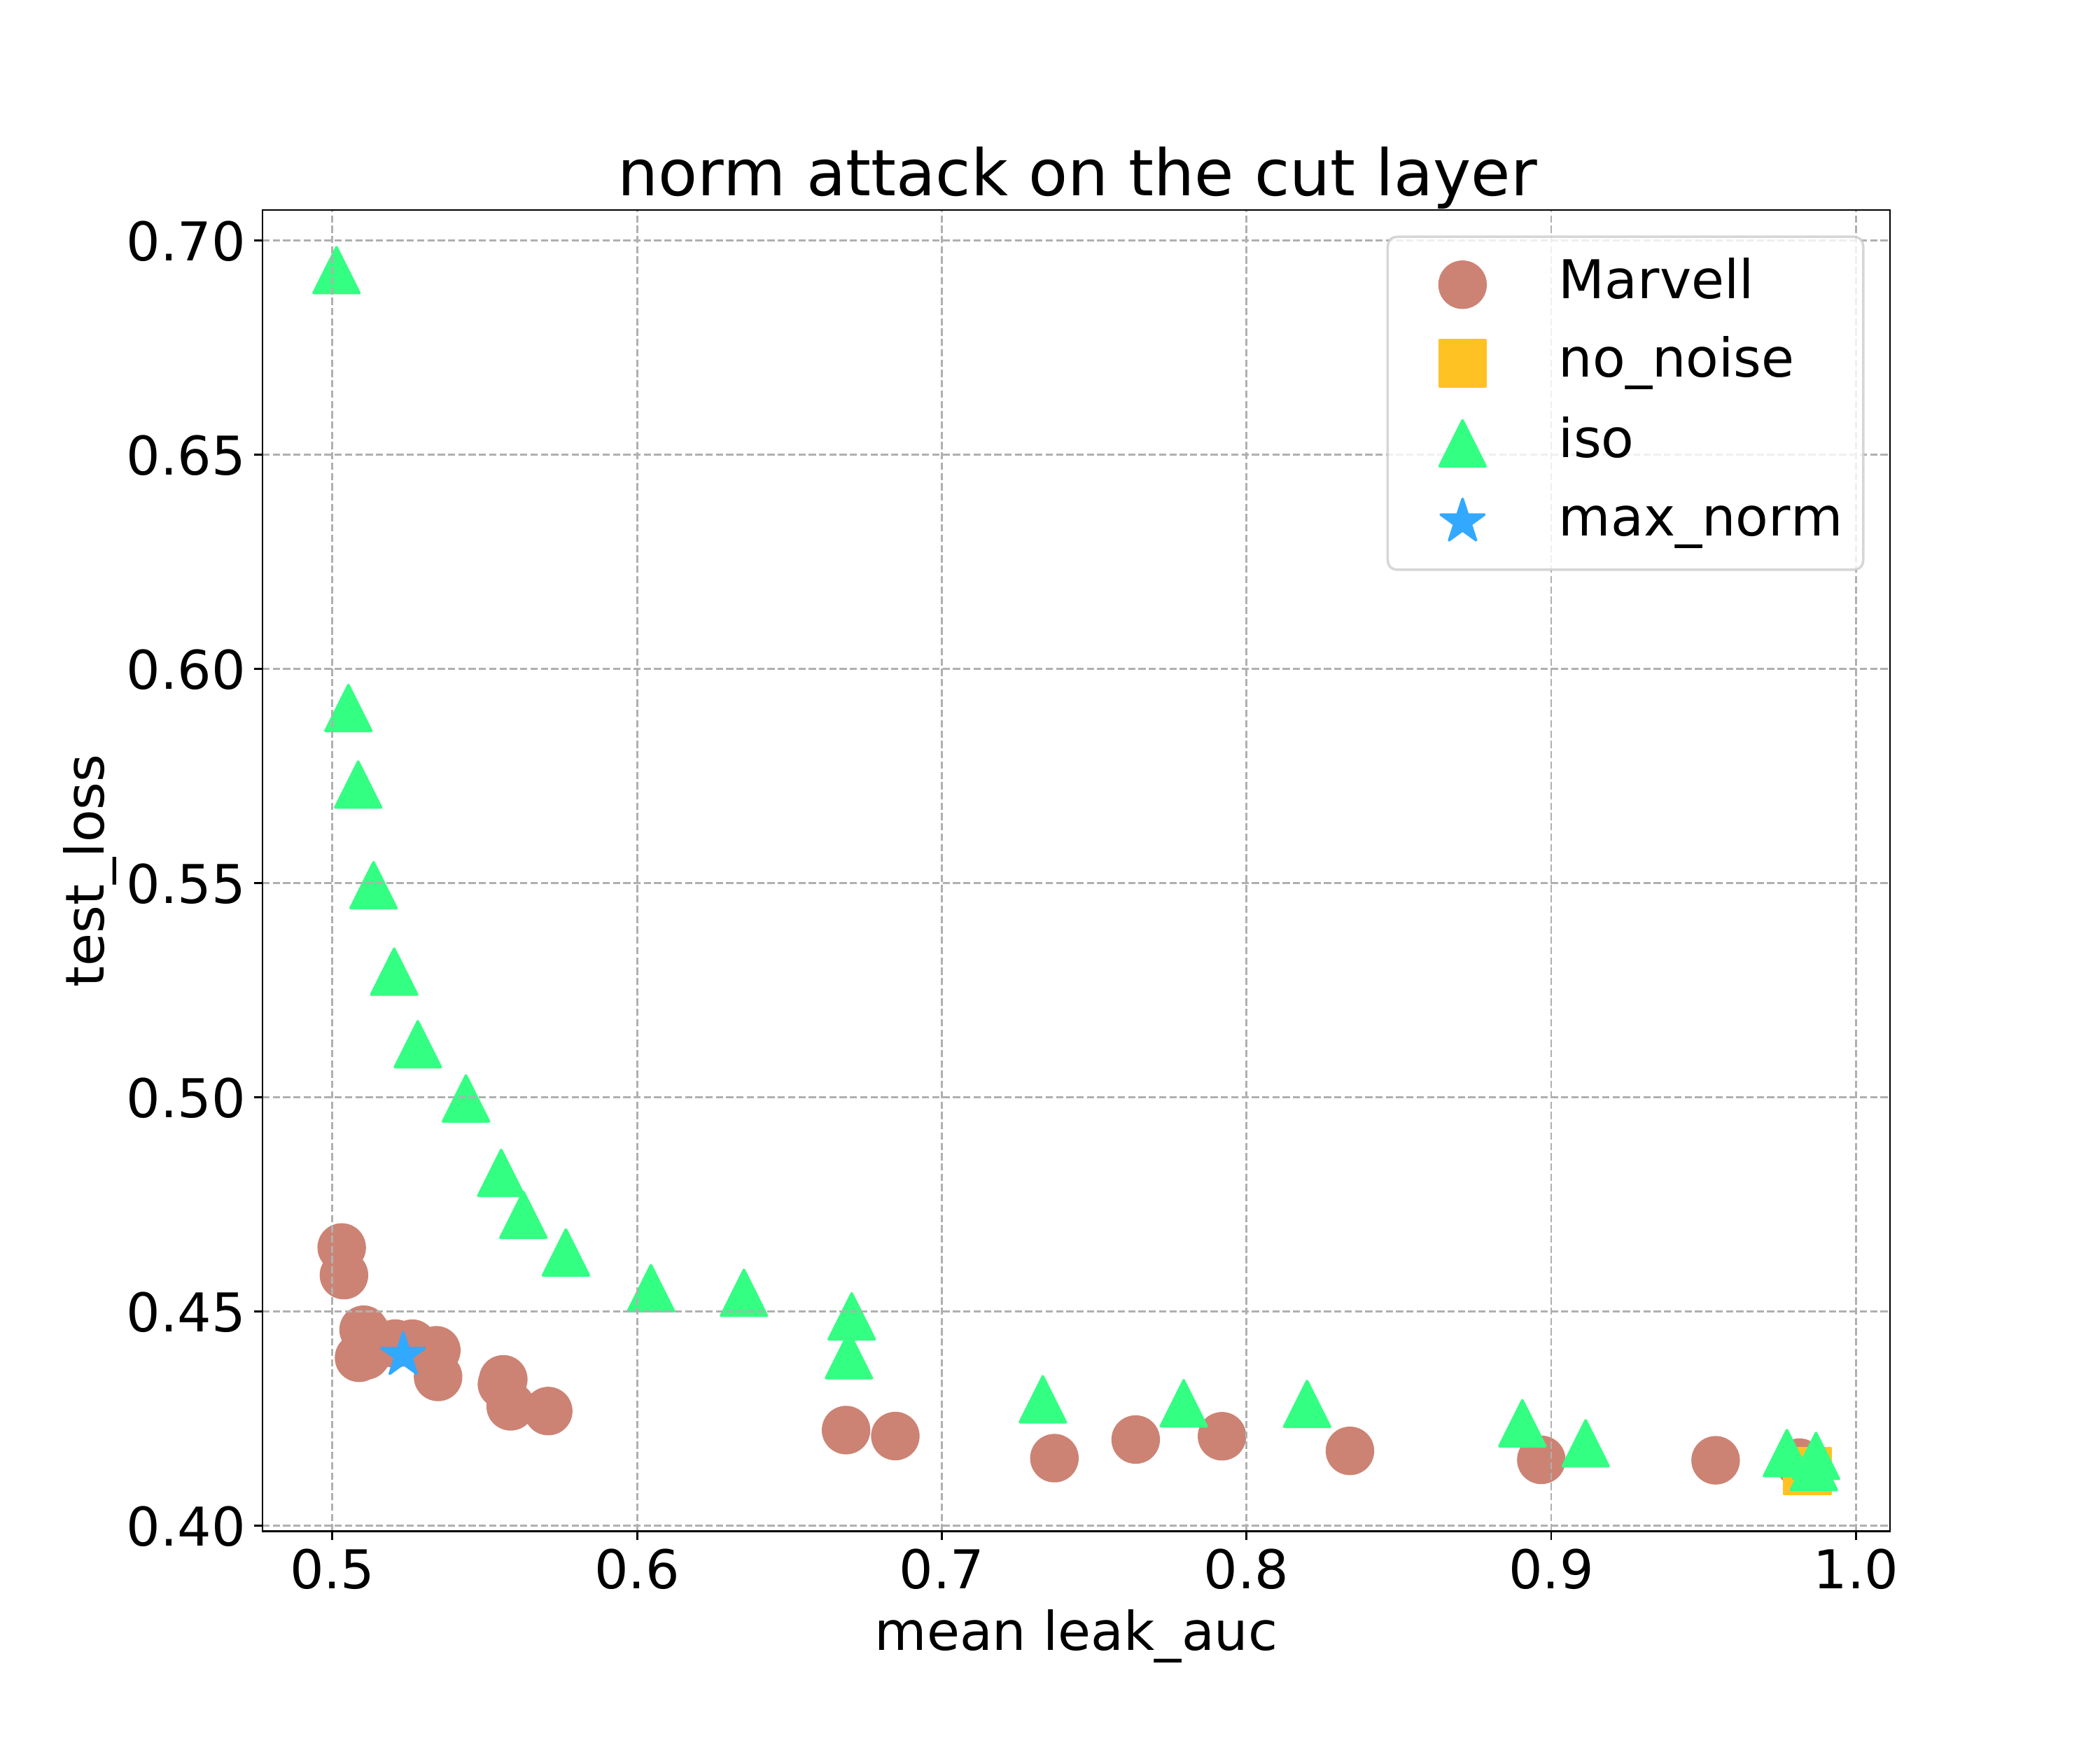}
      \caption*{ (a: )}
  \end{minipage}
  \begin{minipage}[b]{0.33\linewidth}
  \centering
    \includegraphics[width=\linewidth]{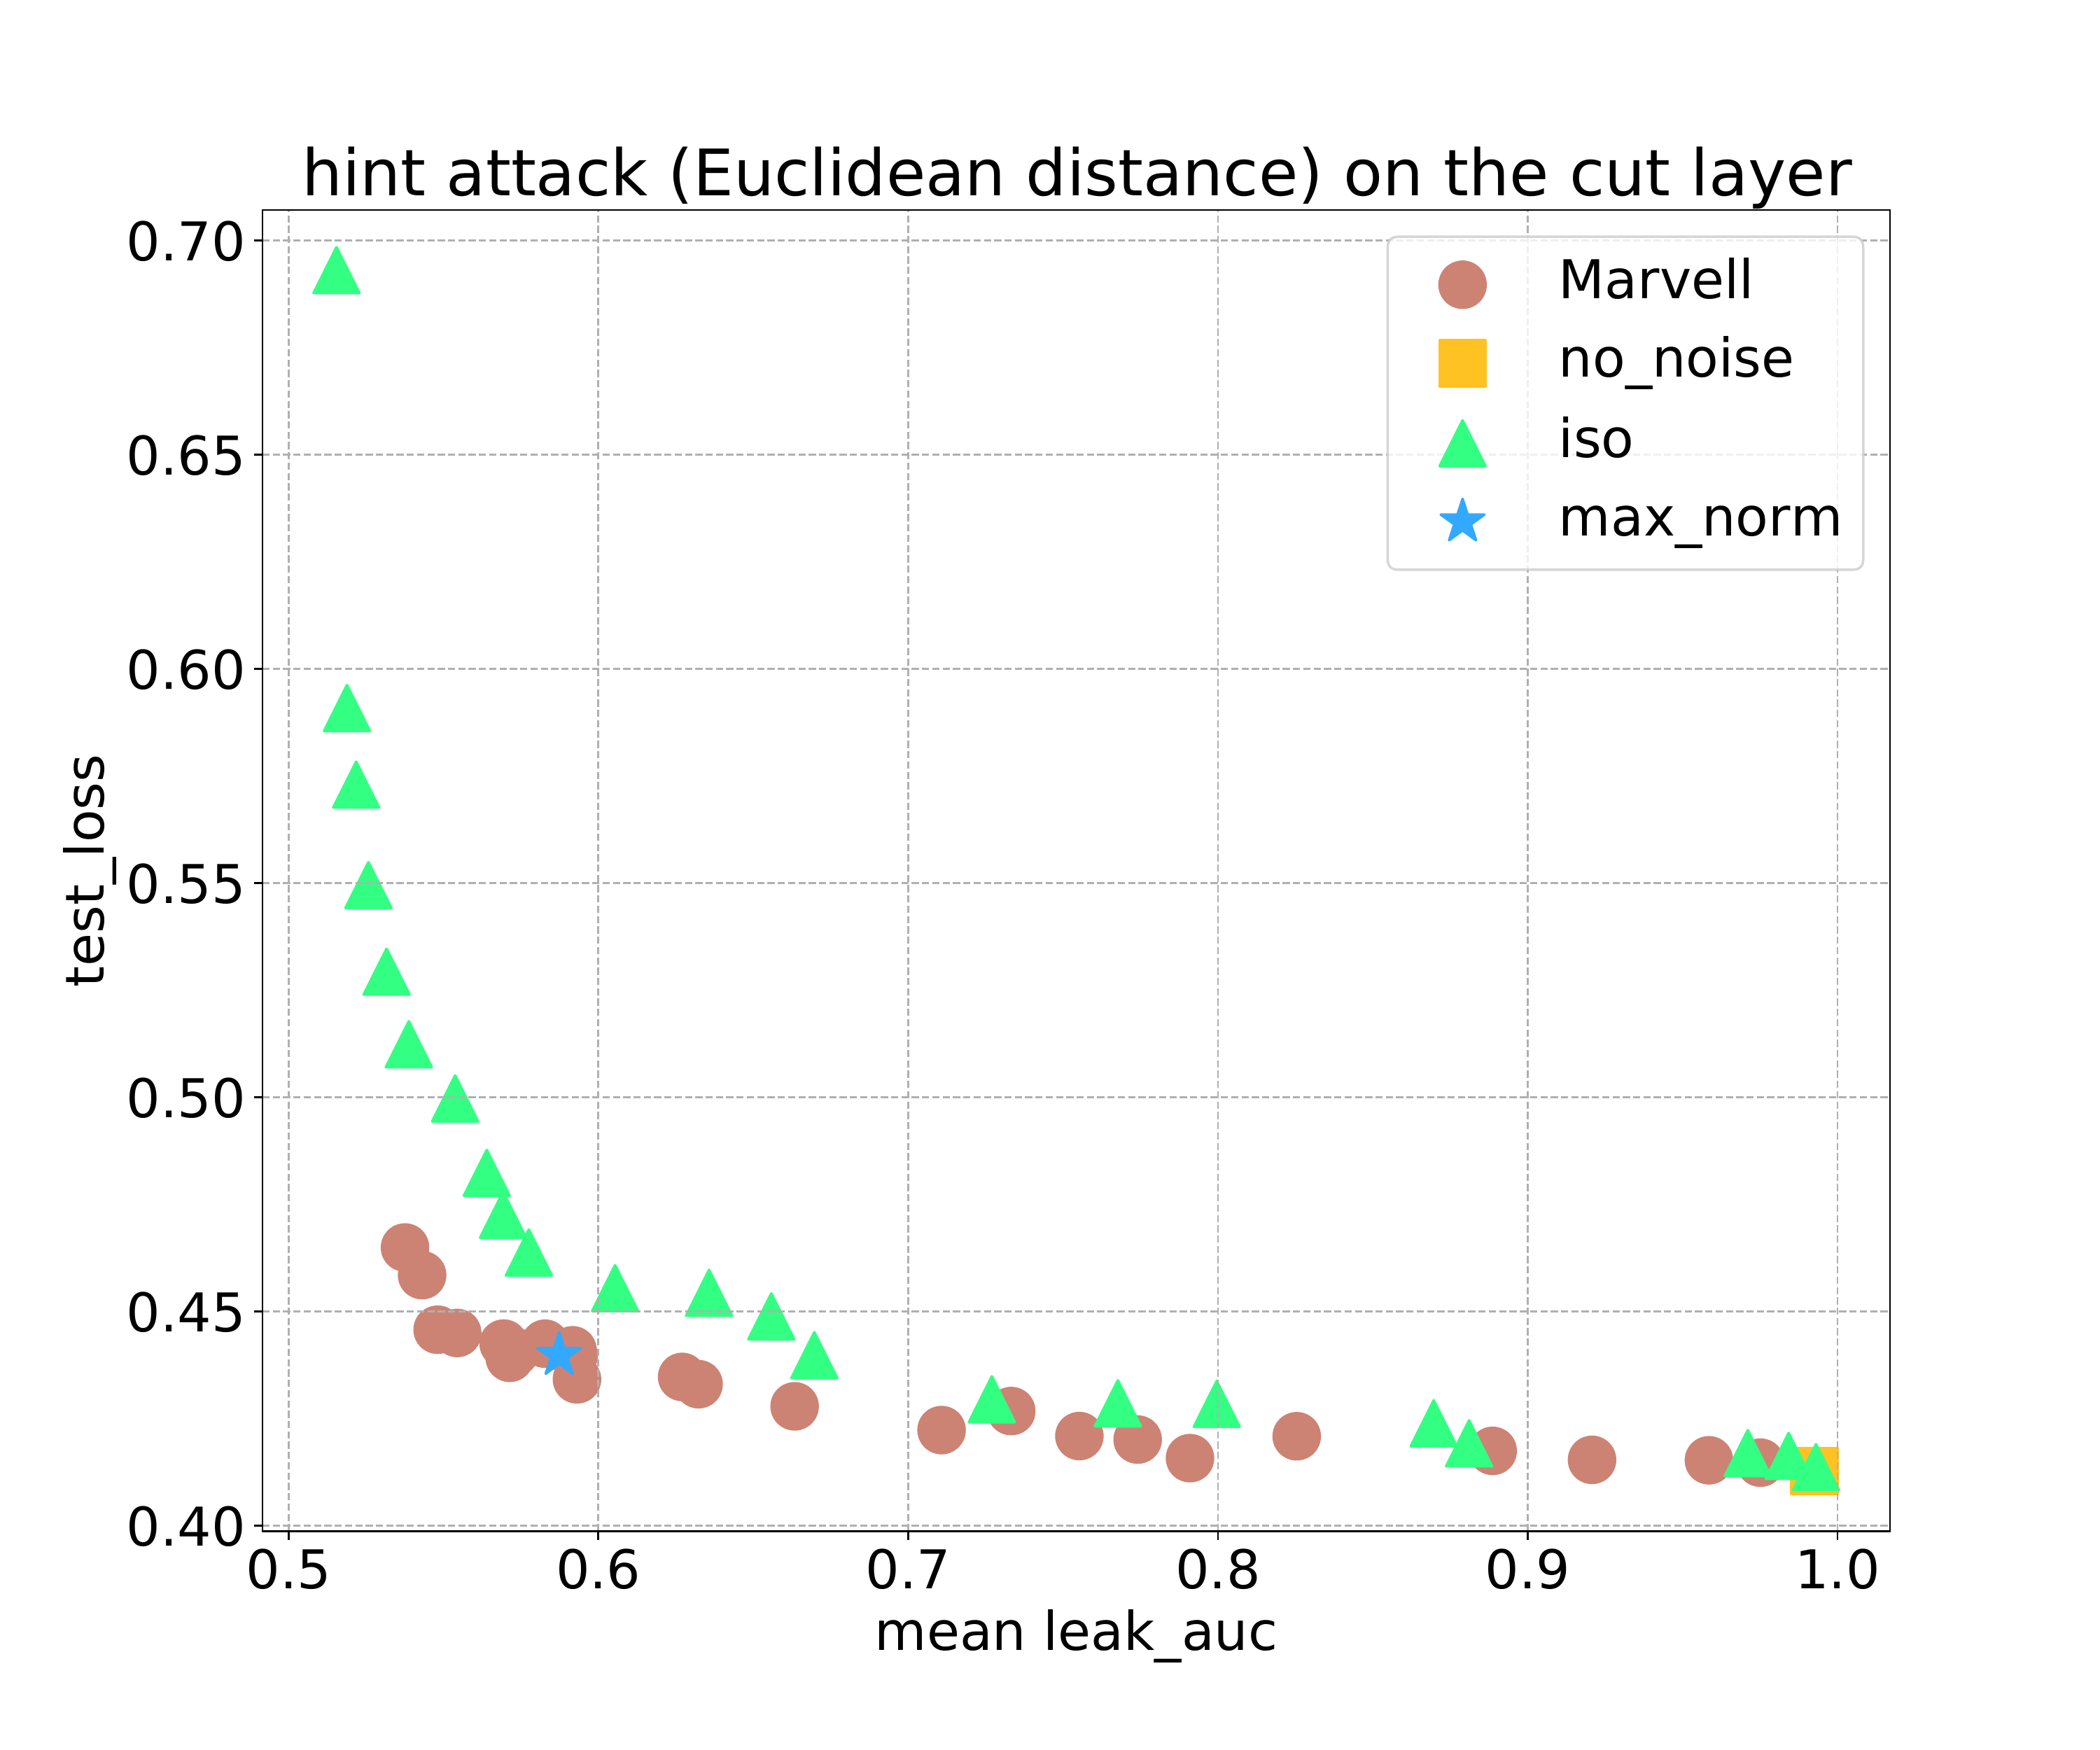}
    \caption*{(b: )}
  \end{minipage}
   \begin{minipage}[b]{0.33\linewidth}
  \centering
    \includegraphics[width=\linewidth]{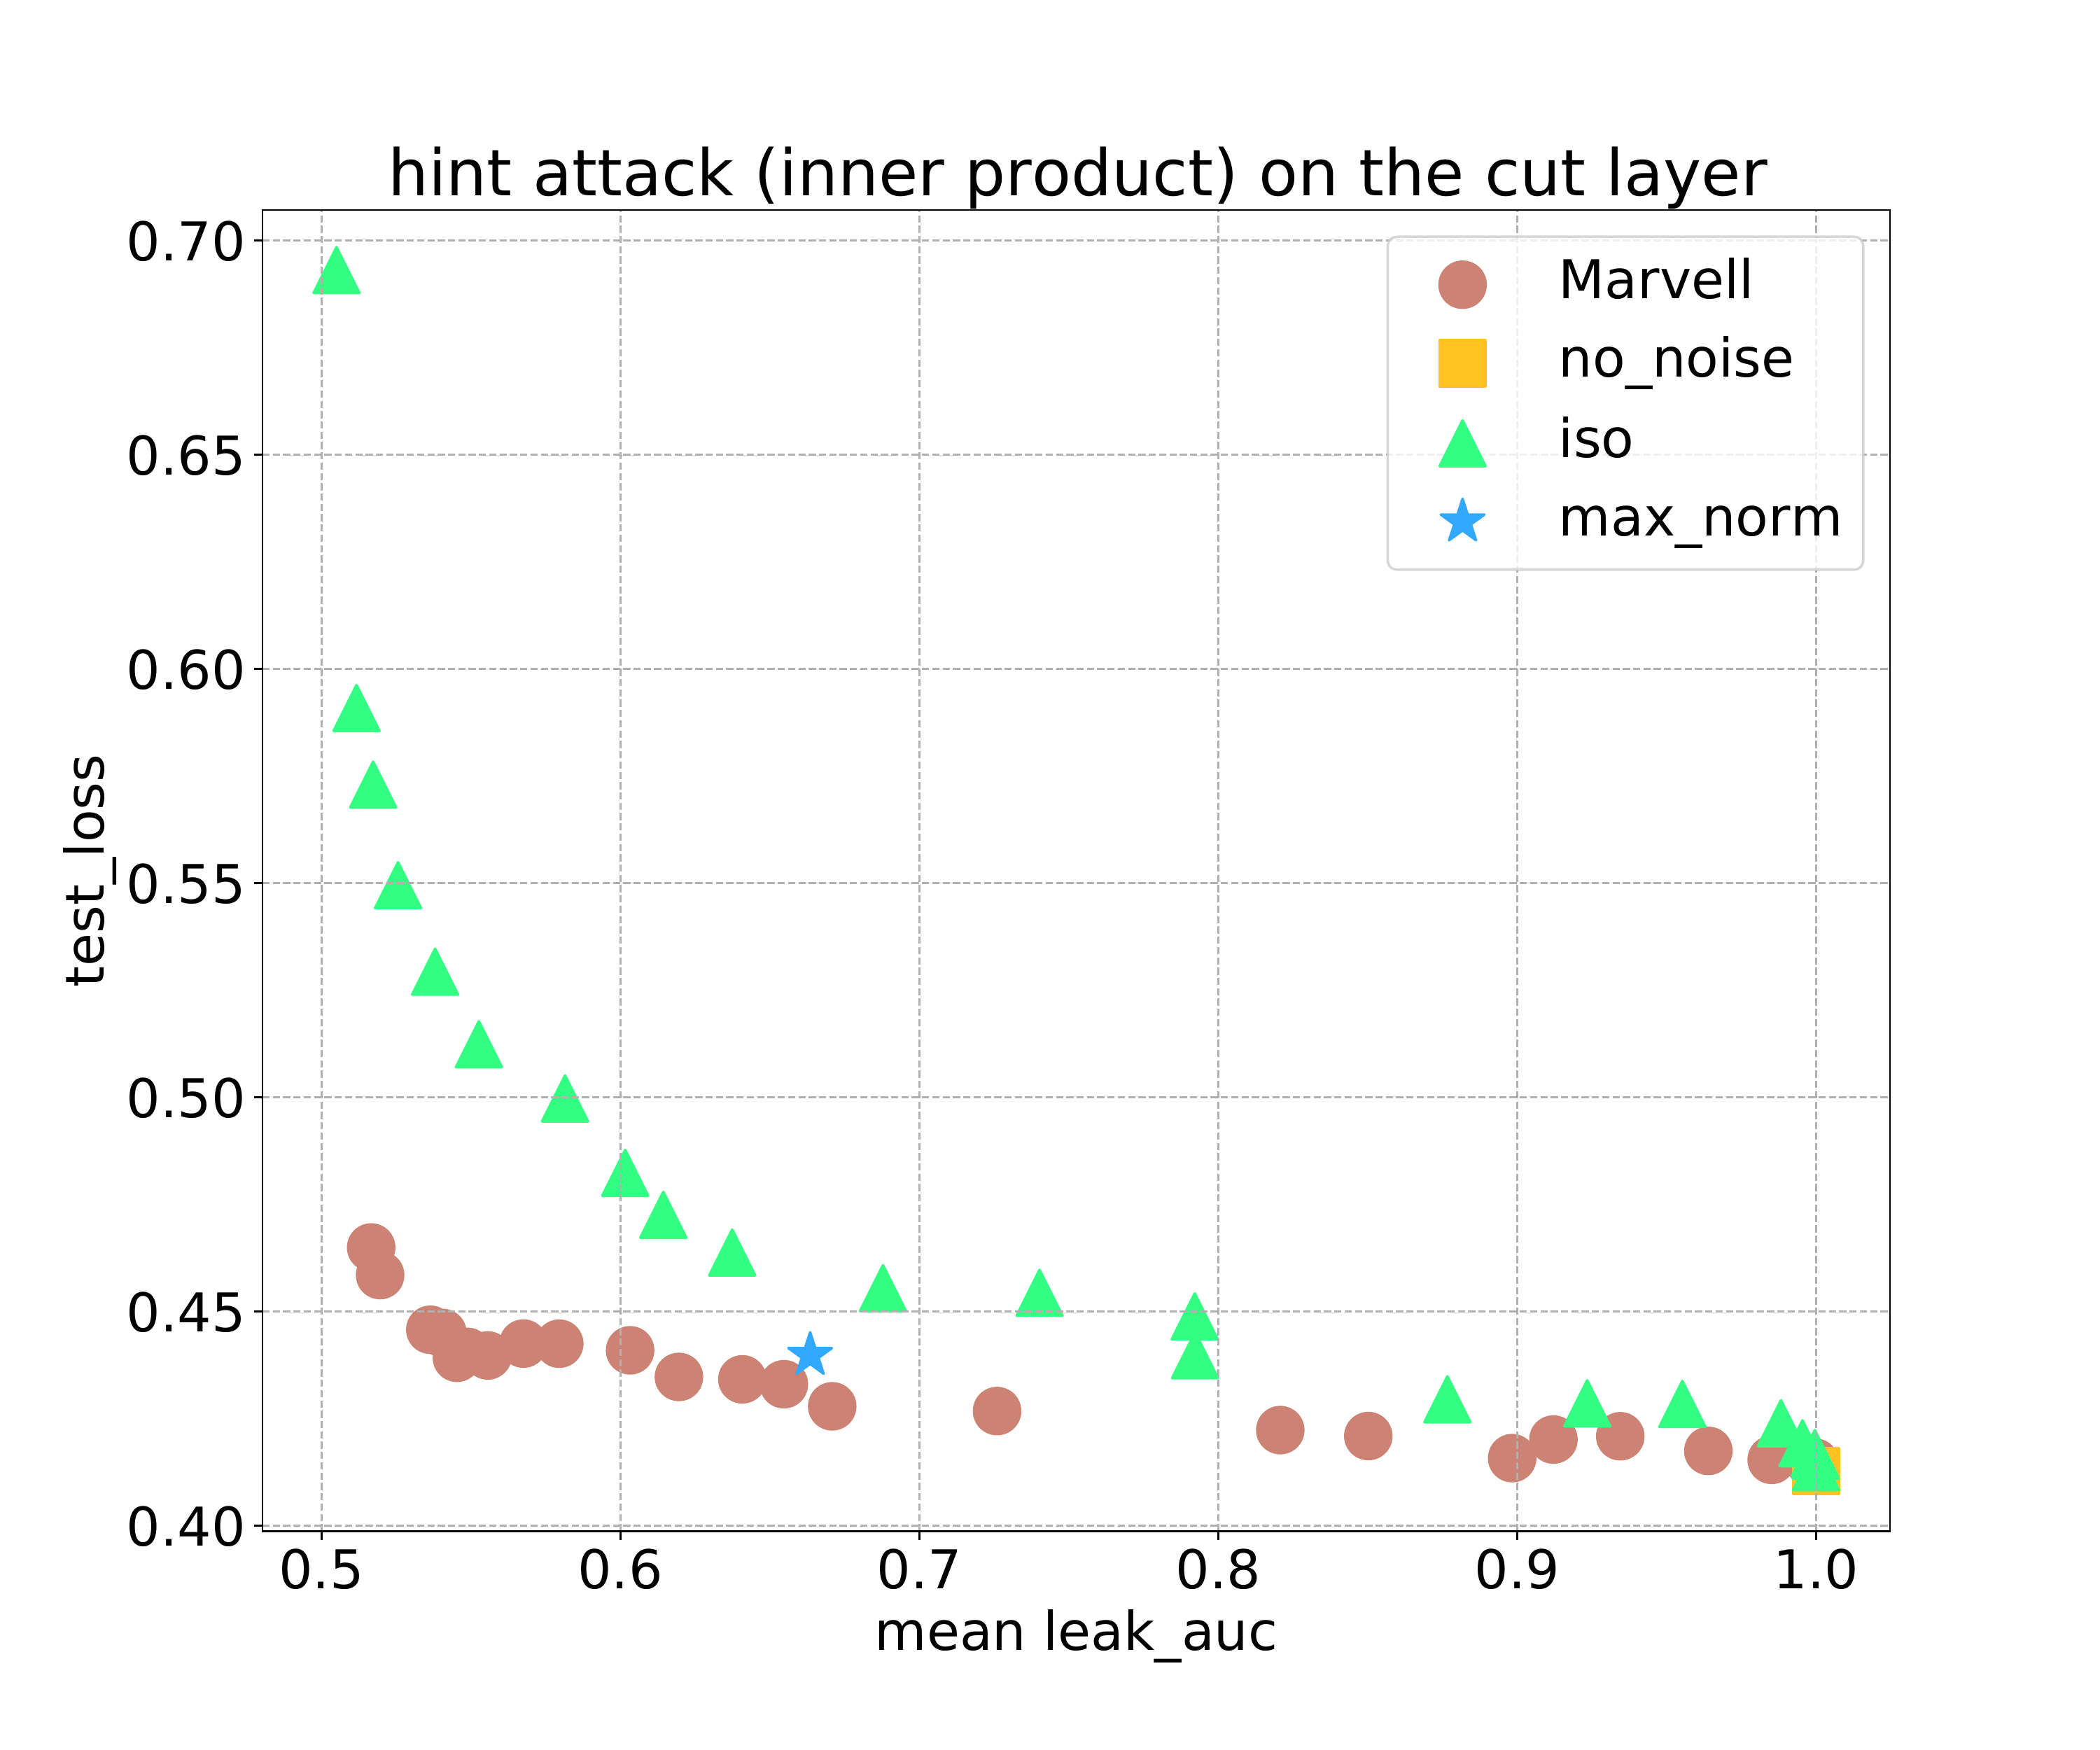}
      \caption*{ (c: )}
  \end{minipage}
 \vspace{-1.5em}
 \caption{Avazu: trade-off between test loss and leak AUC. num hints = $5$.}
 \label{fig:avazu_tradeoff_test_loss_privacy} 
\end{figure*}
