# Supplementary material for: Vertical Federated Learning without Revealing Intersection Membership
Source: arXiv:2106.05508 source file (2021-06-10)
Supplement: Supplementary file 2 [file appendix.tex]

\section*{Appendix}
% % \subsection*{Implementation details}
% \subsection*{A.1 \;\; Proof of theorem
% \subsection{Implementation Details}
% \ref{thm:optimal_solution}}

%\newcommand{\lam}[2]{\lambda_{#1}^{(#2)}}
%\newcommand{\Lam}[2]{\lambda_{#1}^{(#2)*}}
\newcommand{\aaa}[2]{a_{#1}^{(#2)}}
\begin{proof}[Proof of Theorem \ref{thm:optimal_solution}]
Based on the assumption made in Section \ref{sec: optimization}, the optimization problem we want to solve is:

\begin{align*}
    \min_{\Sigma_0, \Sigma_1 \in \Sym}& \KL{\calN(\bar{g}^{(1)}, uI + \Sigma_1)}{\calN(\bar{g}^{(0)}, vI + \Sigma_0)} +  \KL{\calN(\bar{g}^{(0)}, vI + \Sigma_0)}{\calN(\bar{g}^{(1)}, uI + \Sigma_1)} \\
     \subjectto &
\end{align*}
\begin{align*}
    \Sigma_0 \Sigma_1 =& \; \Sigma_1 \Sigma_0, \label{constraint2}\\
    p \cdot \tr(\Sigma_1) + (1-p)\cdot \tr(\Sigma_0) \le& \; P ,\\
    \Sigma_1 \succeq& \; \bzero ,\\
    \Sigma_0 \succeq& \; \bzero.
\end{align*}

By writing out the analytical close-form of the KL divergence between two Gaussian distributions, the optimization can be written as:
\begin{align*}
    &\min_{\Sigma_0, \Sigma_1 \in \Sym} \;  \tr((\Sigma_1+vI)^{-1}(\Sigma_0+uI))  + \tr((\Sigma_0+uI)^{-1}(\Sigma_1+vI))   + (\bar{g}^{(1)} - \bar{g}^{(0)})^{\top}\paren{(\Sigma_1+vI)^{-1} + (\Sigma_0+uI)^{-1}}(\bar{g}^{(1)} - \bar{g}^{(0)})\notag\\
     &\subjectto 
\end{align*}
\begin{equation}\label{constraint2}
    \begin{aligned}
        \Sigma_0 \Sigma_1 =& \; \Sigma_1 \Sigma_0, \\
    p \cdot \tr(\Sigma_1) + (1-p)\cdot \tr(\Sigma_0) \le& \;P, \\
    \Sigma_1 \succeq& \; \bzero, \\
    \Sigma_0 \succeq& \; \bzero.
    \end{aligned}
\end{equation}



By the commutative constraint on the two positive semidefinite matrices $\Sigma_1$ and $\Sigma_0$, we know that we can factor these two matrices using the same set of eigenvectors. We thus write:
\begin{align*}
    \Sigma_0 =& Q^{\top} \diag(\lambda_1^{(0)}, \ldots, \lambda_d^{(0)}) Q,\\
    \Sigma_1 =& Q^{\top} \diag(\lambda_1^{(1)}, \ldots, \lambda_d^{(1)}) Q,
\end{align*} where $Q \in \Real^{d \times d}$ is an orthogonal matrix and the eigenvalues $\lambda_i^{(0)}, \lambda_i^{(1)}$ are nonnegative and decreasing in value.

Using this alternative expression of $\Sigma_1$ and $\Sigma_0$, we can express the optimization in terms of $\{\lambda_i^{(1)}\}, \{\lambda_i^{(0)}\}, Q$:

\begin{align*}
    \min_{\{\lambda_i^{(1)}\}, \{\lambda_i^{(0)}\}, Q} & \sum_{i=1}^d \frac{\lambda_i^{(0)} + u}{\lambda_i^{(1)} + v} + \sum_{i=1}^d \frac{\lambda_i^{(1)} + v}{\lambda_i^{(0)} + u}  + \brck{Q(\bar{g}^{(1)} - \bar{g}^{(0)})}^{\top} \diag\paren{\ldots, \frac{1}{\lambda_i^{(0)} + u} + \frac{1}{\lambda_i^{(1)} + v}, \ldots} Q(\bar{g}^{(1)} - \bar{g}^{(0)})
\end{align*}
\begin{align*}
    \subjectto \quad &p(\sum_{i=1}^d \lambda_i^{(1)}) + (1-p)(\sum_{i=1}^d \lambda_i^{(0)}) \le \; P \\
    &- \lambda_i^{(1)} \le \; 0, \; \forall i \in [d]\\
    &- \lambda_i^{(0)} \le \; 0, \; \forall i \in [d].\\
    &\lam{i}{1} \ge  \lam{j}{1}, \forall i < j. \\
    &\lam{i}{0} \ge  \lam{j}{0}, \forall i < j. \\
    &Q \;\;  \textrm{orthogonal}.
\end{align*}

For any fixed feasible $\{\lambda_i^{(1)}\}, \{\lambda_i^{(0)}\}$, we see that the corresponding minimizing $Q$ will set its first row to be the unit vector in the direction of $\Delta g$. Thus by first minimizing $Q$, the optimization objective reduces to:
\begin{align*}
    &\sum_{i=1}^d \frac{\lambda_i^{(0)} + u}{\lambda_i^{(1)} + v} + \sum_{i=1}^d \frac{\lambda_i^{(1)} + v}{\lambda_1^{(0)} + u} +  \frac{g}{\lambda_1^{(0)} + u} + \frac{g}{\lambda_1^{(1)} + v} \nonumber \\
    =& \sum_{i=2}^d \frac{\lambda_i^{(0)} + u}{\lambda_i^{(1)} + v} + \sum_{i=2}^d \frac{\lambda_i^{(1)} + v}{\lambda_i^{(0)} + u} +  \frac{\lambda_1^{(1)} + v + \norm{\Delta g}_2^2}{\lambda_1^{(0)} + u} + \frac{ \lambda_1^{(0)} + u + \norm{\Delta g}_2^2}{\lambda_1^{(1)} + v} \label{objective1}.
\end{align*}
We see that for the pair of variable $(\lam{i}{1}, \lam{i}{0})$ the function $\frac{\lambda_i^{(0)} + u}{\lambda_i^{(1)} + v} + \frac{\lambda_i^{(1)} + v}{\lambda_1^{(0)} + u}$ is strictly convex over the line segment $p\lam{i}{1} + (1-p)\lam{i}{0} =c $ for any positive $c$ and attains the the minimum value at $\lam{i}{1} = 0$ when $v < u$ and $\lam{i}{0} = 0$ when $v \ge u$. Suppose without loss of generality $u < v$, then for the optimal solution we must have 
$\lam{i}{0}=0$ for all $i$. Under this condition, we notice that the function $x \mapsto \frac{u}{x+v} + \frac{x+v}{u}$ is strictly convex on the positive reals. Thus by Jensen inequality, the optimal solution's variables $\lam{i}{1}$ must take on the same value for all $i$. As a result, we have proved that at the optimal solution, we must have:
\begin{align*}
    \lambda_i^{(0)}=\lambda_j^{(0)} \textrm{ and } \lambda_i^{(1)}=\lambda_j^{(1)}, \textrm{ for } i, j \ge 2.
\end{align*}

Hence, we have the equivalent optimization problem:
\begin{equation}\label{objective2}
    \begin{aligned}
    \min_{\lambda_1^{(0)}, \lambda_1^{(1)}, \lambda_2^{(0)}, \lambda_2^{(1)}}& \; (d-1) \frac{\lambda_2^{(0)} + u}{\lambda_2^{(1)} + v} + (d-1) \frac{\lambda_2^{(1)} + v}{\lambda_2^{(0)} + u} + \frac{\lambda_1^{(0)} + u + \norm{\Delta g}_2^2}{\lambda_1^{(1)} + v} + \frac{ \lambda_1^{(1)} + v + \norm{\Delta g}_2^2}{\lambda_1^{(0)} + u} \\
    \subjectto &  \\
    & p \lambda_1^{(1)} + p(d-1) \lambda_2^{(1)}+ (1-p) \lambda_1^{(0)}+ (1-p)(d-1)(\lambda_2^{(0)}) \le \; P \\
    & \tenquad - \lambda_1^{(1)} \le \; 0  \\
    & \tenquad - \lambda_1^{(0)} \le \; 0  \\
    & \tenquad - \lambda_2^{(1)} \le \; 0  \\
    & \tenquad - \lambda_2^{(0)} \le \; 0  \\
    & \tenquad \lambda_2^{(1)} - \lambda_1^{(1)} \le \; 0 \\
    & \tenquad \lambda_2^{(0)} - \lambda_1^{(0)} \le \; 0 .
\end{aligned}
\end{equation}

Given the optimal solution to the above 4-variable problem $(\Lam{1}{0}, \Lam{2}{0}, \Lam{1}{1}, \Lam{2}{1})$, we can set $Q$ to be any orthogonal matrix whose first row is the vector $\frac{\Delta g}{\norm{\Delta g}_2}$. Plugging this back into the expression of $\Sigma_1$ and $\Sigma_0$ gives us the final result.

Thus the proof is complete.
\end{proof}
\bigskip

\remark{} By analyzing the KKT condition of this four variable problem we can find that the optimal solution must occur on the hyperplane $p \lambda_1^{(1)} + p(d-1) \lambda_2^{(1)}+ (1-p) \lambda_1^{(0)}+ (1-p)(d-1)\lambda_2^{(0)} = P$. Knowing from the proof above that in addition $\lam{2}{1} = 0$ if $u \ge v$ and $\lam{2}{0} = 0$ if $u < v$ further reduces this problem to a 3-variable problem. Keeping one of them fixed and optimizing the other two reduces the problem to a line search over a convex objective. Alternatingly fixing one of these three variables while optimizing the other two would eventually converge and give us the optimal solution.



% \subsection{Implementation Details}

% % \begin{equation}\label{eq1}
% %   \begin{gathered}
% %     x_1 = 1, x_2 = 1        \\
% %     h(x) = f(-20 + 15 + 17) \\
% %     h(x) = f(12) \approx 1   % no "\\" needed here
% %   \end{gathered}
% % \end{equation}
% In this section, we discuss the implementation details of optimizing the objective. Based on the assumption made in Section \ref{sec: optimization}, the optimization problem we want to solve is:

% \begin{equation}\label{eq1}
%   \begin{gathered}
%       \min_{\Sigma_0, \Sigma_1 \in \Sym} \KL{\calN(\bar{g}^{(1)}, uI + \Sigma_1)}{\calN(\bar{g}^{(0)}, vI + \Sigma_0)} +  \\ \KL{\calN(\bar{g}^{(0)}, vI + \Sigma_0)}{\calN(\bar{g}^{(1)}, uI + \Sigma_1)} \\
%   \end{gathered}
% \end{equation}
% subject to 
% % \begin{align*}
% %     \Sigma_0 \Sigma_1 =& \; \Sigma_1 \Sigma_0 \label{constraint2}\\
% %     p \cdot \tr(\Sigma_1) + (1-p)\cdot \tr(\Sigma_0) \le& \; P \\
% %     \Sigma_1 \succeq& \; \bzero \\
% %     \Sigma_0 \succeq& \; \bzero.
% % \end{align*}


% % \begin{equation}\label{constraint2}
% %     \begin{aligned}
% %         \Sigma_0 \Sigma_1 =& \; \Sigma_1 \Sigma_0 \\
% %     p \cdot \tr(\Sigma_1) + (1-p)\cdot \tr(\Sigma_0) \le& \; P \\
% %     \Sigma_1 \succeq& \; \bzero \\
% %     \Sigma_0 \succeq& \; \bzero.
% %     \end{aligned}
% % \end{equation}

% \begin{equation}\label{constraint2}
%     \begin{aligned}
%         \Sigma_0 \Sigma_1 =& \; \Sigma_1 \Sigma_0 \\
%     p \cdot \tr(\Sigma_1) + (1-p)\cdot \tr(\Sigma_0) \le& \; P \\
%     \Sigma_1 \succeq& \; \bzero \\
%     \Sigma_0 \succeq& \; \bzero.
%     \end{aligned}
% \end{equation}

% % \begin{align*}
% %     \min_{\Sigma_0, \Sigma_1 \in \Sym}& \KL{\calN(\bar{g}^{(1)}, uI + \Sigma_1)}{\calN(\bar{g}^{(0)}, vI + \Sigma_0)} +  \\ \KL{\calN(\bar{g}^{(0)}, vI + \Sigma_0)}{\calN(\bar{g}^{(1)}, uI + \Sigma_1)} \\
% %      \subjectto &
% % \end{align*}
% % \begin{align*}
% %     \Sigma_0 \Sigma_1 =& \; \Sigma_1 \Sigma_0 \label{constraint2}\\
% %     p \cdot \tr(\Sigma_1) + (1-p)\cdot \tr(\Sigma_0) \le& \; P \\
% %     \Sigma_1 \succeq& \; \bzero \\
% %     \Sigma_0 \succeq& \; \bzero.
% % \end{align*}

% By writing out the analytical close-form of the KL divergence between two Gaussian distributions, the optimization can be written as:
% \begin{align*}
%     &\min_{\Sigma_0, \Sigma_1 \in \Sym} \;  \tr((\Sigma_1+vI)^{-1}(\Sigma_0+uI)) + \tr((\Sigma_0+uI)^{-1}(\Sigma_1+vI)) \\ & \quad  + (\bar{g}^{(1)} - \bar{g}^{(0)})^{\top}\paren{(\Sigma_1+vI)^{-1} + (\Sigma_0+uI)^{-1}}(\bar{g}^{(1)} - \bar{g}^{(0)})\notag\\
%     %  &\subjectto 
% \end{align*}
% subject to the same constraints defined in Equation \ref{constraint2}.

% % \begin{equation}\label{constraint2}
% %     \begin{aligned}
% %         \Sigma_0 \Sigma_1 =& \; \Sigma_1 \Sigma_0 \\
% %     p \cdot \tr(\Sigma_1) + (1-p)\cdot \tr(\Sigma_0) \le& \; P \\
% %     \Sigma_1 \succeq& \; \bzero \\
% %     \Sigma_0 \succeq& \; \bzero.
% %     \end{aligned}
% % \end{equation}

% By the commutative constraint on the two positive semidefinite matrices $\Sigma_1$ and $\Sigma_0$, we know that we can factor these two matrices using the same set of eigenvectors. We thus write:
% \begin{align*}
%     \Sigma_0 =& Q^{\top} \diag(\lambda_1^{(0)}, \ldots, \lambda_d^{(0)}) Q\\
%     \Sigma_1 =& Q^{\top} \diag(\lambda_1^{(1)}, \ldots, \lambda_d^{(1)}) Q,
% \end{align*} where $Q \in \Real^{d \times d}$ is an orthogonal matrix and the eigenvalues $\lambda_i^{(0)}, \lambda_i^{(1)}$ are non-negative and decreasing in value.

% Using this alternative expression of $\Sigma_1$ and $\Sigma_0$, we can express the optimization in terms of $\{\lambda_i^{(1)}\}, \{\lambda_i^{(0)}\}, Q$:

% % \begin{equation}\label{eq:optimization_1}
% %     \begin{split}
% %          \min_{\{\lambda_i^{(1)}\}, \{\lambda_i^{(0)}\}, Q} & \sum_{i=1}^d \frac{\lambda_i^{(0)} + u}{\lambda_i^{(1)} + v} + \sum_{i=1}^d \frac{\lambda_i^{(1)} + v}{\lambda_i^{(0)} + u} \\
% %          & + \brck{Q(\bar{g}^{(1)} - \bar{g}^{(0)})}^{\top} \diag\paren{\ldots, \frac{1}{\lambda_i^{(0)} + u} + \frac{1}{\lambda_i^{(1)} + v}, \ldots} \\
% %          & Q(\bar{g}^{(1)} - \bar{g}^{(0)}) \\
% %     \end{split}
% % \end{equation}
% \begin{align*}
%     \min_{\{\lambda_i^{(1)}\}, \{\lambda_i^{(0)}\}, Q} & \sum_{i=1}^d \frac{\lambda_i^{(0)} + u}{\lambda_i^{(1)} + v} + \sum_{i=1}^d \frac{\lambda_i^{(1)} + v}{\lambda_i^{(0)} + u} \nonumber \\  +& \brck{Q(\bar{g}^{(1)} - \bar{g}^{(0)})}^{\top} \nonumber \\ & \diag\paren{\ldots, \frac{1}{\lambda_i^{(0)} + u} + \frac{1}{\lambda_i^{(1)} + v}, \ldots}  \nonumber \\  & Q(\bar{g}^{(1)} - \bar{g}^{(0)}) \\ 
%     \subjectto &
%     \\ &  p(\sum_{i=1}^d \lambda_i^{(1)}) + (1-p)(\sum_{i=1}^d \lambda_i^{(0)}) \le P \\ &
%     - \lambda_i^{(1)} \le 0, \; \forall i \in [d]\\ &
%     - \lambda_i^{(0)} \le 0, \; \forall i \in [d].\\ &
%     \lam{i}{1} \ge  \lam{j}{1}, \forall i < j. \\ &
%     \lam{i}{0} \ge  \lam{j}{0}, \forall i < j. \\ &
%     Q \; \textrm{orthogonal}.
% \end{align*}

% For any fixed feasible $\{\lambda_i^{(1)}\}, \{\lambda_i^{(0)}\}$, we see that the corresponding minimizing $Q$ will set its first row to be the unit vector in the direction of $\Delta g$. Thus by first minimizing $Q$, the optimization objective reduces to:
% \begin{align*}
%     &\sum_{i=1}^d \frac{\lambda_i^{(0)} + u}{\lambda_i^{(1)} + v} + \sum_{i=1}^d \frac{\lambda_i^{(1)} + v}{\lambda_1^{(0)} + u} +  \frac{g}{\lambda_1^{(0)} + u} + \frac{g}{\lambda_1^{(1)} + v} \nonumber \\
%     =& \sum_{i=2}^d \frac{\lambda_i^{(0)} + u}{\lambda_i^{(1)} + v} + \sum_{i=2}^d \frac{\lambda_i^{(1)} + v}{\lambda_i^{(0)} + u} + \frac{\lambda_1^{(1)} + v + \norm{\Delta g}_2^2}{\lambda_1^{(0)} + u} \nonumber \\ +& \frac{ \lambda_1^{(0)} + u + \norm{\Delta g}_2^2}{\lambda_1^{(1)} + v} \label{objective1}.
% \end{align*}
% We see that for the pair of variable $(\lam{i}{1}, \lam{i}{0})$ the function $\frac{\lambda_i^{(0)} + u}{\lambda_i^{(1)} + v} + \frac{\lambda_i^{(1)} + v}{\lambda_1^{(0)} + u}$ is strictly convex over the line segment $p\lam{i}{1} + (1-p)\lam{i}{0} =c $ for any positive $c$ and attains the the minimum value at $\lam{i}{1} = 0$ when $v < u$ and $\lam{i}{0} = 0$ when $v \ge u$. Suppose without loss of generality $u < v$, then for the optimal solution we must have 
% $\lam{i}{0}=0$ for all $i$. Under this condition, we notice that the function $x \mapsto \frac{u}{x+v} + \frac{x+v}{u}$ is strictly convex on the positive reals. Thus by Jensen inequality, the optimal solution's variables $\lam{i}{1}$ must take on the same value for all $i$. As a result, we have proved that at the optimal solution, we must have:
% \begin{align*}
%     \lambda_i^{(0)}=\lambda_j^{(0)} \textrm{ and } \lambda_i^{(1)}=\lambda_j^{(1)}, \textrm{ for } i, j \ge 2.
% \end{align*}

% Hence, we have the equivalent optimization problem as described in Theorem ~\ref{thm:optimal_solution}.
% % Hence, we have the equivalent optimization problem:
% % \begin{equation}\label{objective2}
% %     \begin{aligned}
% %     \min_{\lambda_1^{(0)}, \lambda_1^{(1)}, \lambda_2^{(0)}, \lambda_2^{(1)}}& \; (d-1) \frac{\lambda_2^{(0)} + u}{\lambda_2^{(1)} + v} + (d-1) \frac{\lambda_2^{(1)} + v}{\lambda_2^{(0)} + u} + \\ & \frac{\lambda_1^{(0)} + u + \norm{\Delta g}_2^2}{\lambda_1^{(1)} + v}  + \frac{ \lambda_1^{(1)} + v + \norm{\Delta g}_2^2}{\lambda_1^{(0)} + u} \\
% %     \subjectto &  \\
% %     & p \lambda_1^{(1)} + p(d-1) \lambda_2^{(1)}+ (1-p) \lambda_1^{(0)}+ (1-p)(d-1)(\lambda_2^{(0)}) \le \; P \\
% %     & \tenquad - \lambda_1^{(1)} \le \; 0  \\
% %     & \tenquad - \lambda_1^{(0)} \le \; 0  \\
% %     & \tenquad - \lambda_2^{(1)} \le \; 0  \\
% %     & \tenquad - \lambda_2^{(0)} \le \; 0  \\
% %     & \tenquad \lambda_2^{(1)} - \lambda_1^{(1)} \le \; 0 \\
% %     & \tenquad \lambda_2^{(0)} - \lambda_1^{(0)} \le \; 0 .
% % \end{aligned}
% % \end{equation}

% Given the optimal solution to the above 4-variable problem $(\Lam{1}{0}, \Lam{2}{0}, \Lam{1}{1}, \Lam{2}{1})$, we can set $Q$ to be any orthogonal matrix whose first row is the vector $\frac{\Delta g}{\norm{\Delta g}_2}$. Plugging this back into the expression of $\Sigma_1$ and $\Sigma_0$ gives us the final result.

% % Thus the proof is complete.
% % \bigskip

% \remark{} By analyzing the KKT condition of this four variable problem we can find that the optimal solution must occur on the hyperplane $p \lambda_1^{(1)} + p(d-1) \lambda_2^{(1)}+ (1-p) \lambda_1^{(0)}+ (1-p)(d-1)(\lambda_2^{(0)}) = P$. Knowing from the proof above that in addition $\lam{2}{1} = 0$ if $u \ge v$ and $\lam{2}{0} = 0$ if $u < v$ further reduces this problem to a 3-variable problem. Keeping one of them fixed and optimizing the other two reduces the problem to a line search over a convex objective. Alternatively fixing one of these three variables while optimizing the other two would eventually converge and give us the optimal solution.
